# Supplementary material for: EPIC-Bench: A Perception-Centric Benchmark for Fine-Grained Embodied Visual Grounding in Vision-Language Models
Source: arXiv:2605.17070 source file (2026-10-15)
Supplement: Supplementary file 1 [file appendix_emnlp.tex]

\appendix
\clearpage
% In the supplementary material, Appendix.~\ref{app:examples} presents benchmark examples, Appendix.~\ref{app:data_sources} details the data sources, Appendix.~\ref{app:prompts} provides the prompt templates for each sub-task, Appendix.~\ref{app:path_score} describes the path score definition, and Appendix~\ref{app:additional_results} reports the additional evaluation results on EPIC-Bench.


\section{Appendix Outline}

In these supplementary materials, we provide:
\begin{itemize}[noitemsep, topsep=0pt, leftmargin=*]
    \item Additional discussion on vision-language grounding in embodied applications (Appendix~B);
    \item Benchmark examples, data sources, and quality-control details (Appendix~C);
    \item Evaluation prompts, prompt robustness experiments, post-processing analysis, and Path Score details (Appendix~D);
    \item Full evaluation results for all tested models (Appendix~E).
\end{itemize}



\section{Vision-Language Grounding for Embodied Application}



Vision-language grounding (VLG) has become an increasingly important capability for embodied intelligence. Rather than directly mapping observations and instructions into actions, many recent systems explicitly or implicitly rely on grounding intermediate representations that connect language instructions to executable physical targets.

A representative direction adopts modular perception–action decomposition, where grounding and control are handled separately. In these frameworks, VLMs first localize instruction-relevant targets and downstream robot policies then generate actions based on grounded observations. For example, [MOO, Manipulate Anything] use VLMs to predict target locations from language instructions before planning or grasp generation. [DexGraspVLA] converts instructions into object-level grasp specifications and conditions a DiT-based action policy on localized object representations. Similarly, [OWG, MOKA, ReKep] assume access to target masks and perform grasp keypoint estimation or manipulation planning based on localized targets. [GraspVLA] explicitly models grounding as an intermediate stage of action generation, whereas [RoboGround] directly predicts target and placement masks and uses them as conditions for downstream VLA execution.

The effectiveness of these modular systems suggests that accurate grounding can improve generalization by disentangling semantic interpretation from physical control. Under this design, VLMs handle instruction-to-scene alignment in novel environments, while robot policies concentrate on understanding spatial outputs and executing interactions with unseen object geometries.

Recent end-to-end VLA studies further support this observation by incorporating mechanisms that strengthen grounding-aware representations during training. For example, [DexGraspVLA] extracts target-mask features as action conditions to reduce background interference and encourage object-centric representations. [ReconVLA] introduces an auxiliary reconstruction objective that reconstructs instruction-related target regions, thereby improving grounding quality and fine-grained perception for manipulation.

Collectively, these works indicate that visual-language grounding is not merely an auxiliary perception capability but an increasingly important factor affecting embodied generalization and manipulation performance.











\section{Benchmark Construction Details}




\subsection{Benchmark Examples}
\label{app:examples}
In this section, we present detailed examples from EPIC-Bench to illustrate the input–output content required by tasks across different categories. For certain tasks, we also provide optional auxiliary annotations. These additional labels enable more accurate evaluation by accounting for the specific characteristics of different tasks and data types.

\paragraph{Target Localization} Figure~\ref{fig:example_TL_BA}, \ref{fig:example_TL_SRA} and \ref{fig:example_TL_ECA} present examples from the Target Localization category, including the three task types of Basic Attributes, Spatial-Related Attributes, and Embodied Compositional Attributes.

\paragraph{Navigation} Figure \ref{fig:example_NAV} illustrates the Navigation category, which includes the tasks of Ground Detection, Feasible Path Recognition, and Visual Matching.

\paragraph{Manipulation} Figure \ref{fig:example_MAN_AR} and \ref{fig:example_MAN_CR_PR} present examples from the Manipulation category, covering the tasks of Affordance Region, Contact Relationship, and Placement Region.




% \clearpage
\begin{figure*}[t]
\centering
\includegraphics[width=0.48\textwidth]{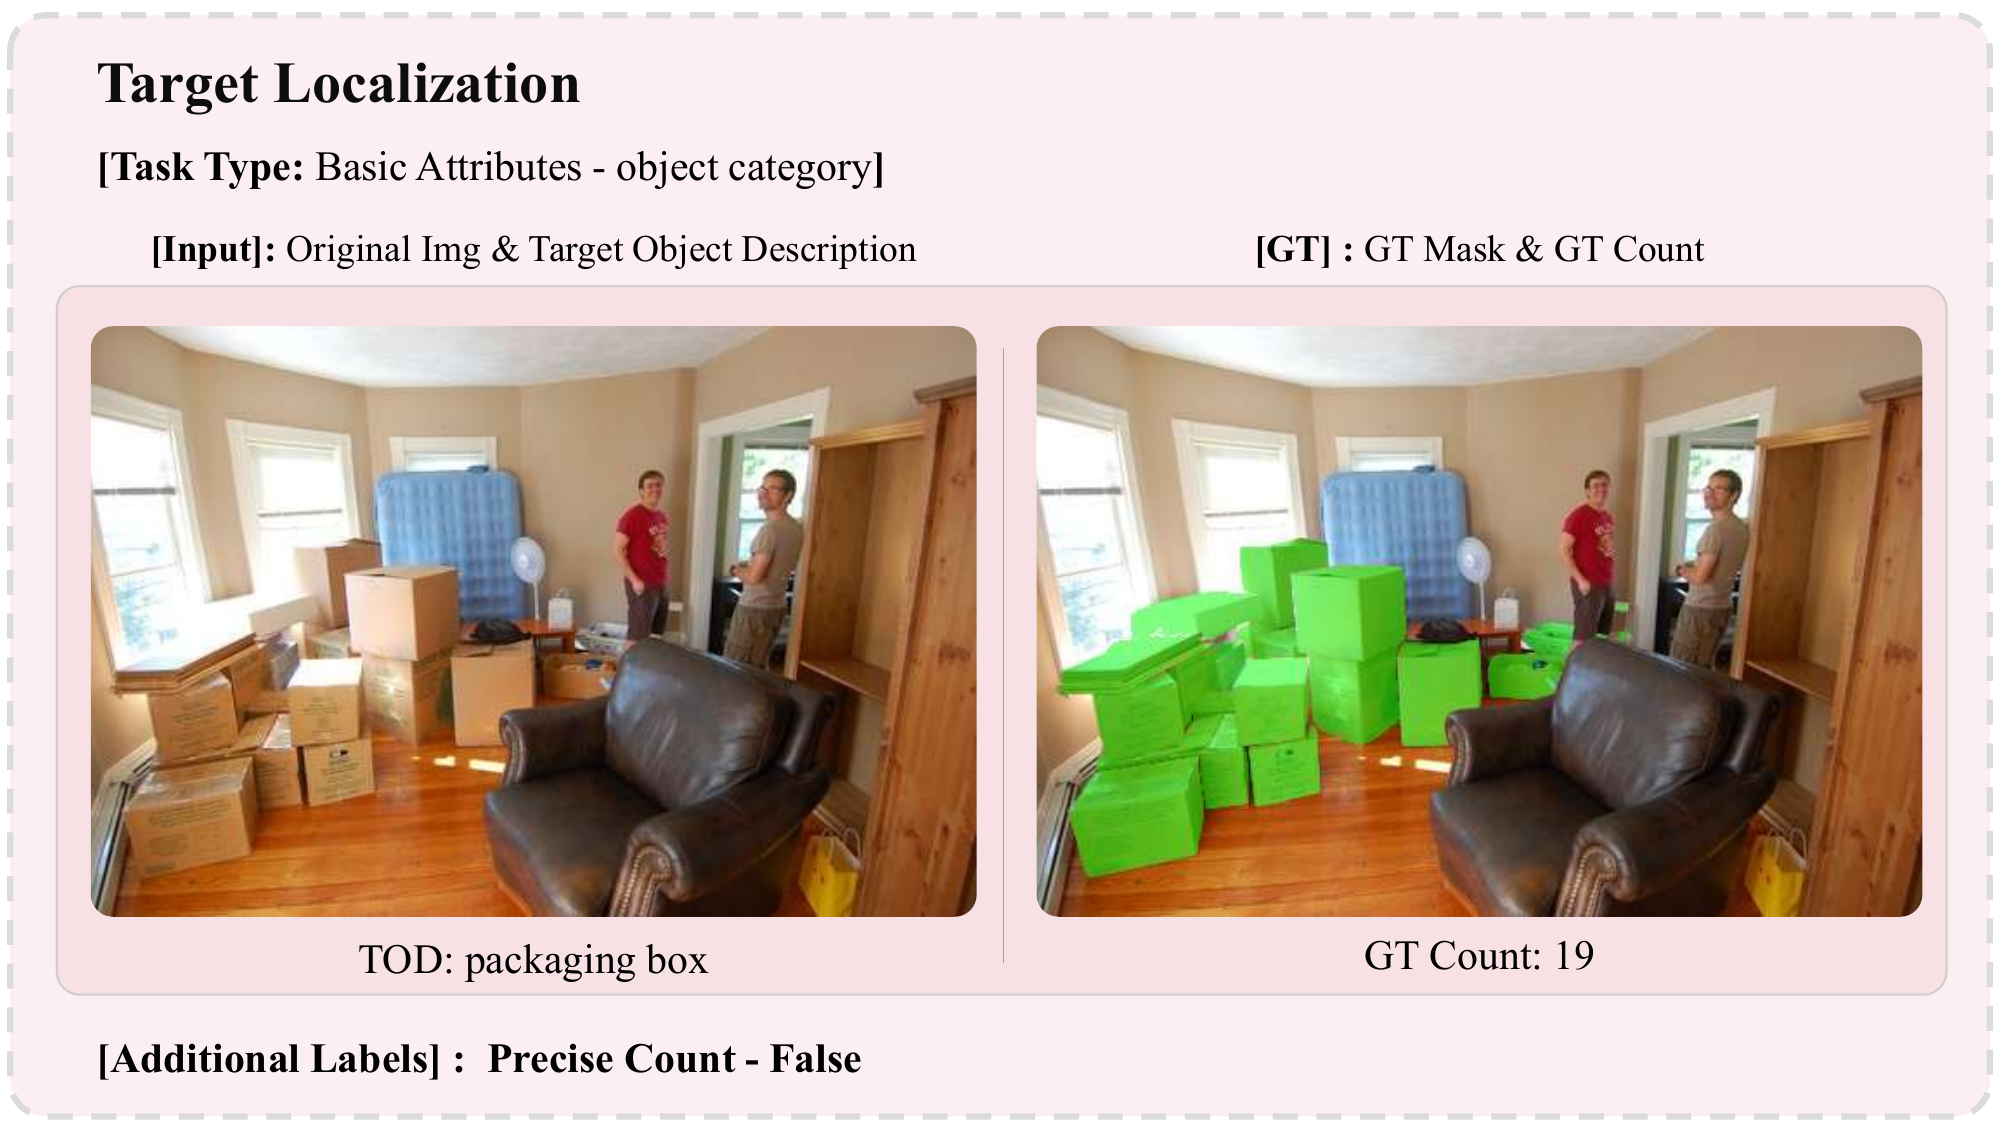}
\includegraphics[width=0.48\textwidth]{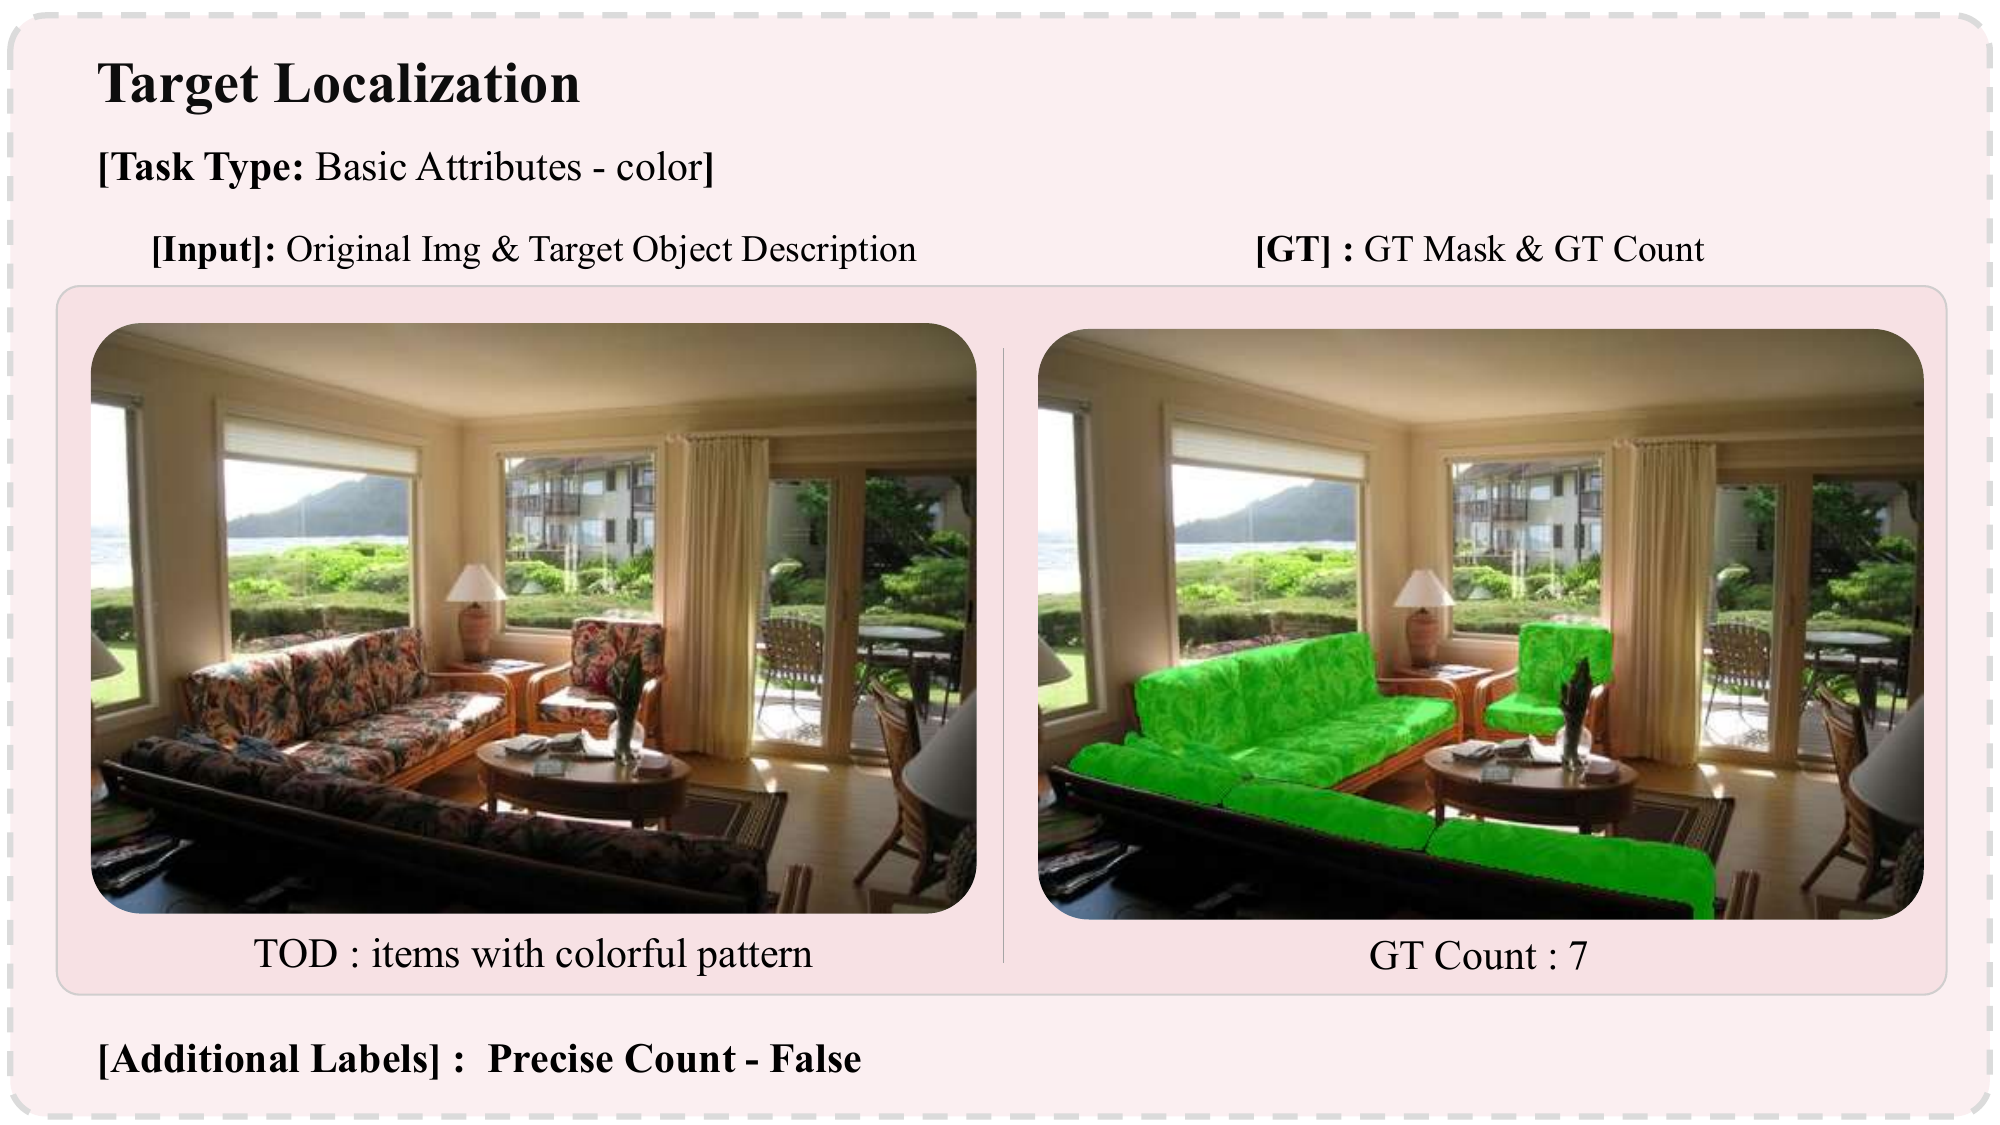}

\includegraphics[width=0.48\textwidth]{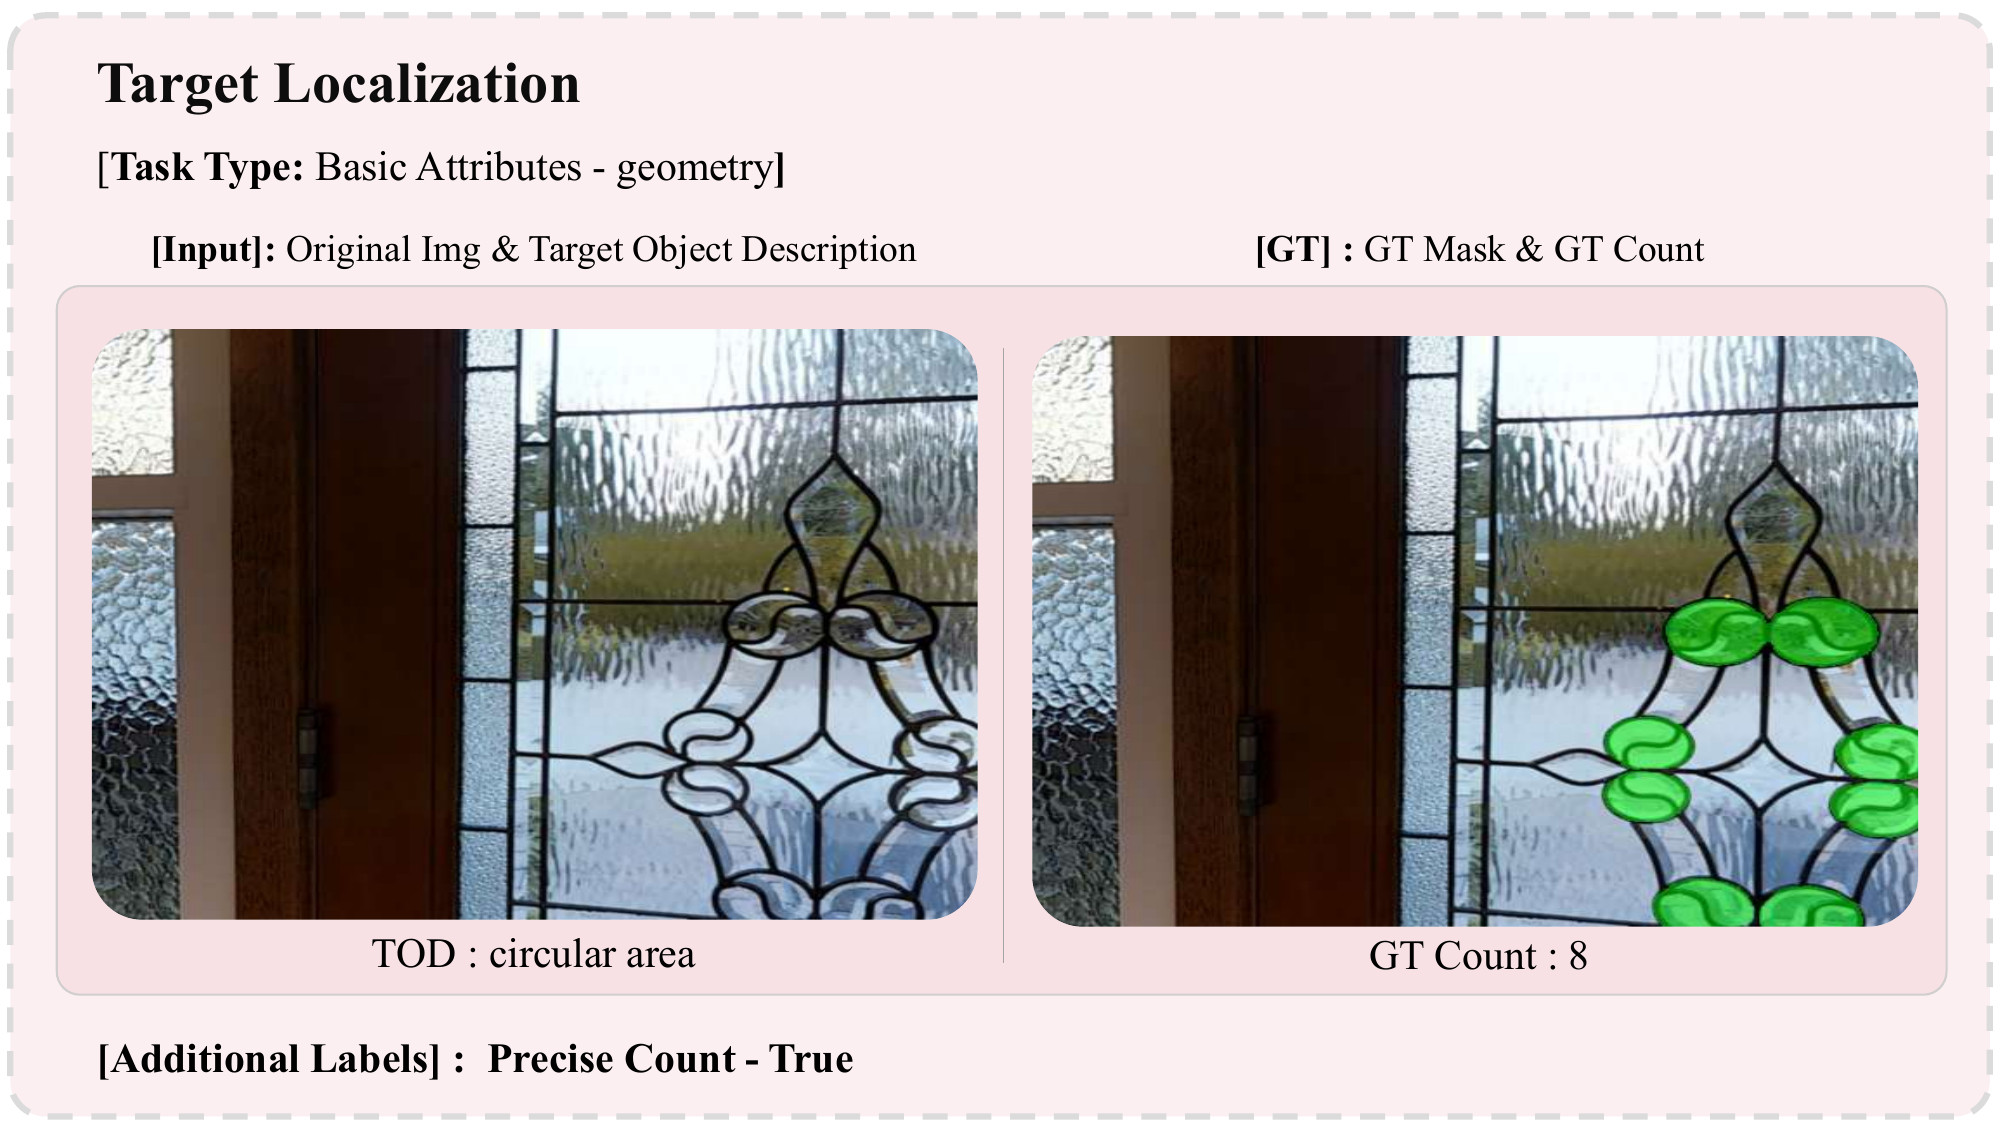}
\includegraphics[width=0.48\textwidth]{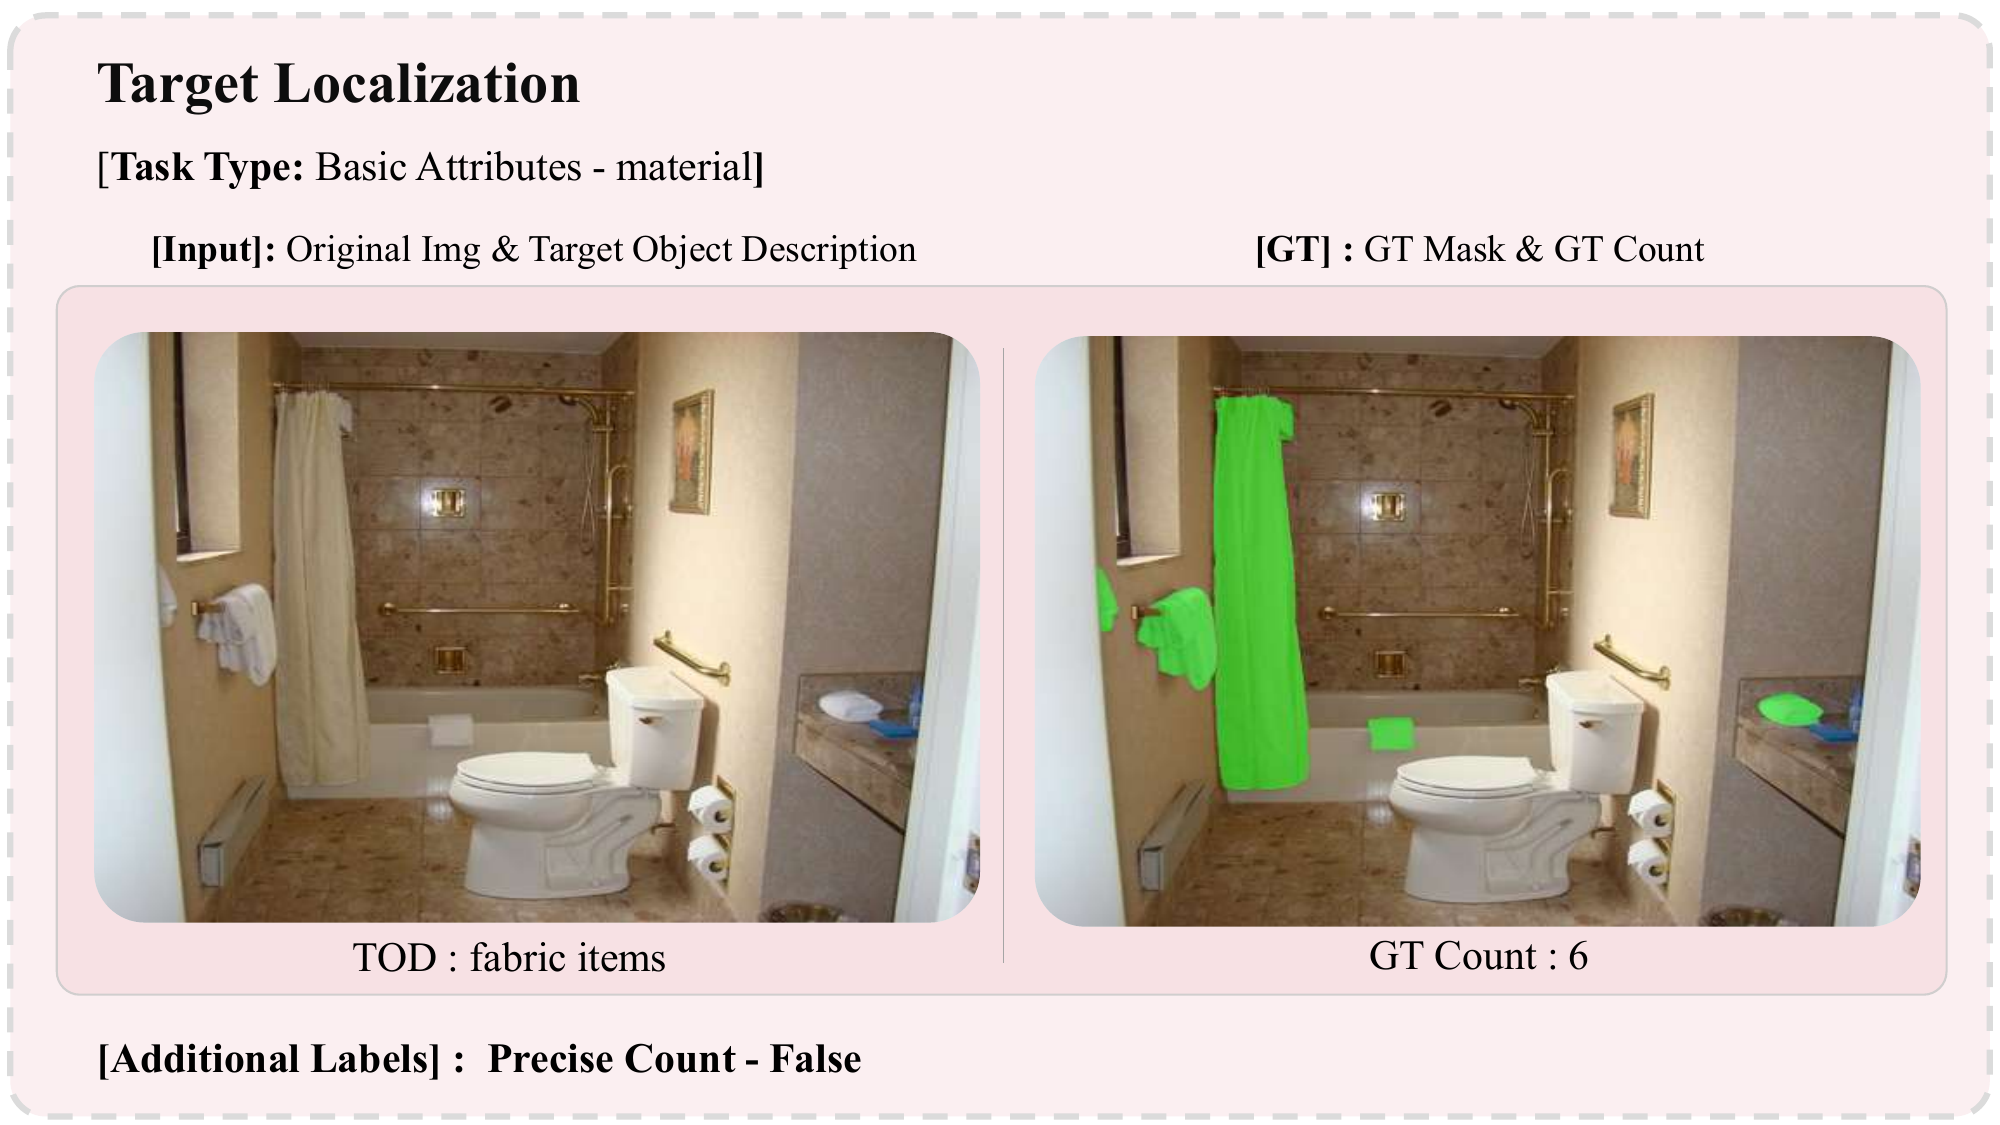}

\includegraphics[width=0.48\textwidth]{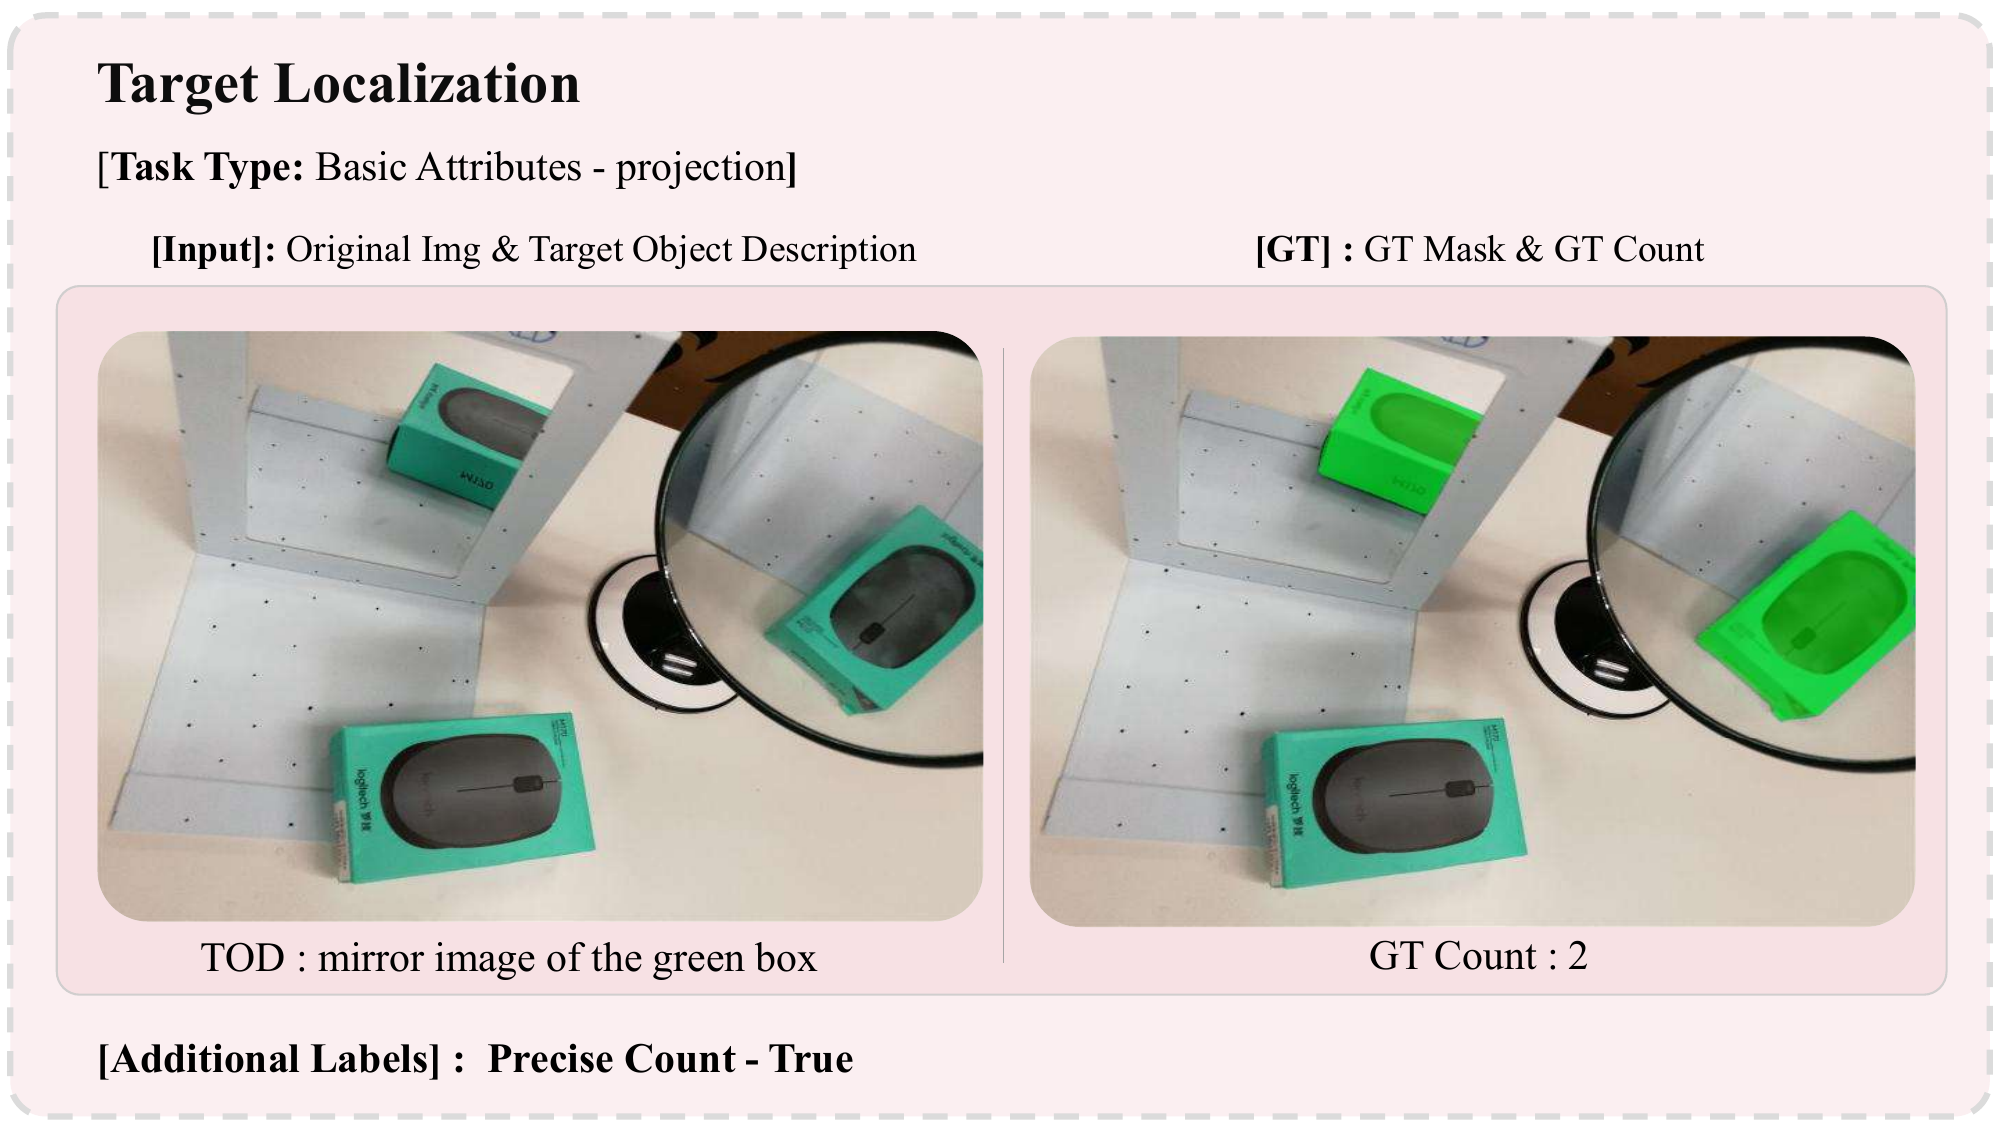}
\includegraphics[width=0.48\textwidth]{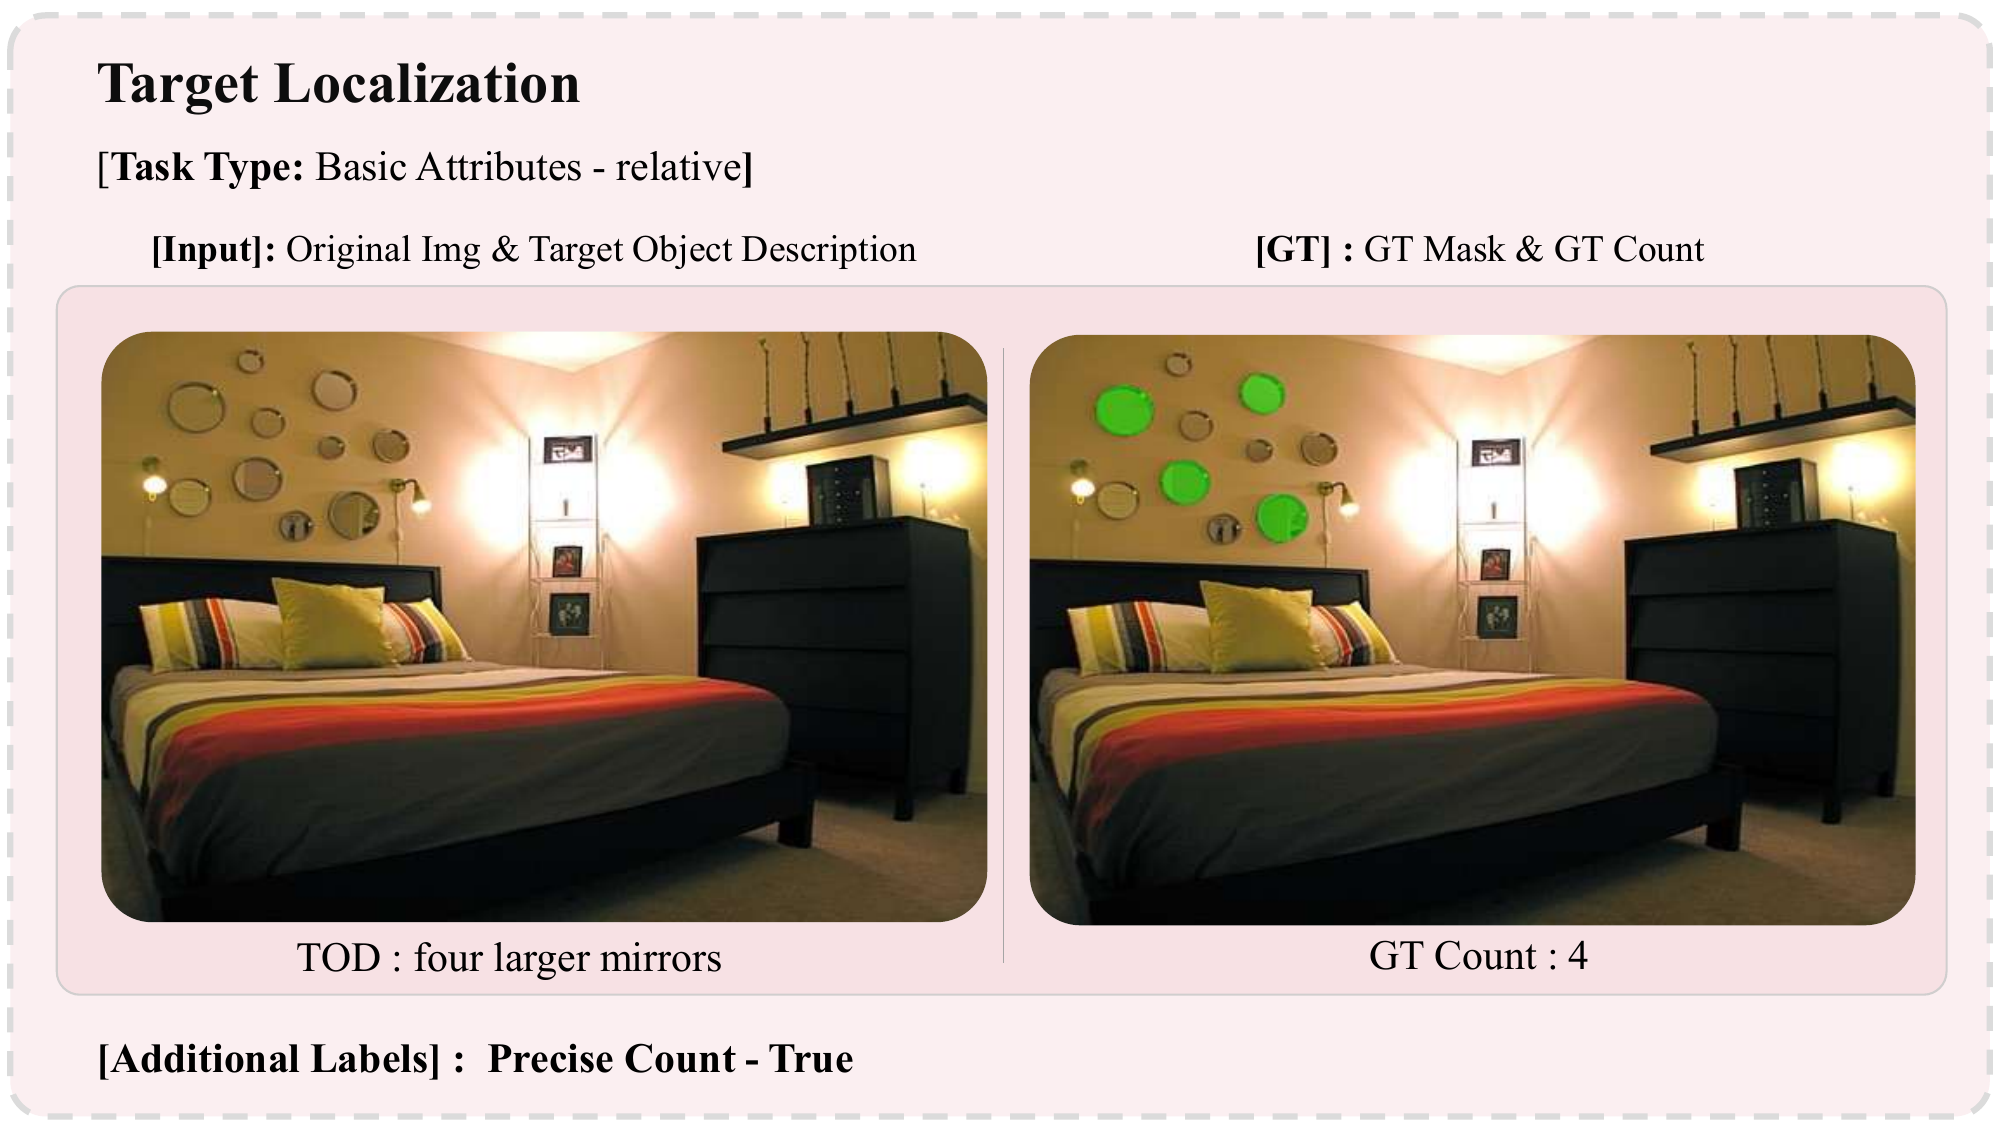}

\caption{Examples of Target Localization - Basic Attributes task.}
\label{fig:example_TL_BA}
\end{figure*}


% \clearpage
\begin{figure*}[t]
\centering
\includegraphics[width=0.48\textwidth]{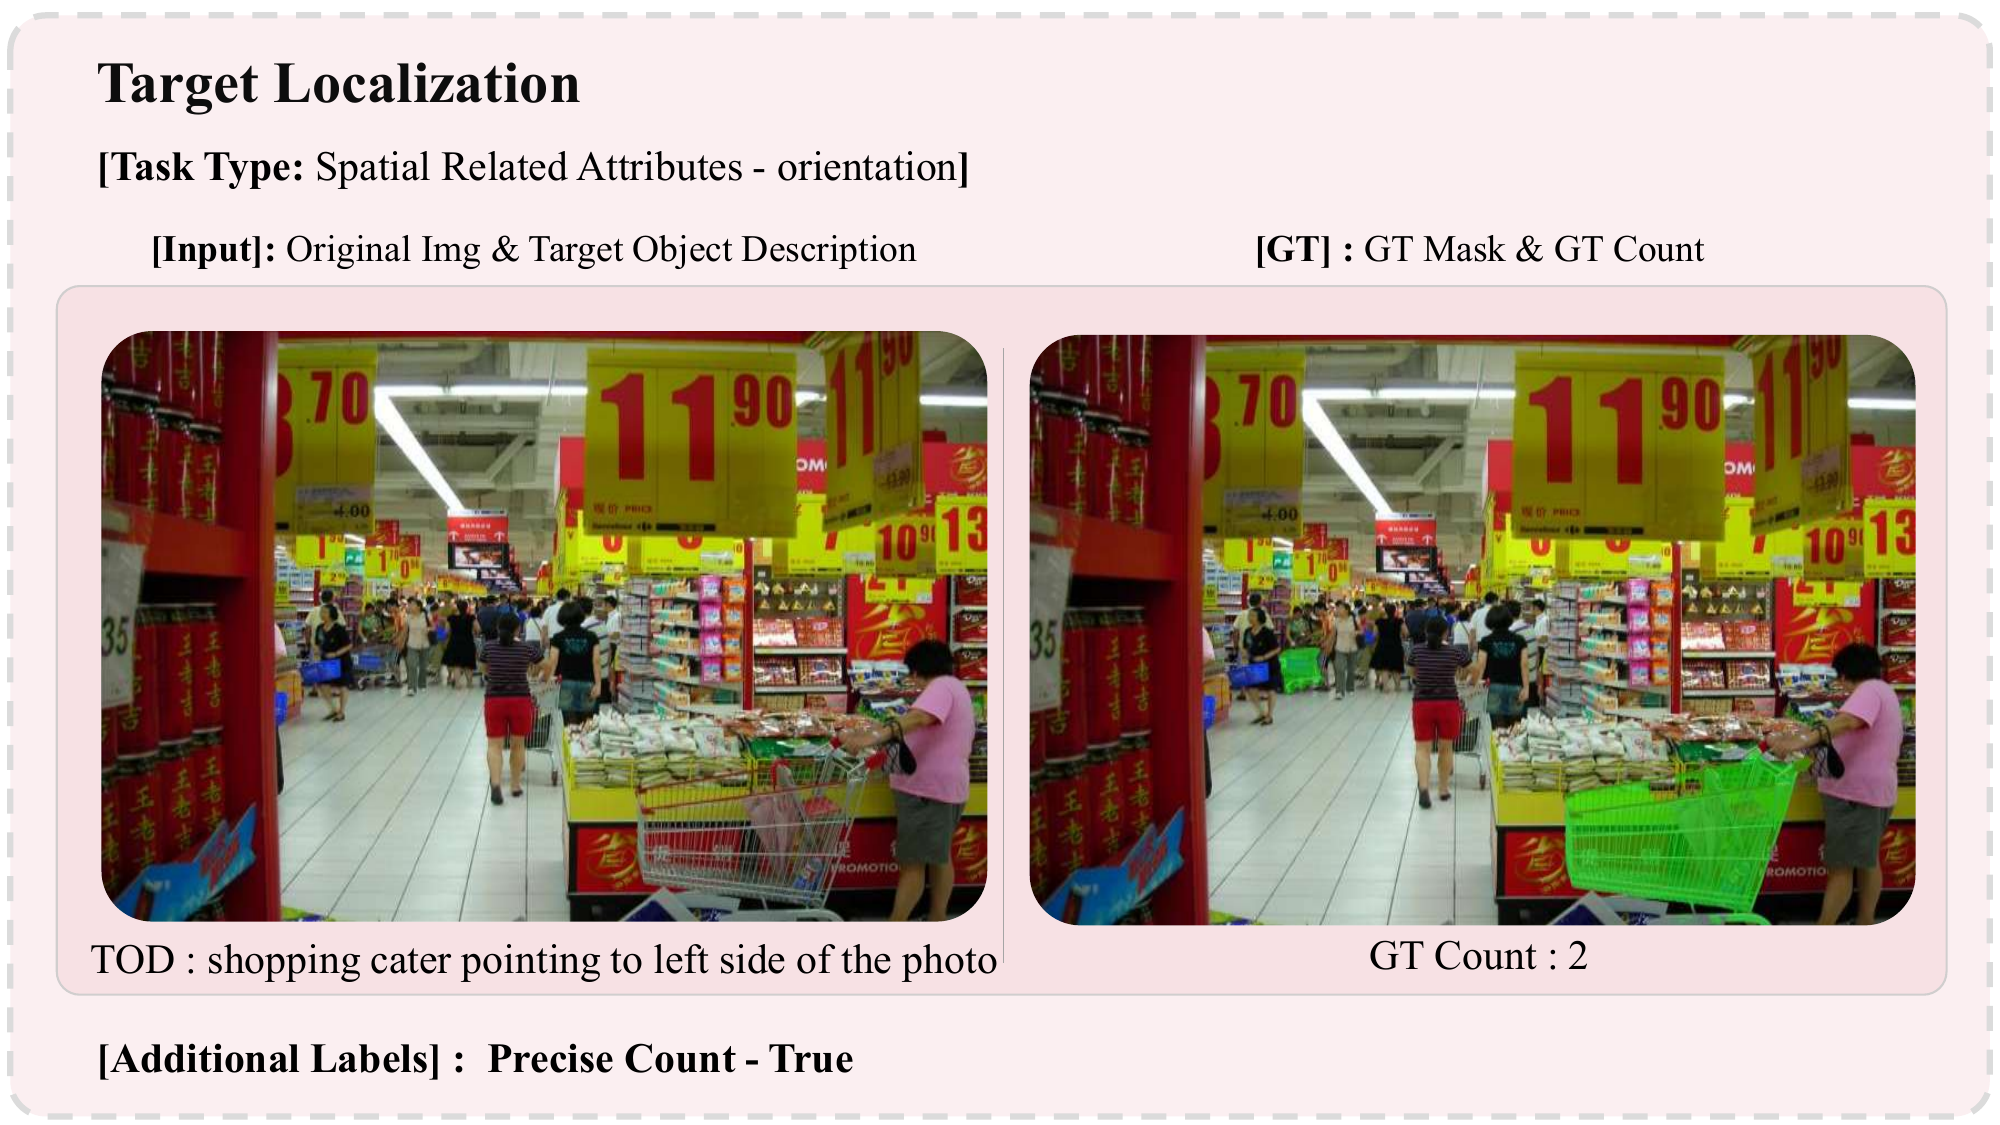}
\includegraphics[width=0.48\textwidth]{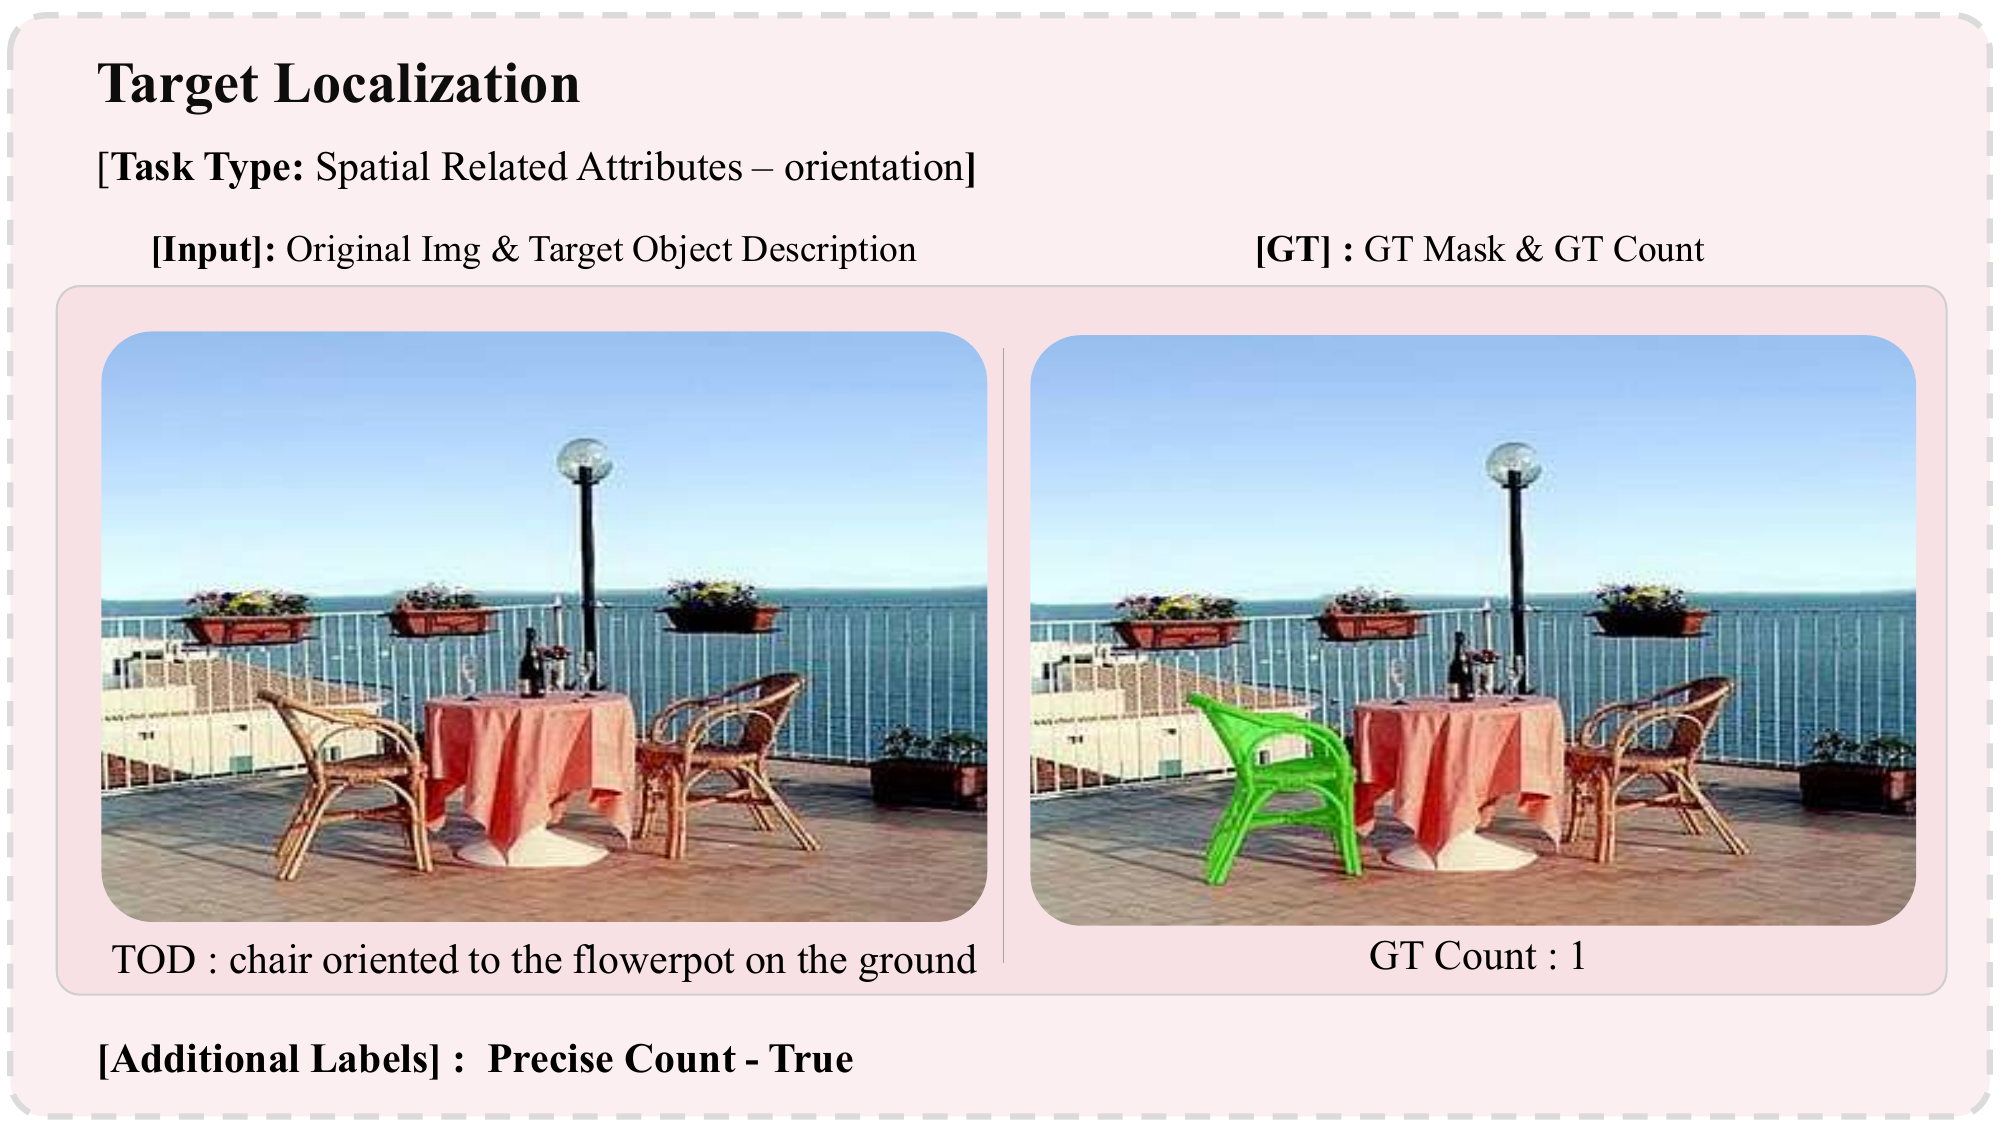}

\includegraphics[width=0.48\textwidth]{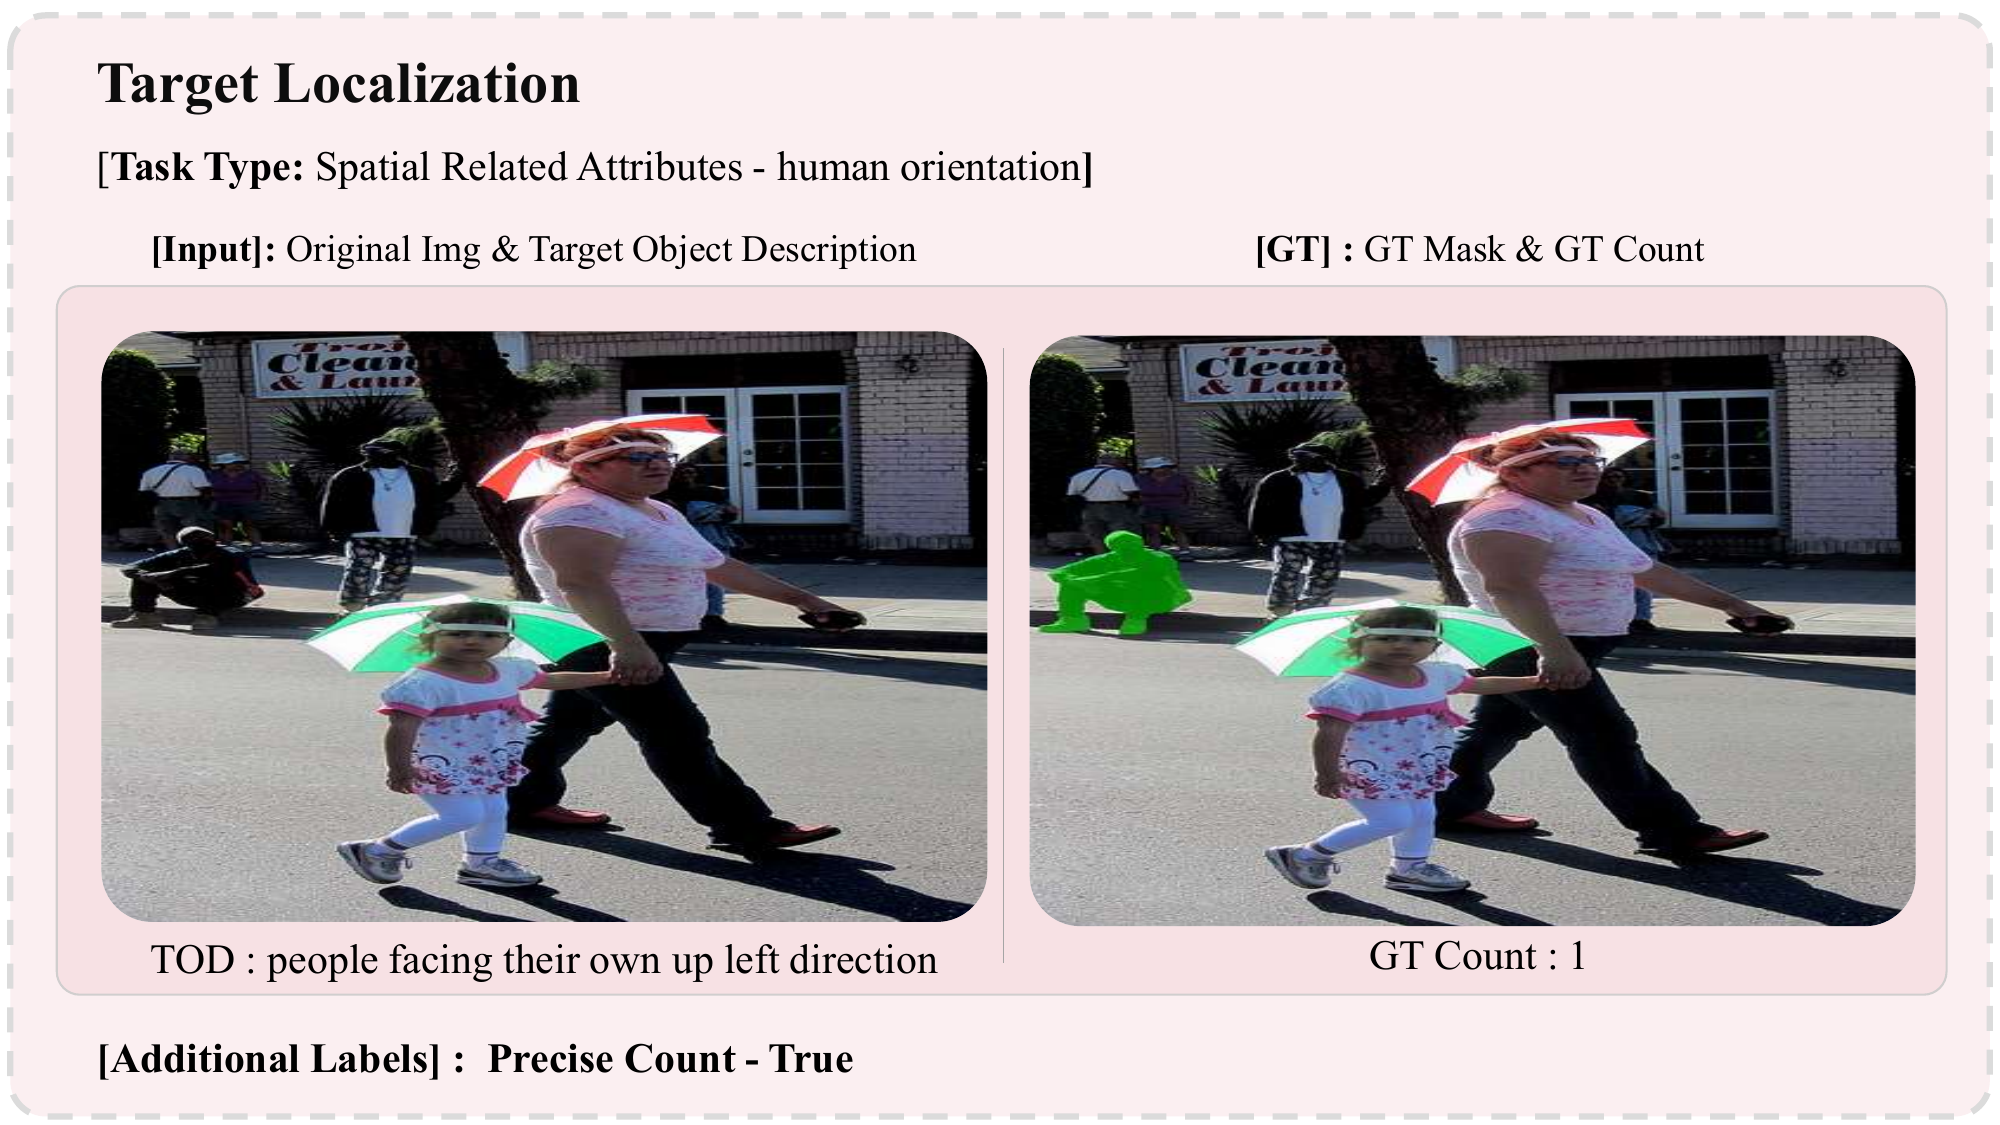}
\includegraphics[width=0.48\textwidth]{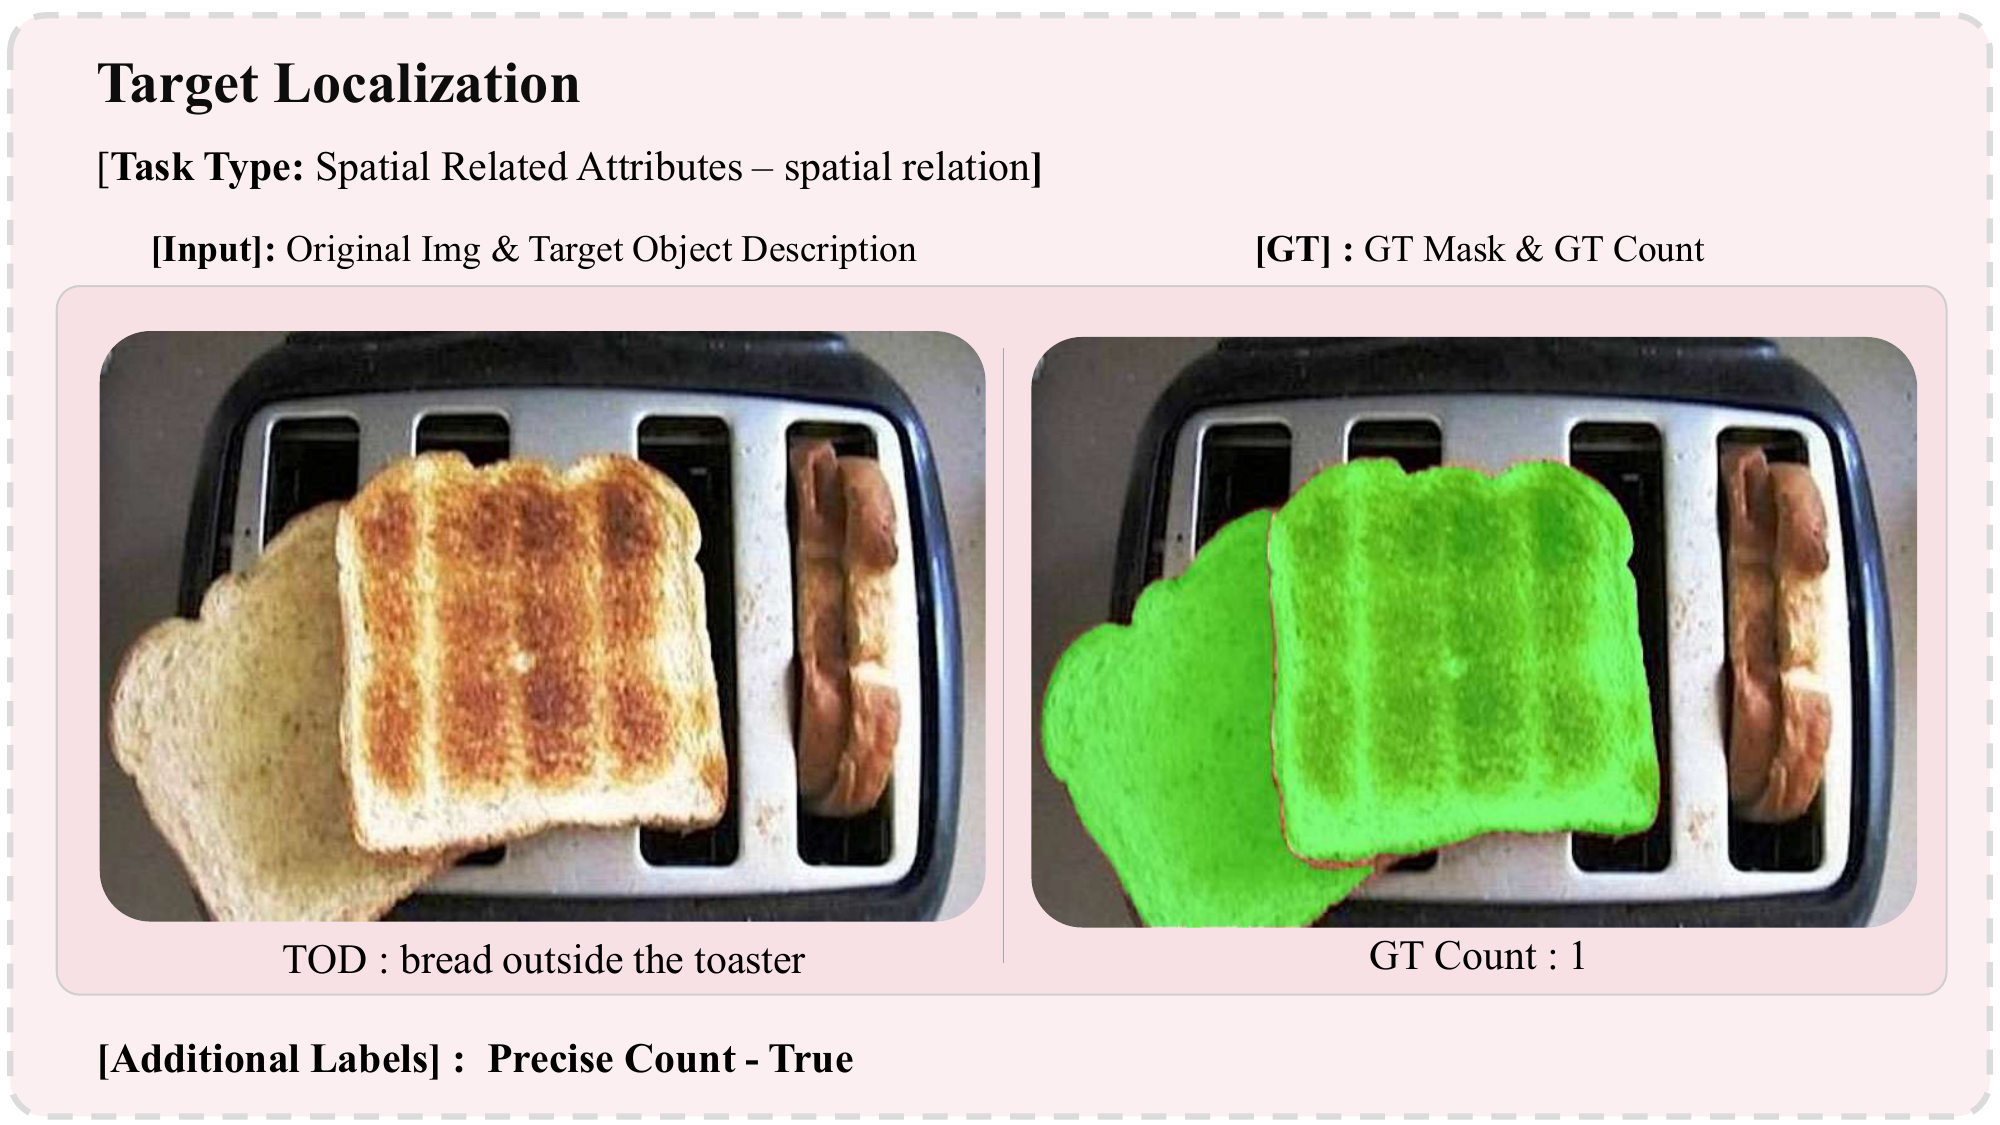}

\includegraphics[width=0.48\textwidth]{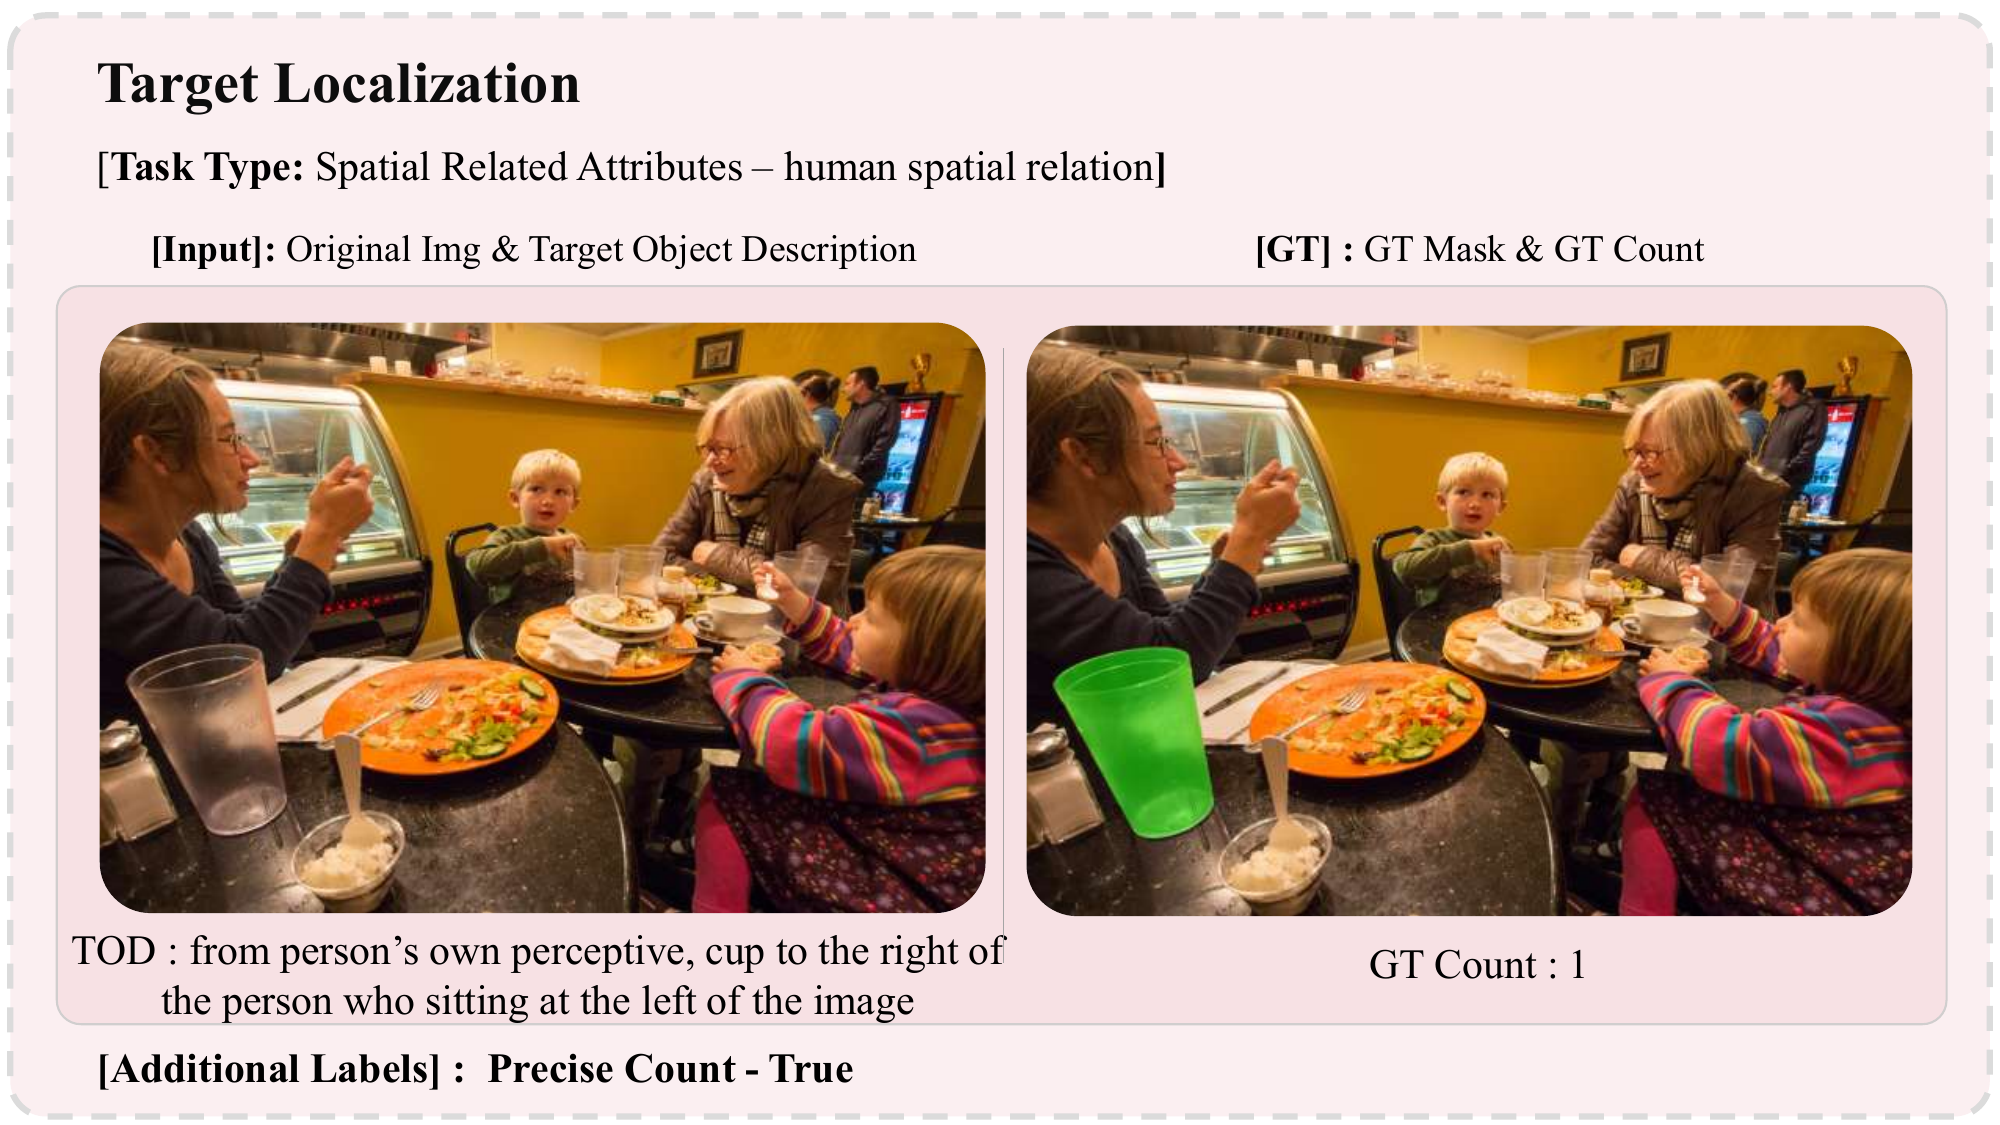}
\includegraphics[width=0.48\textwidth]{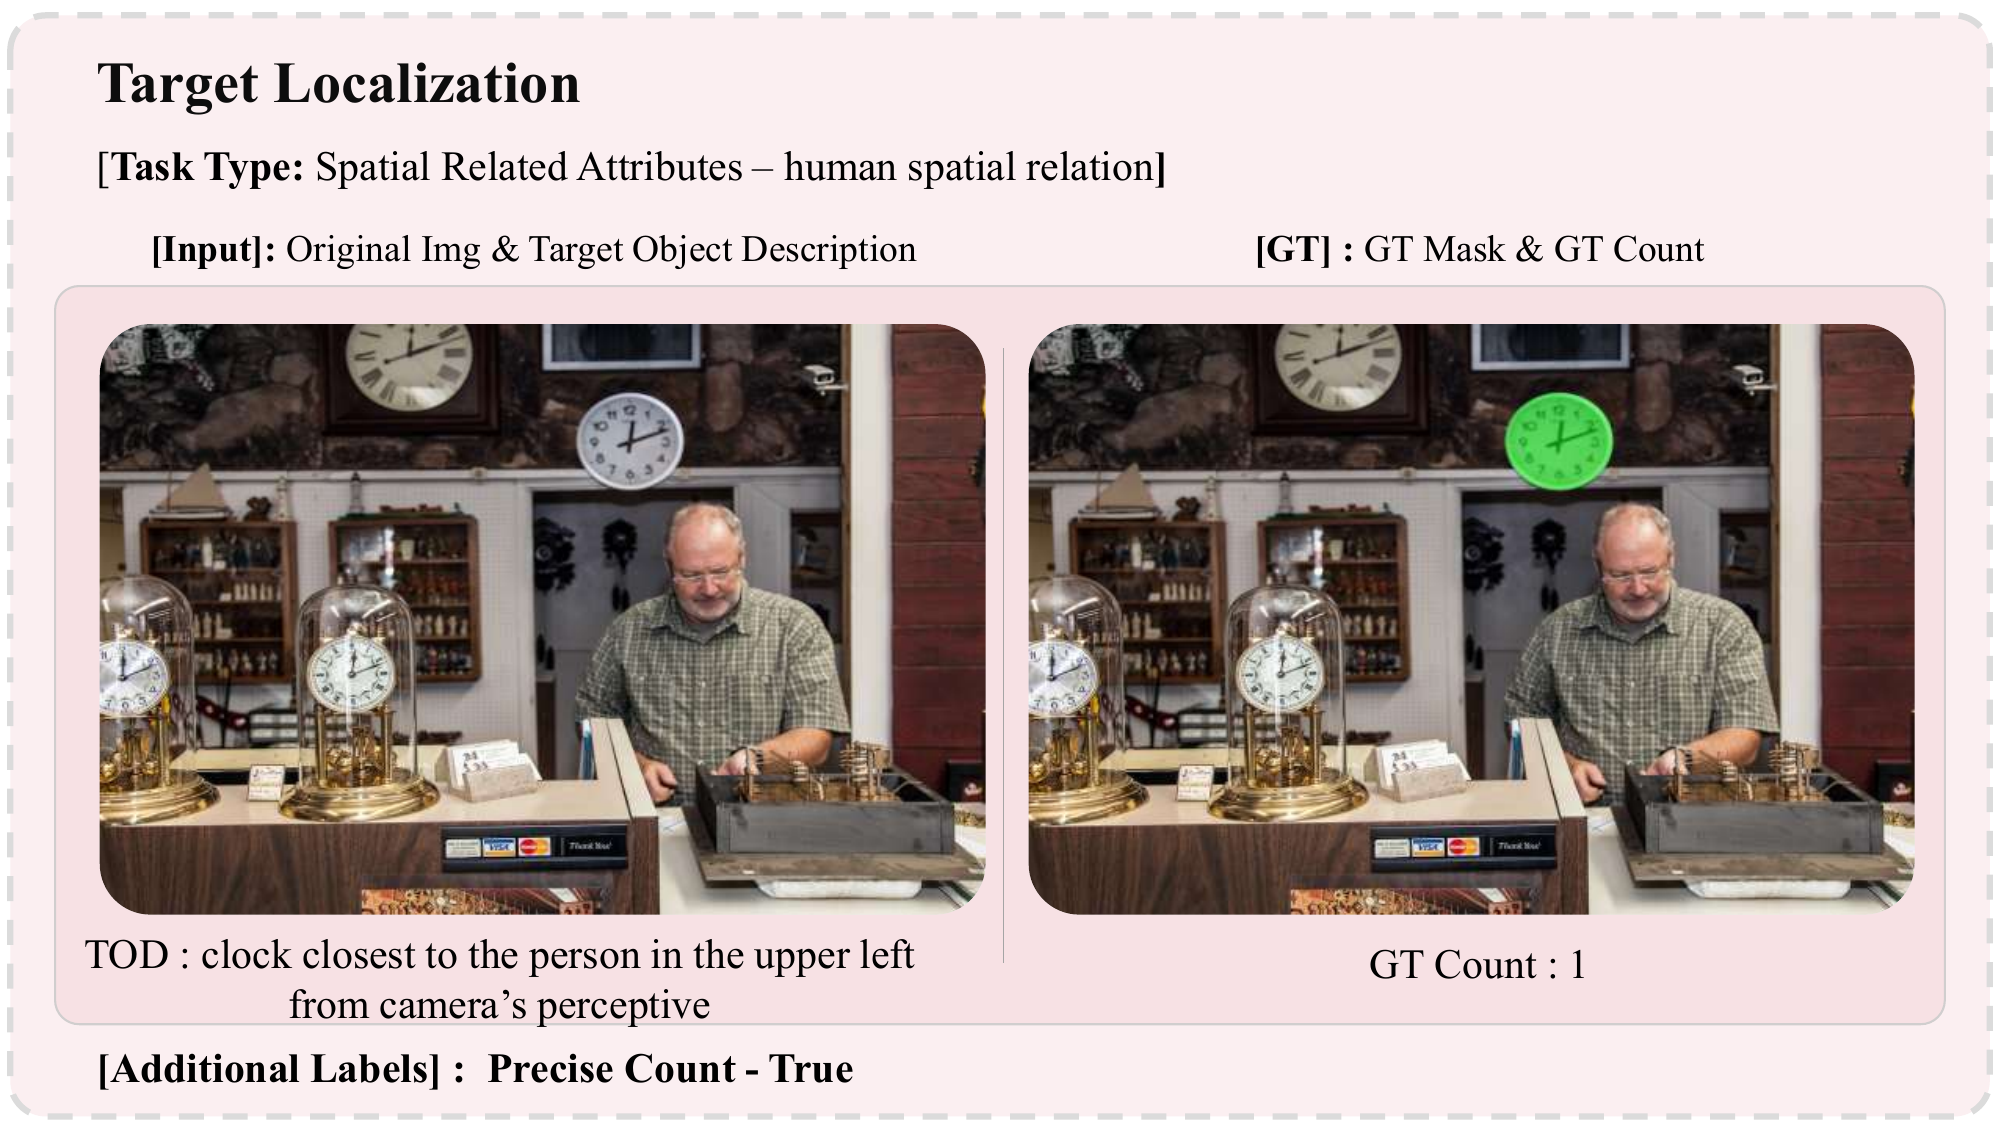}

\caption{Examples of Target Localization - Spatial Related Attributes task}
\label{fig:example_TL_SRA}
\end{figure*}




% \clearpage
\begin{figure*}[t]
\centering
\includegraphics[width=0.48\textwidth]{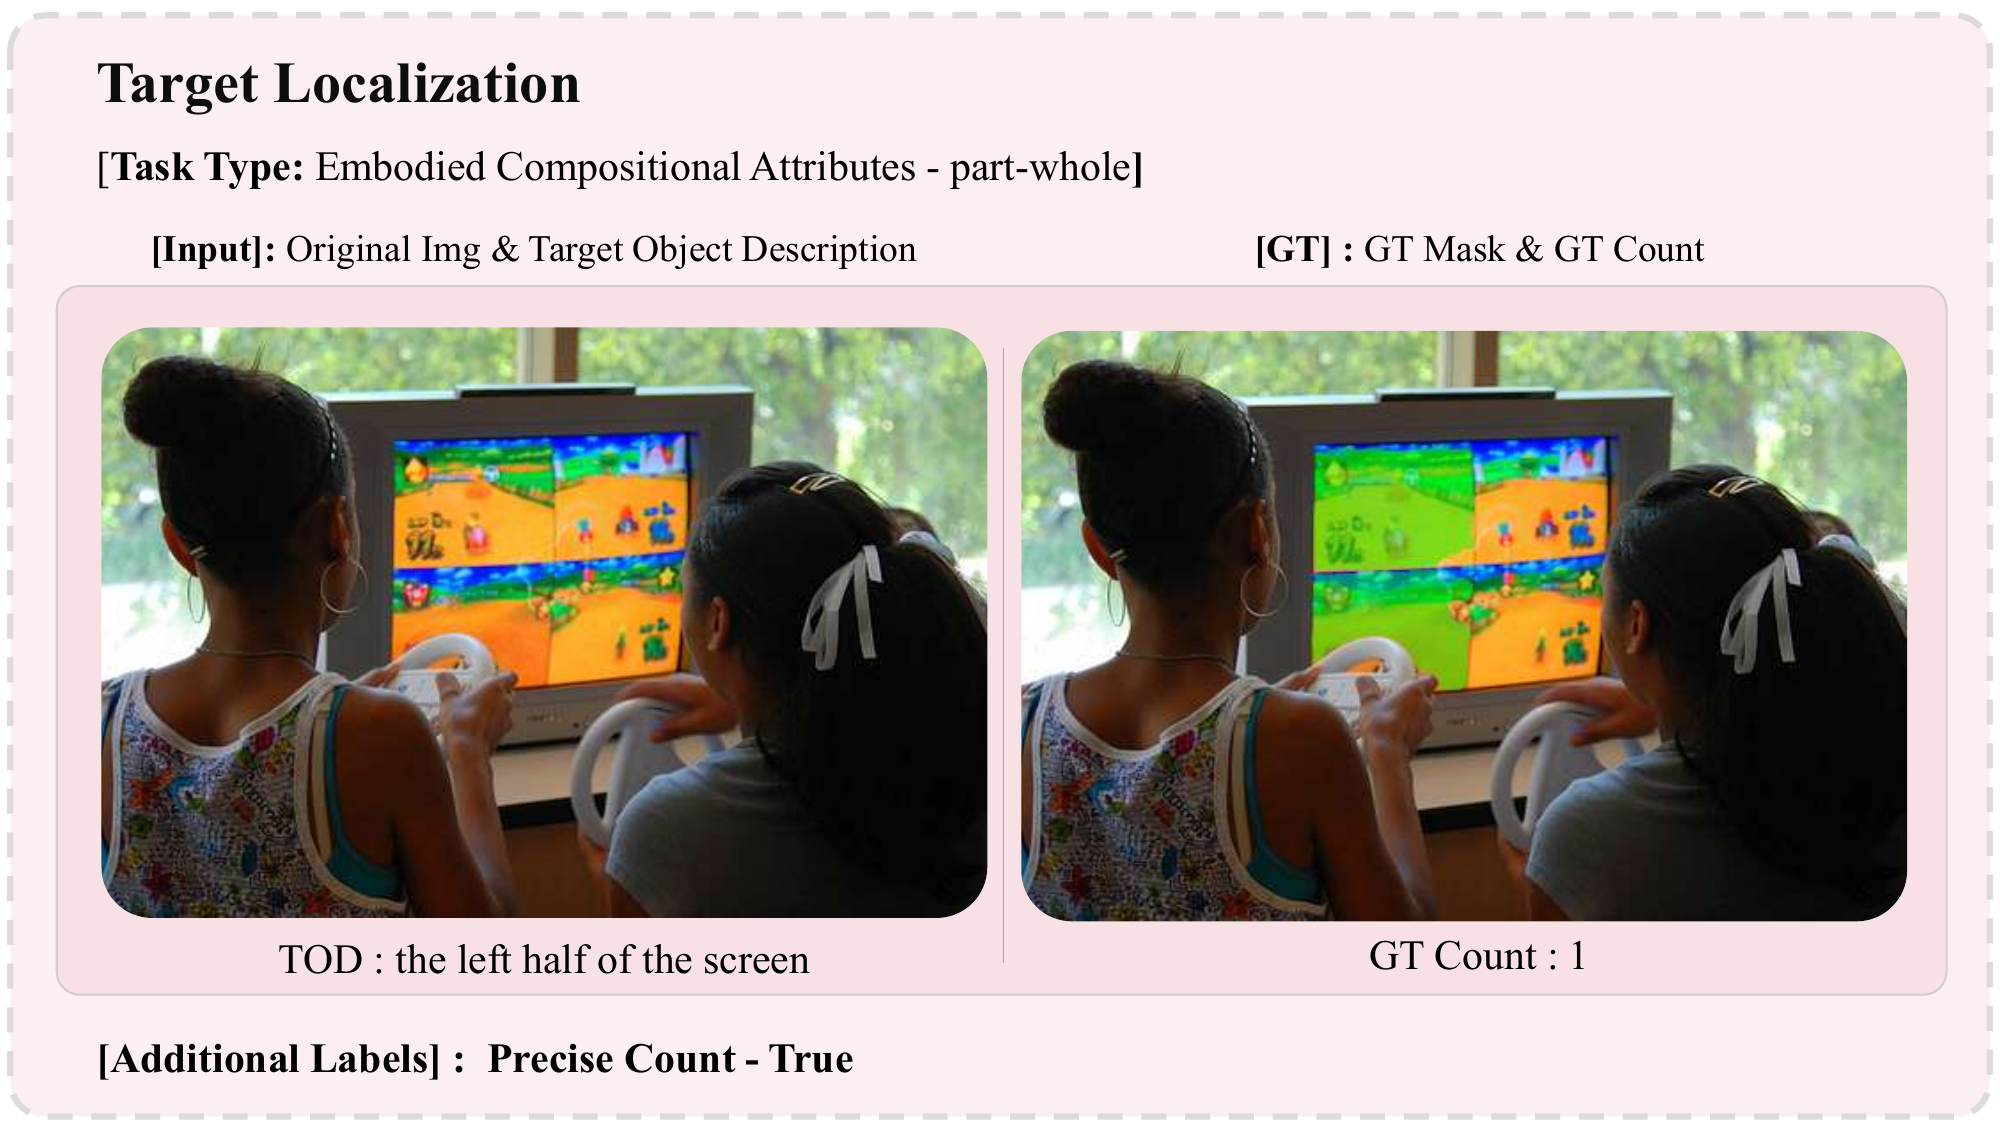}
\includegraphics[width=0.48\textwidth]{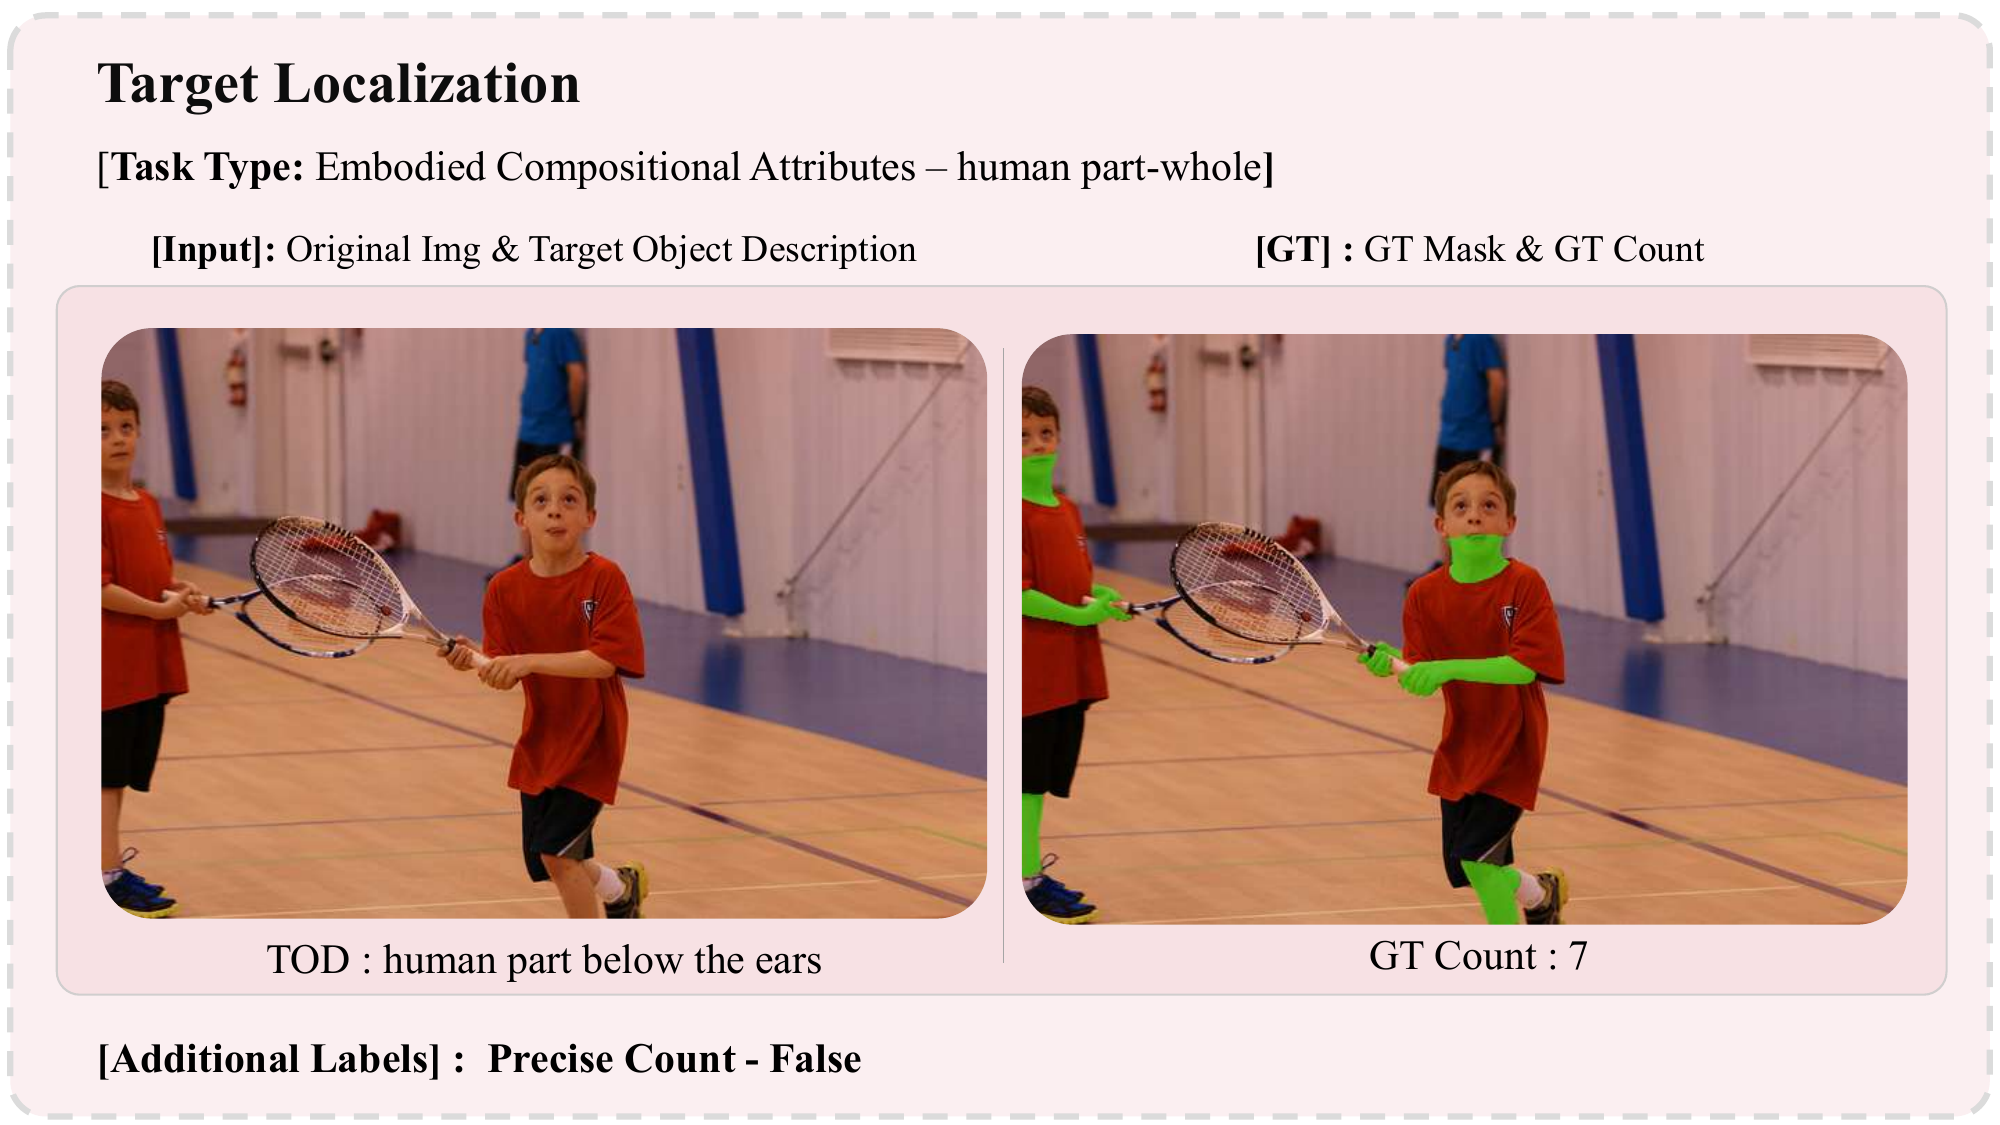}
\includegraphics[width=0.48\textwidth]{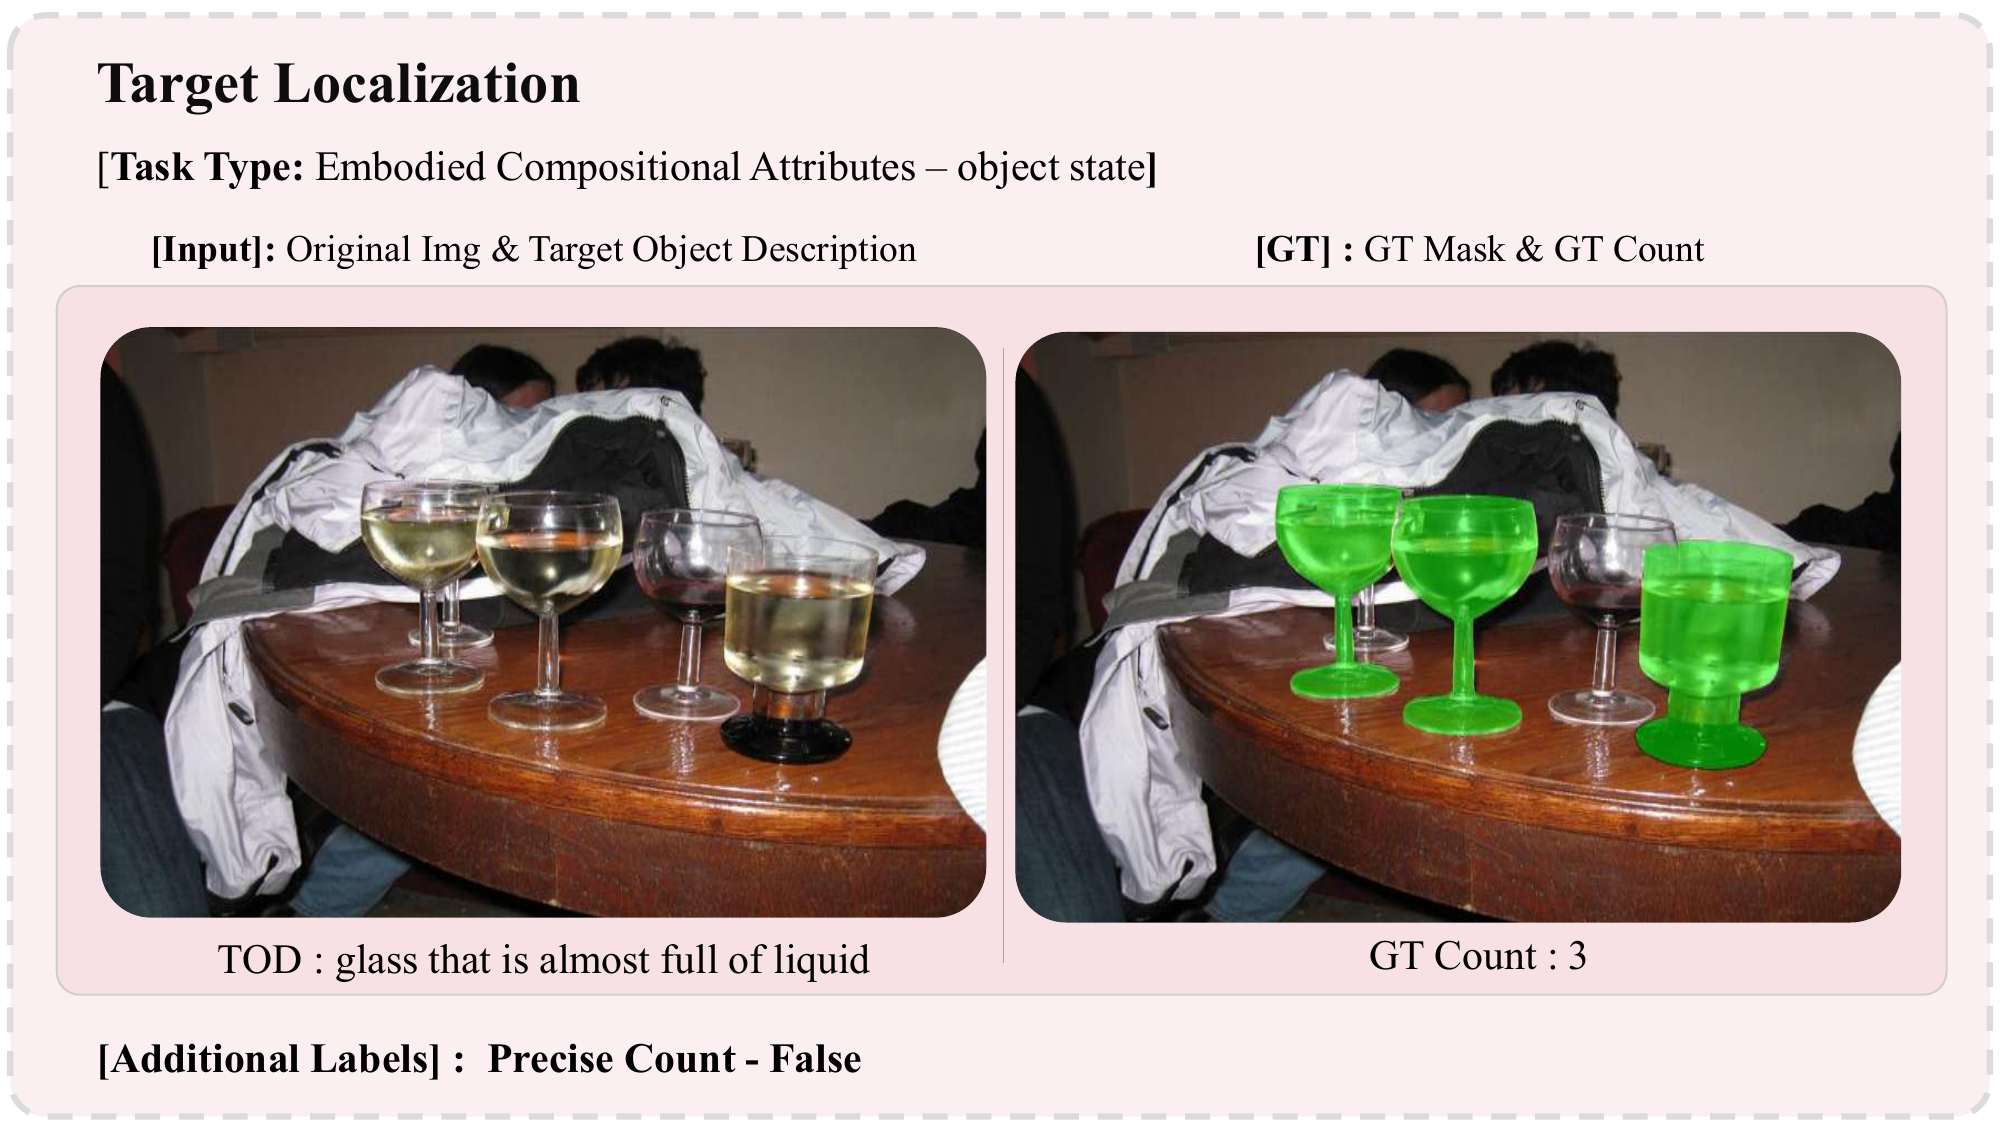}
\includegraphics[width=0.48\textwidth]{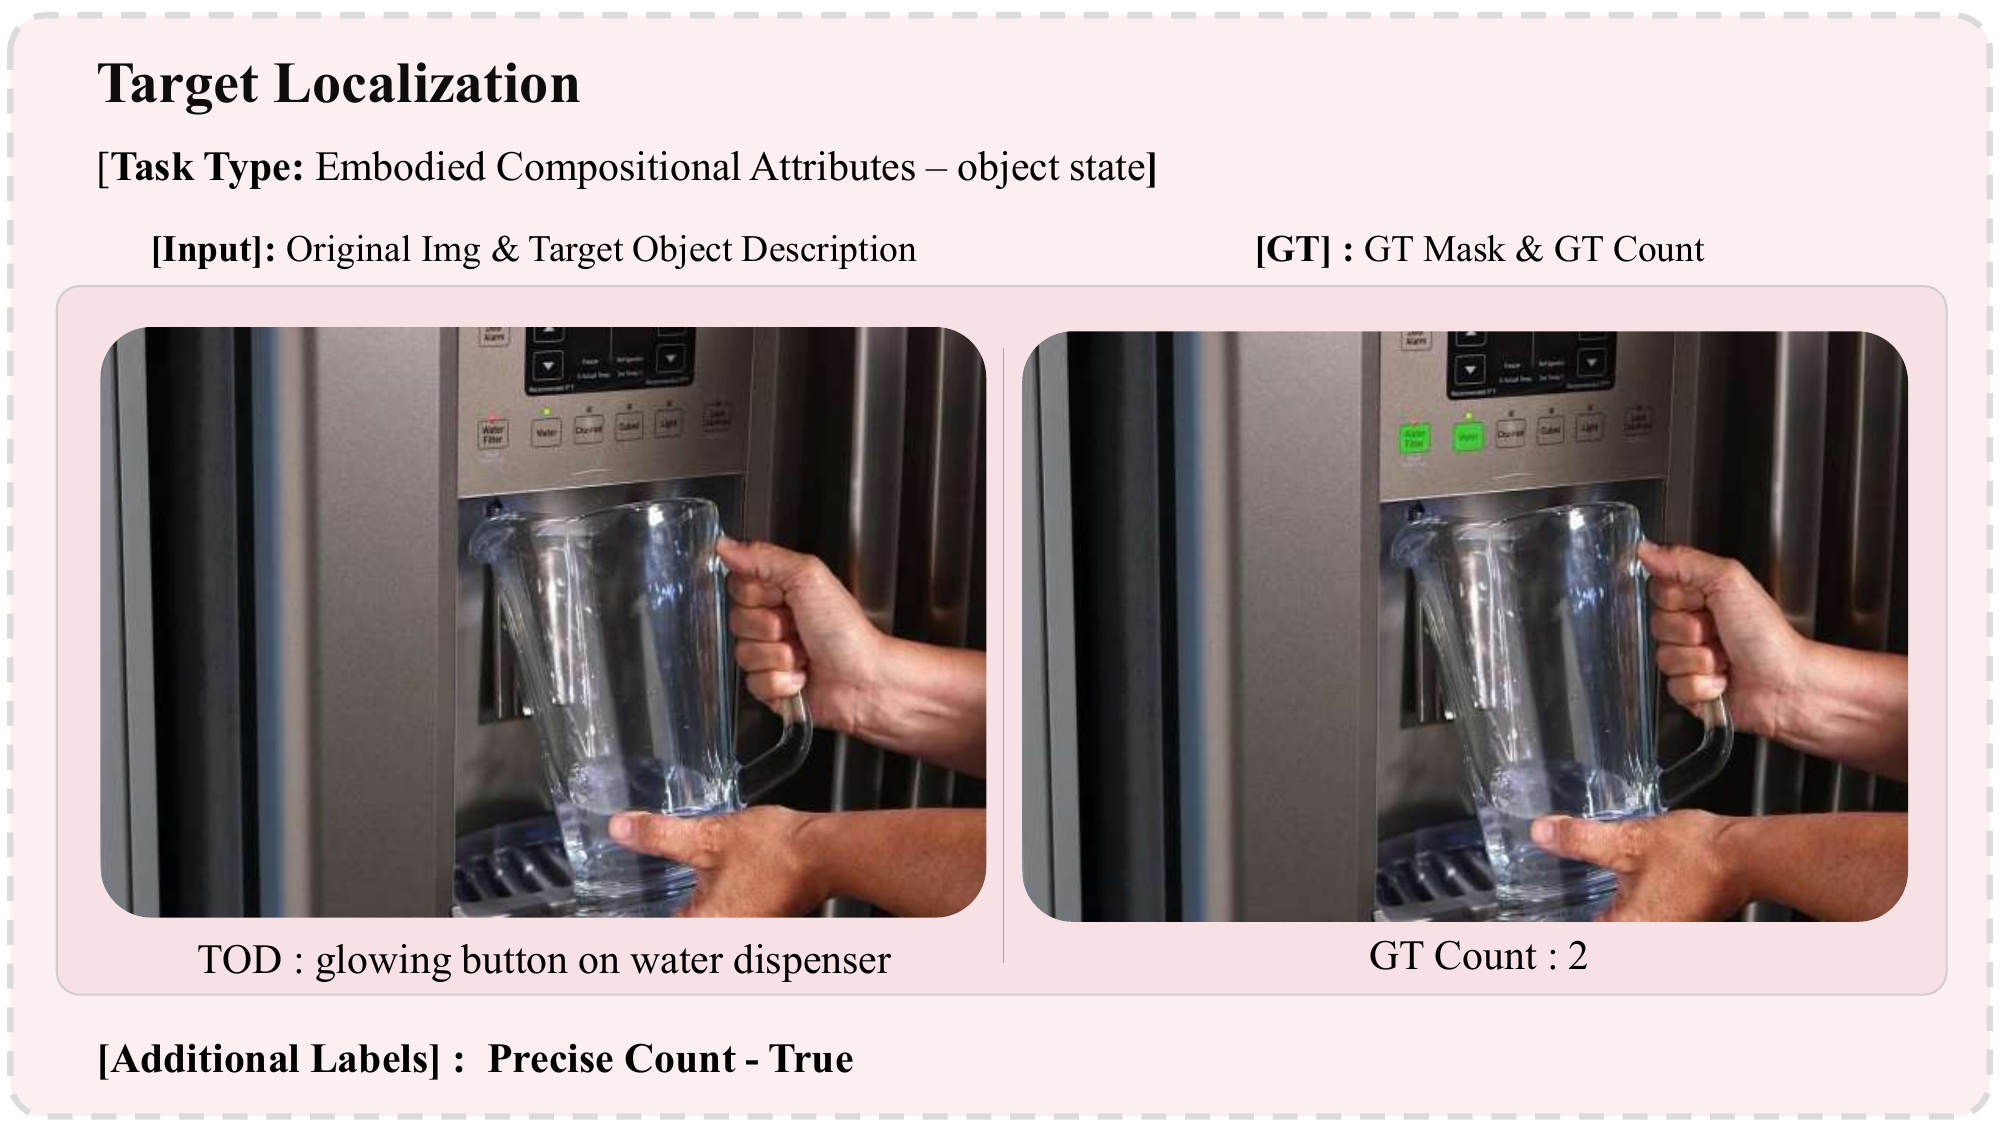}
\includegraphics[width=0.48\textwidth]{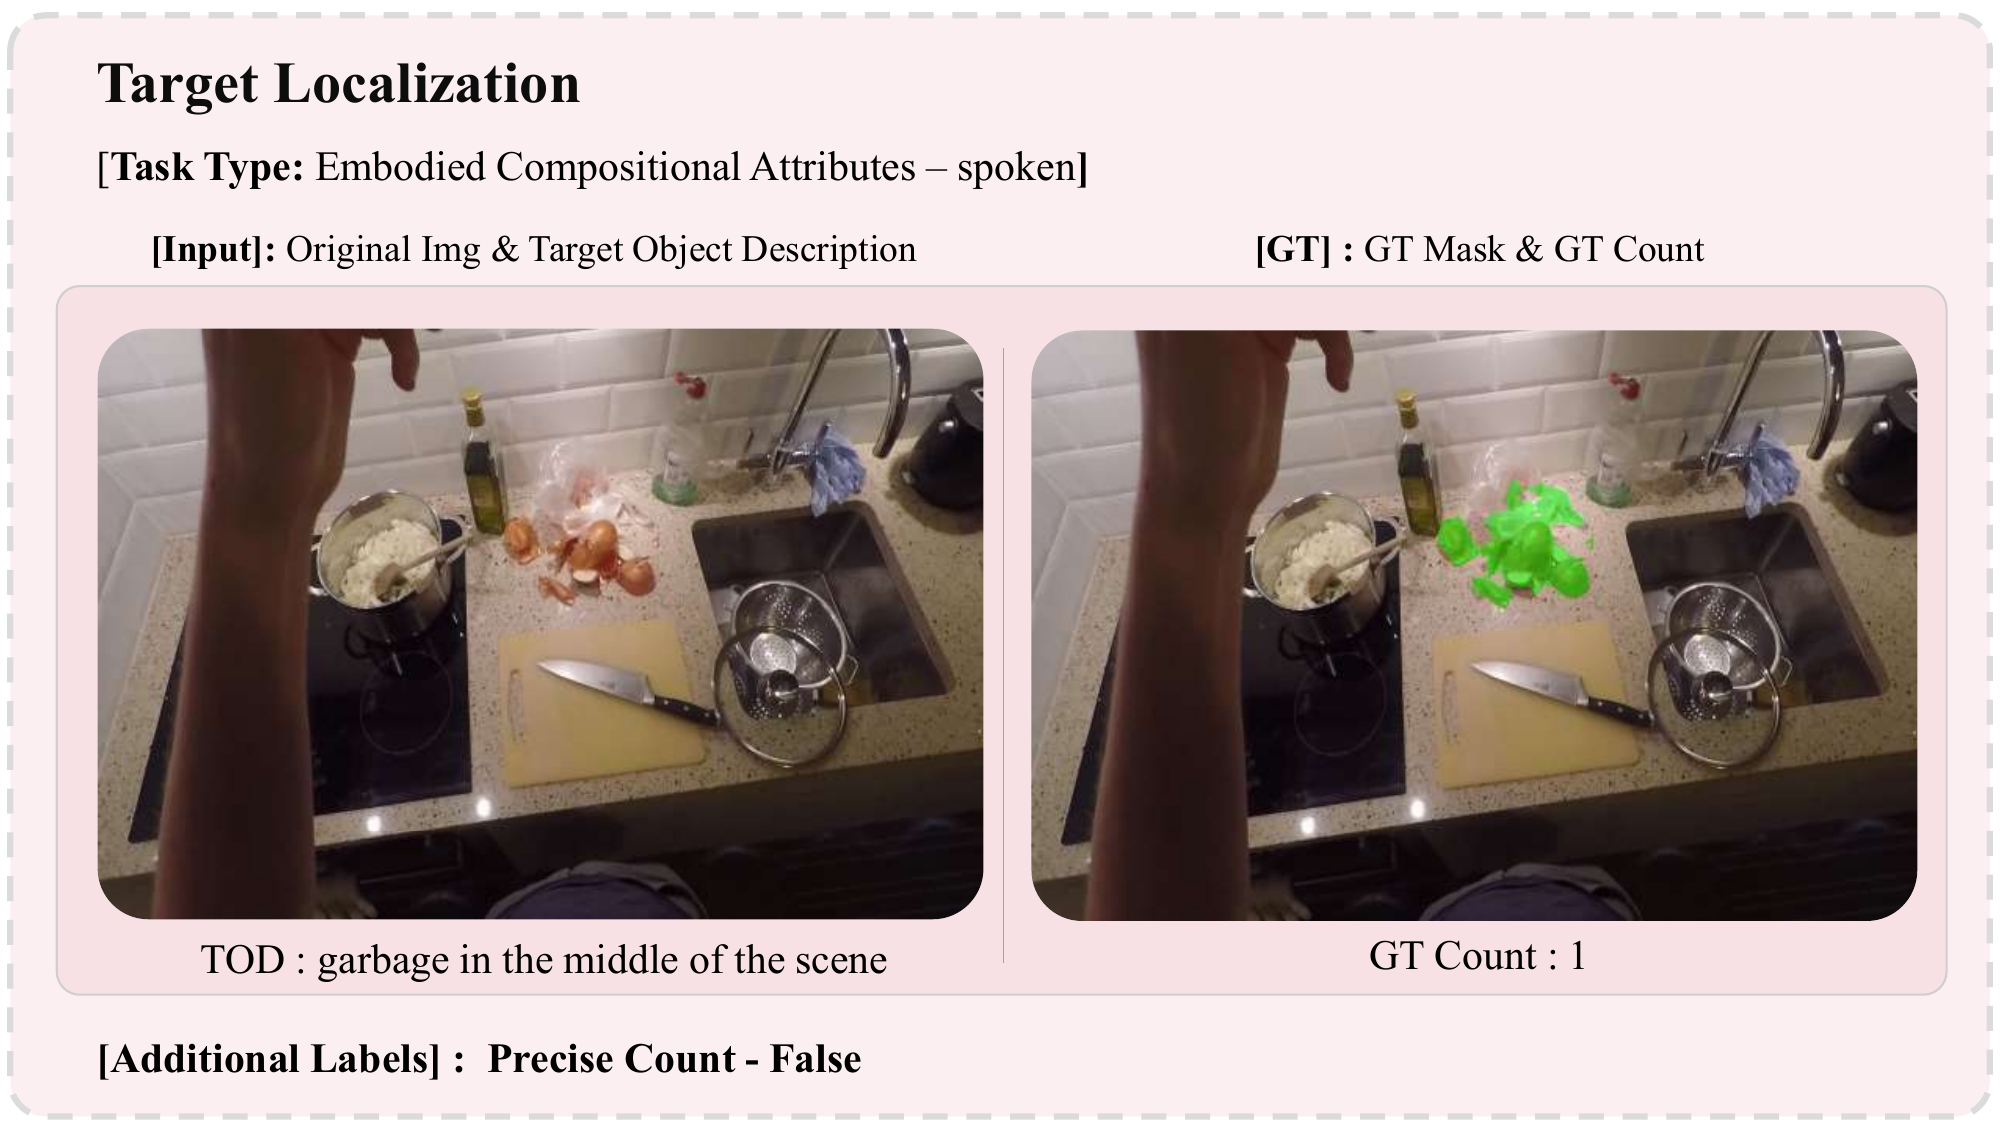}
\includegraphics[width=0.48\textwidth]{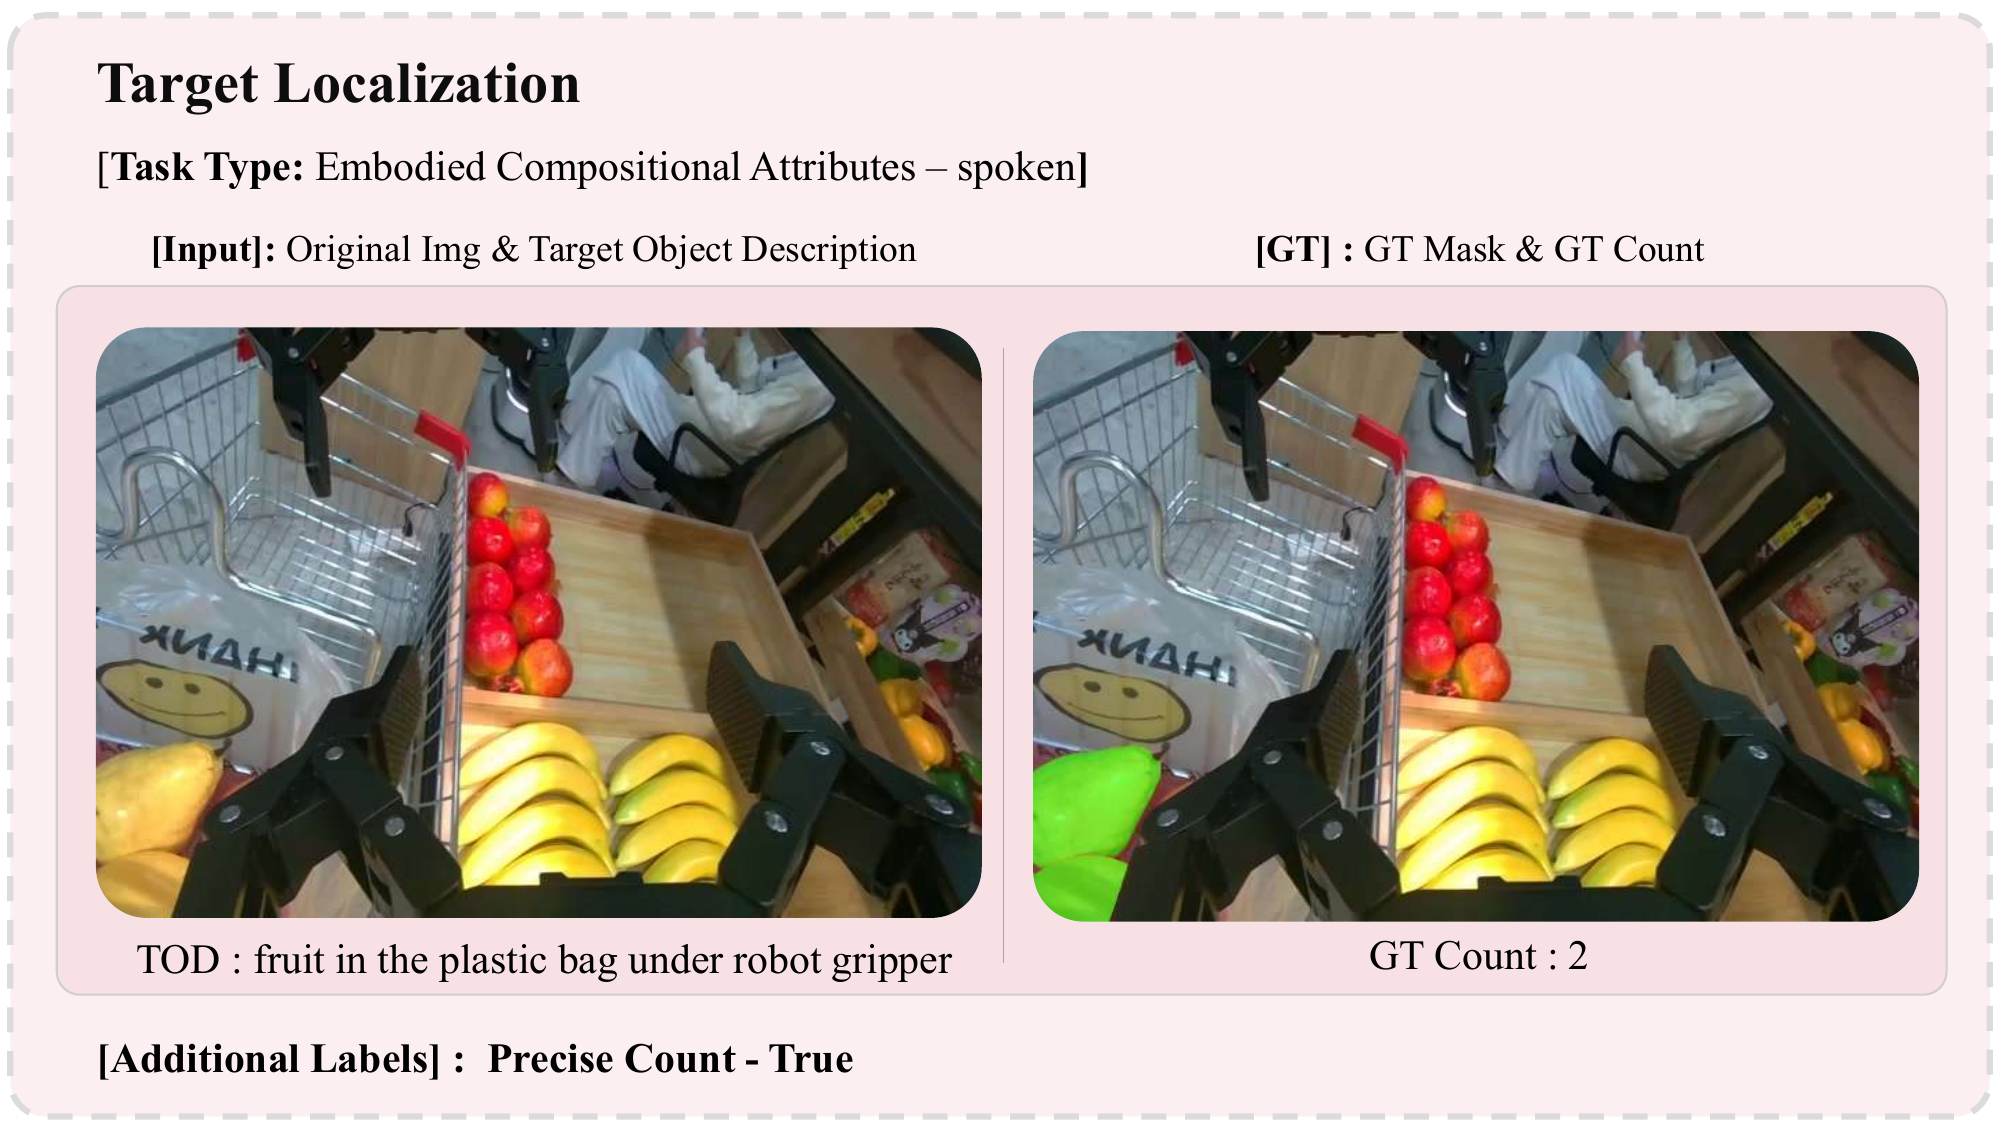}
\caption{Examples of Target Localization - Embodied Compositional Attributes task}
\label{fig:example_TL_ECA}
\end{figure*}





% \clearpage
\begin{figure*}[t]
\centering
\includegraphics[width=0.48\textwidth]{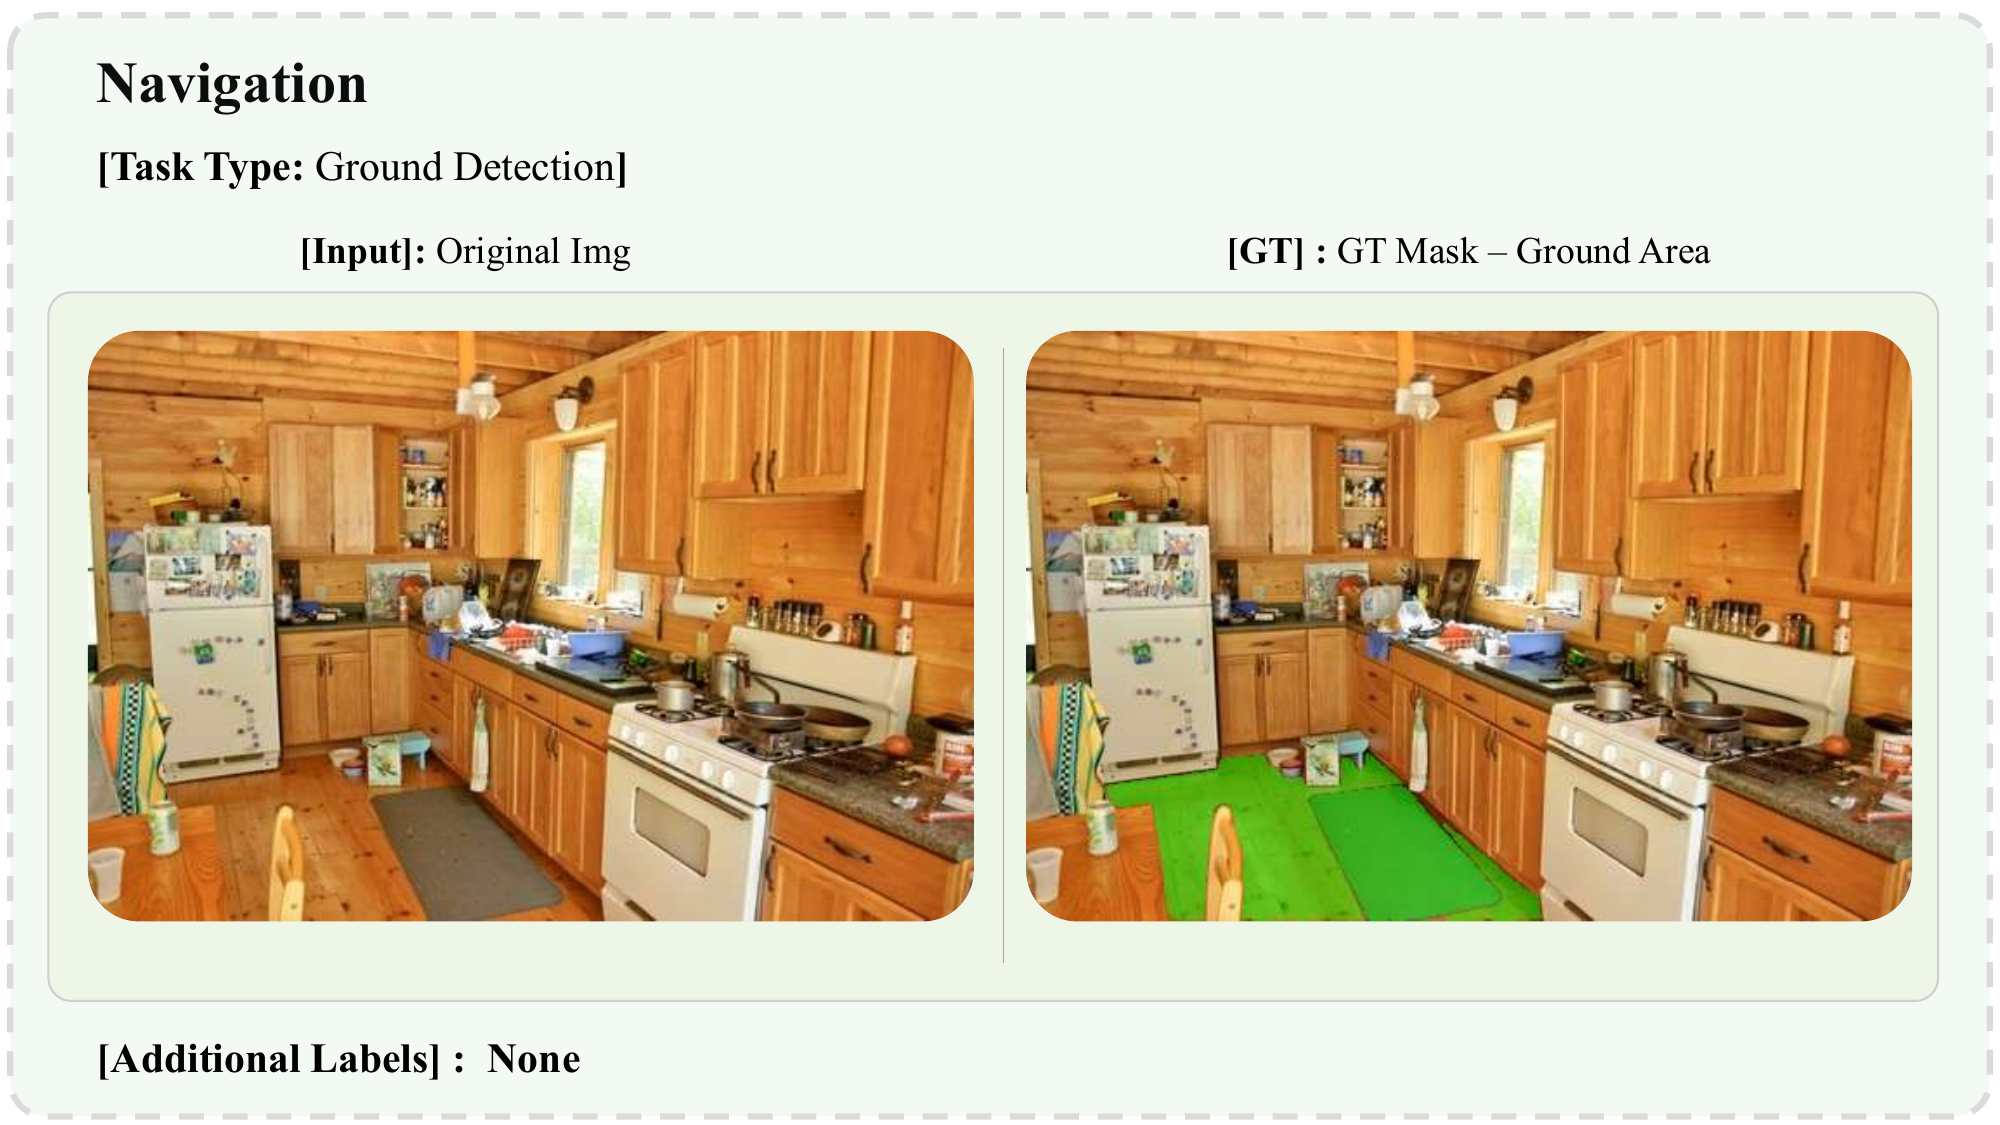}
\includegraphics[width=0.48\textwidth]{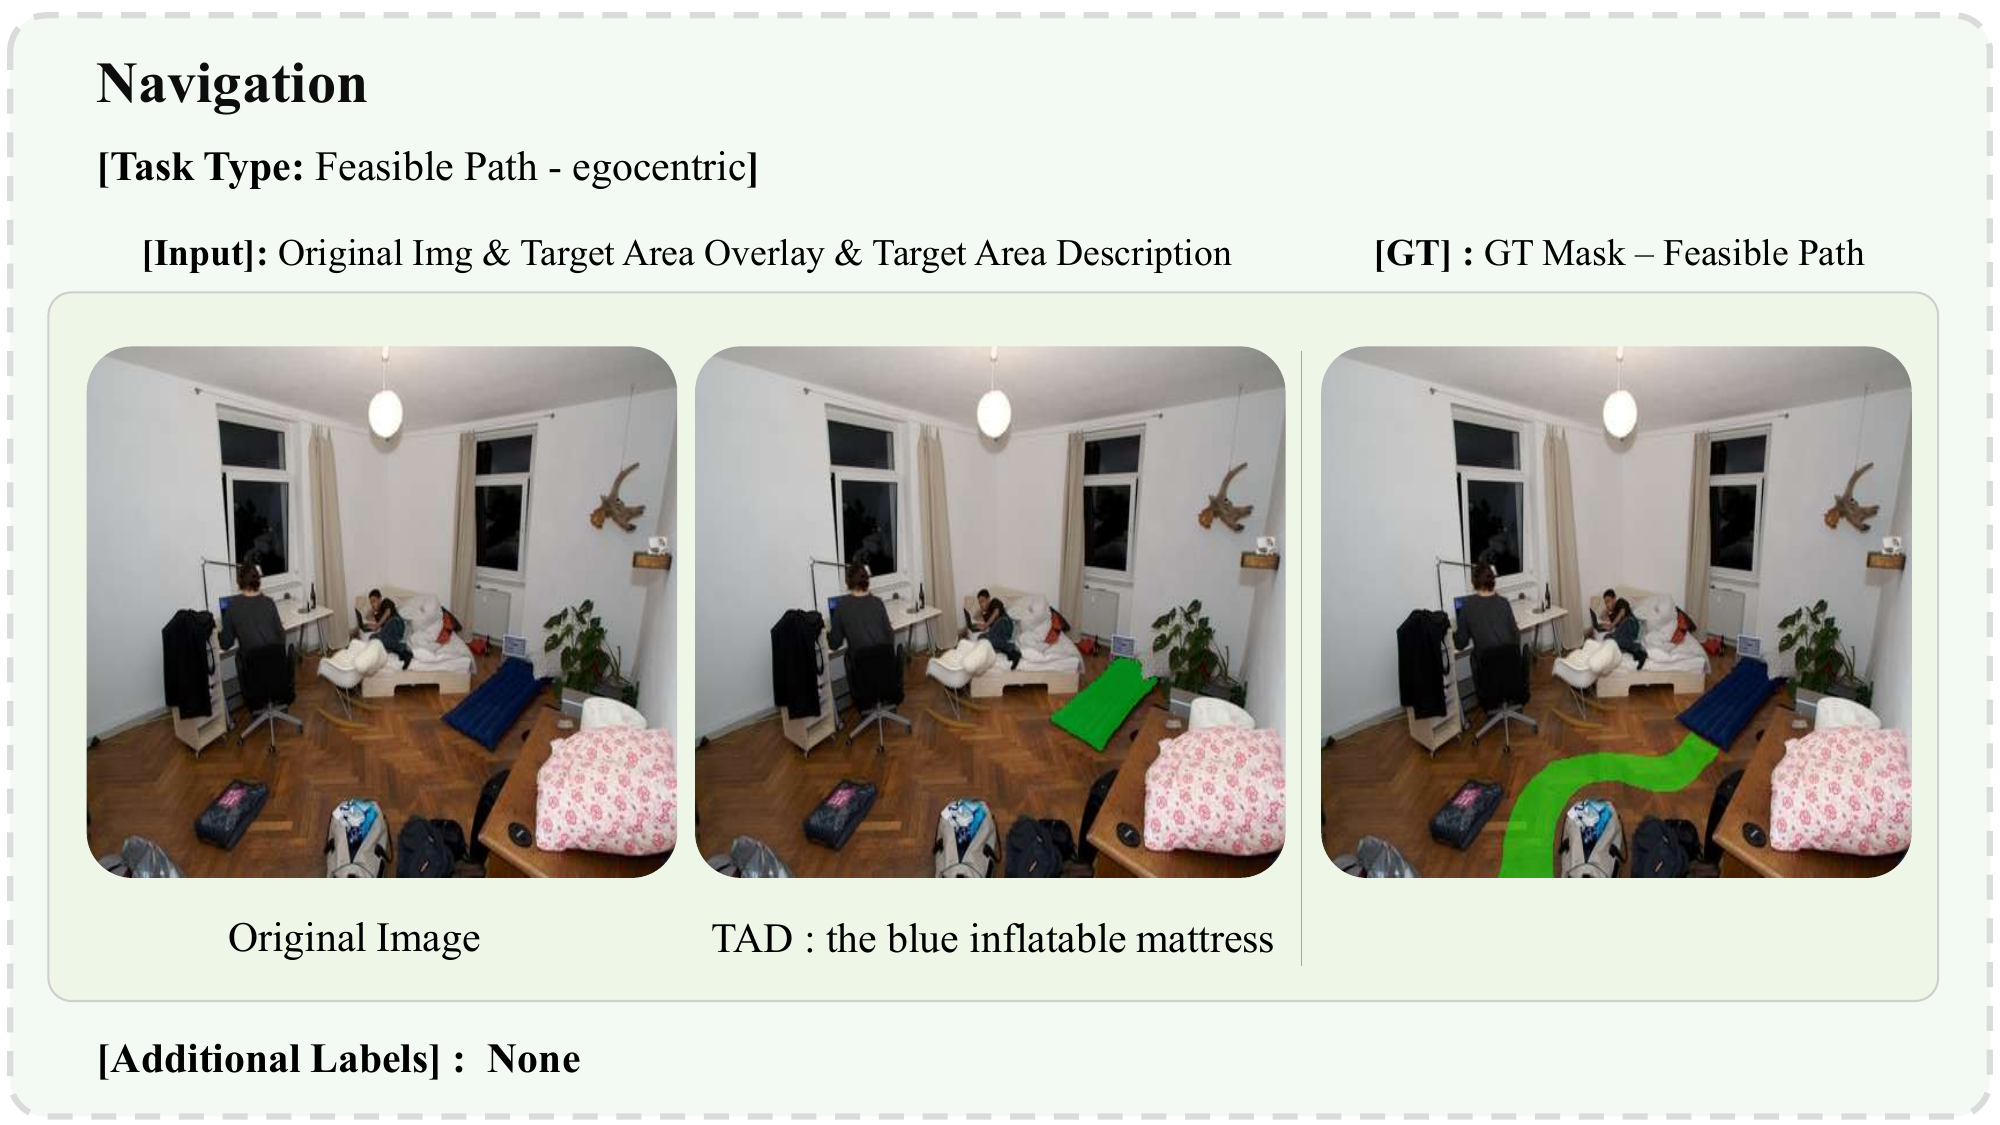}
\includegraphics[width=0.48\textwidth]{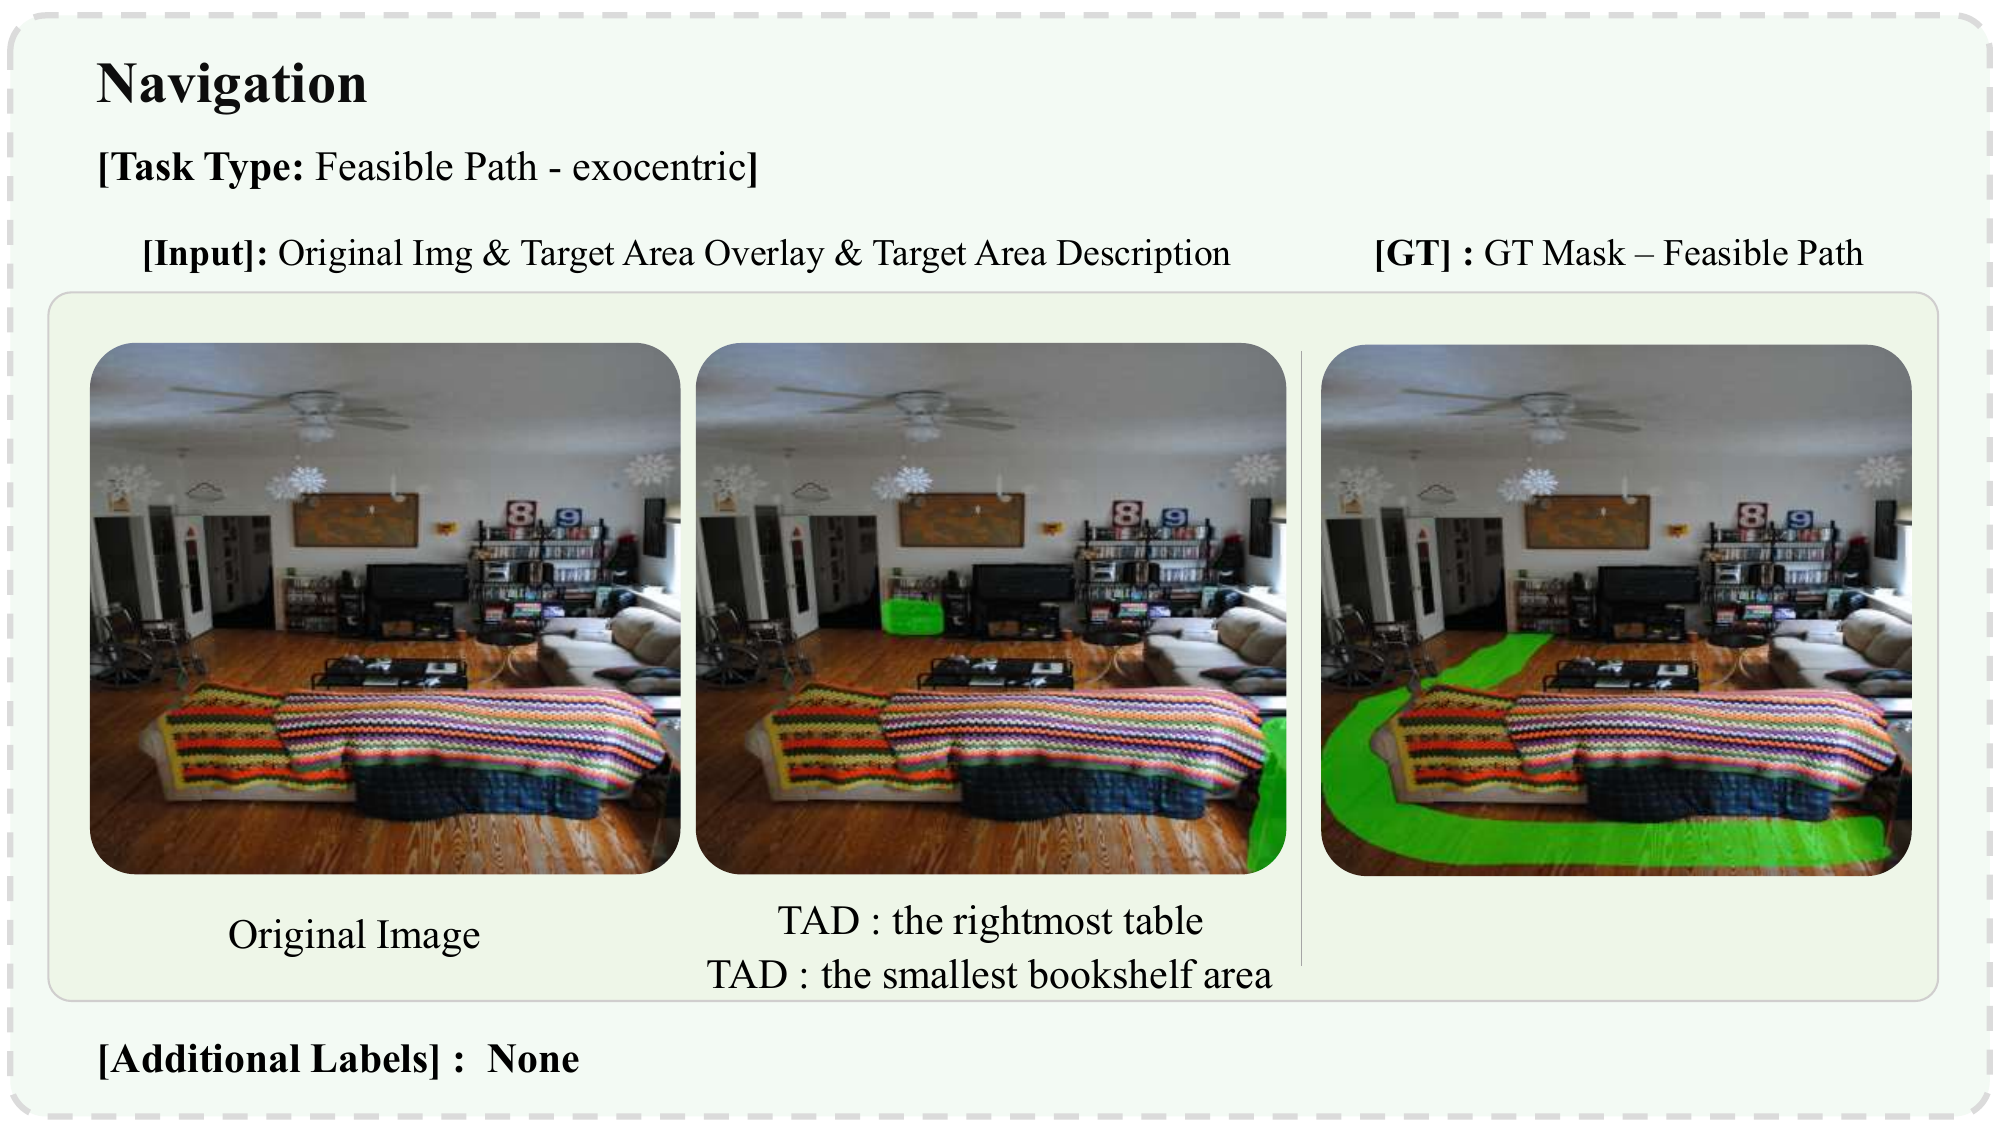}
\includegraphics[width=0.48\textwidth]{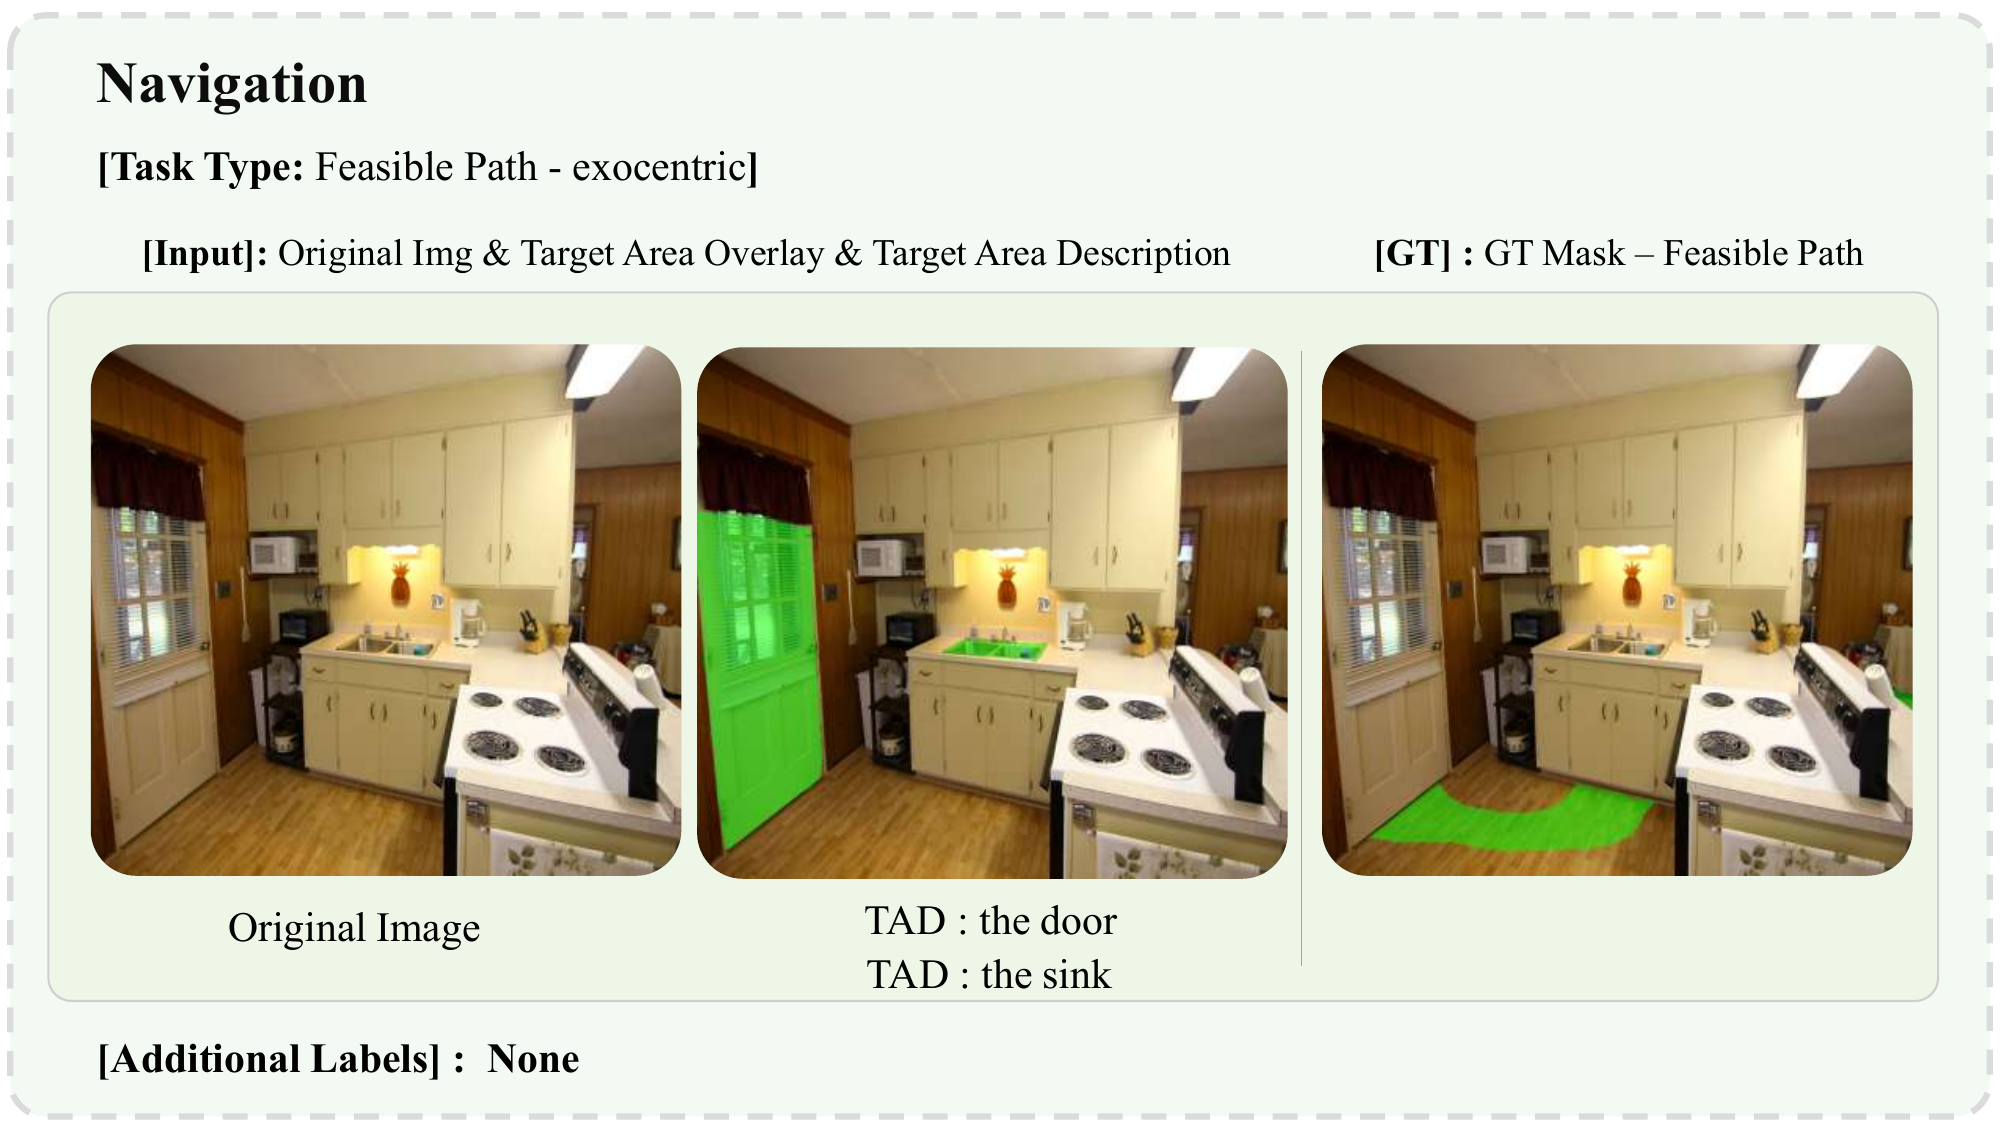}
\includegraphics[width=0.48\textwidth]{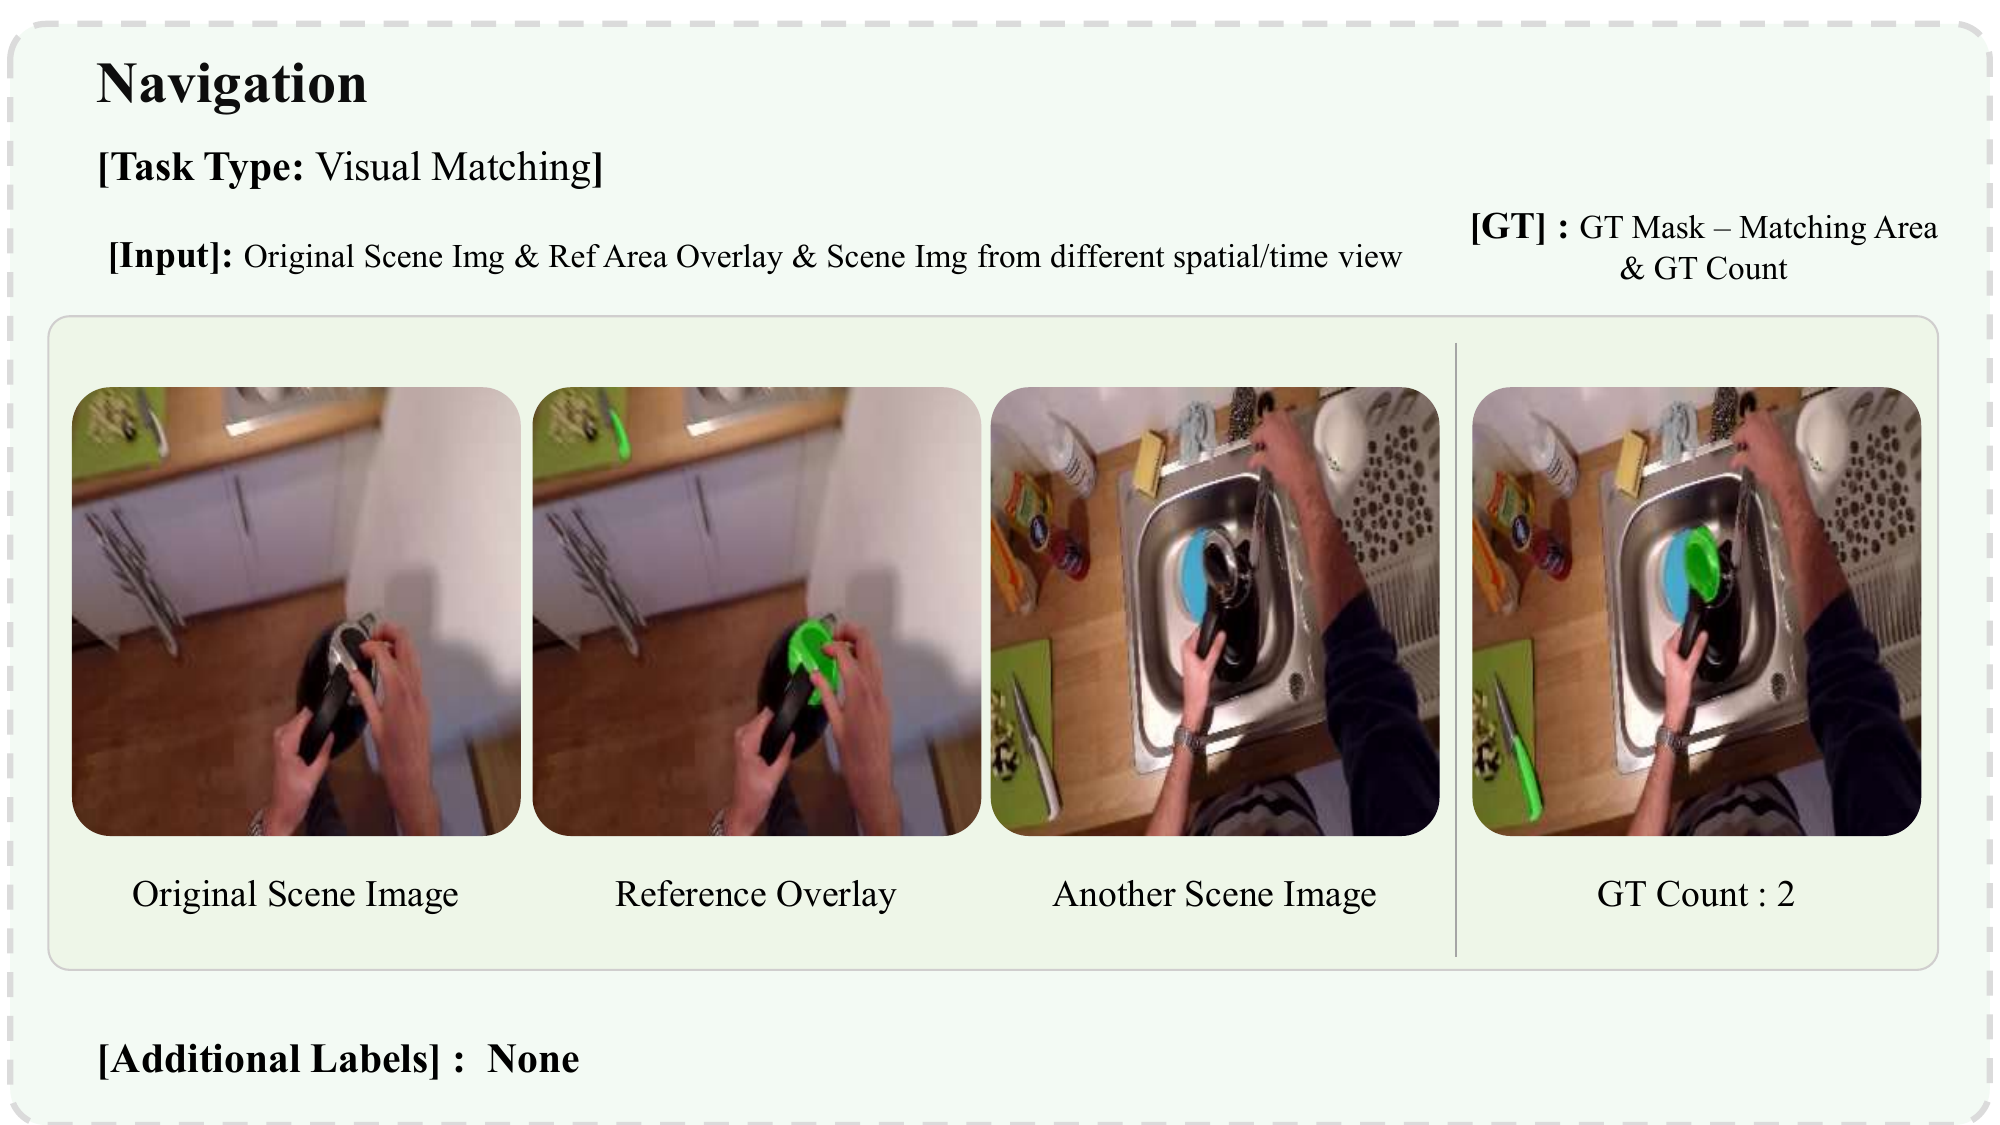}
\includegraphics[width=0.48\textwidth]{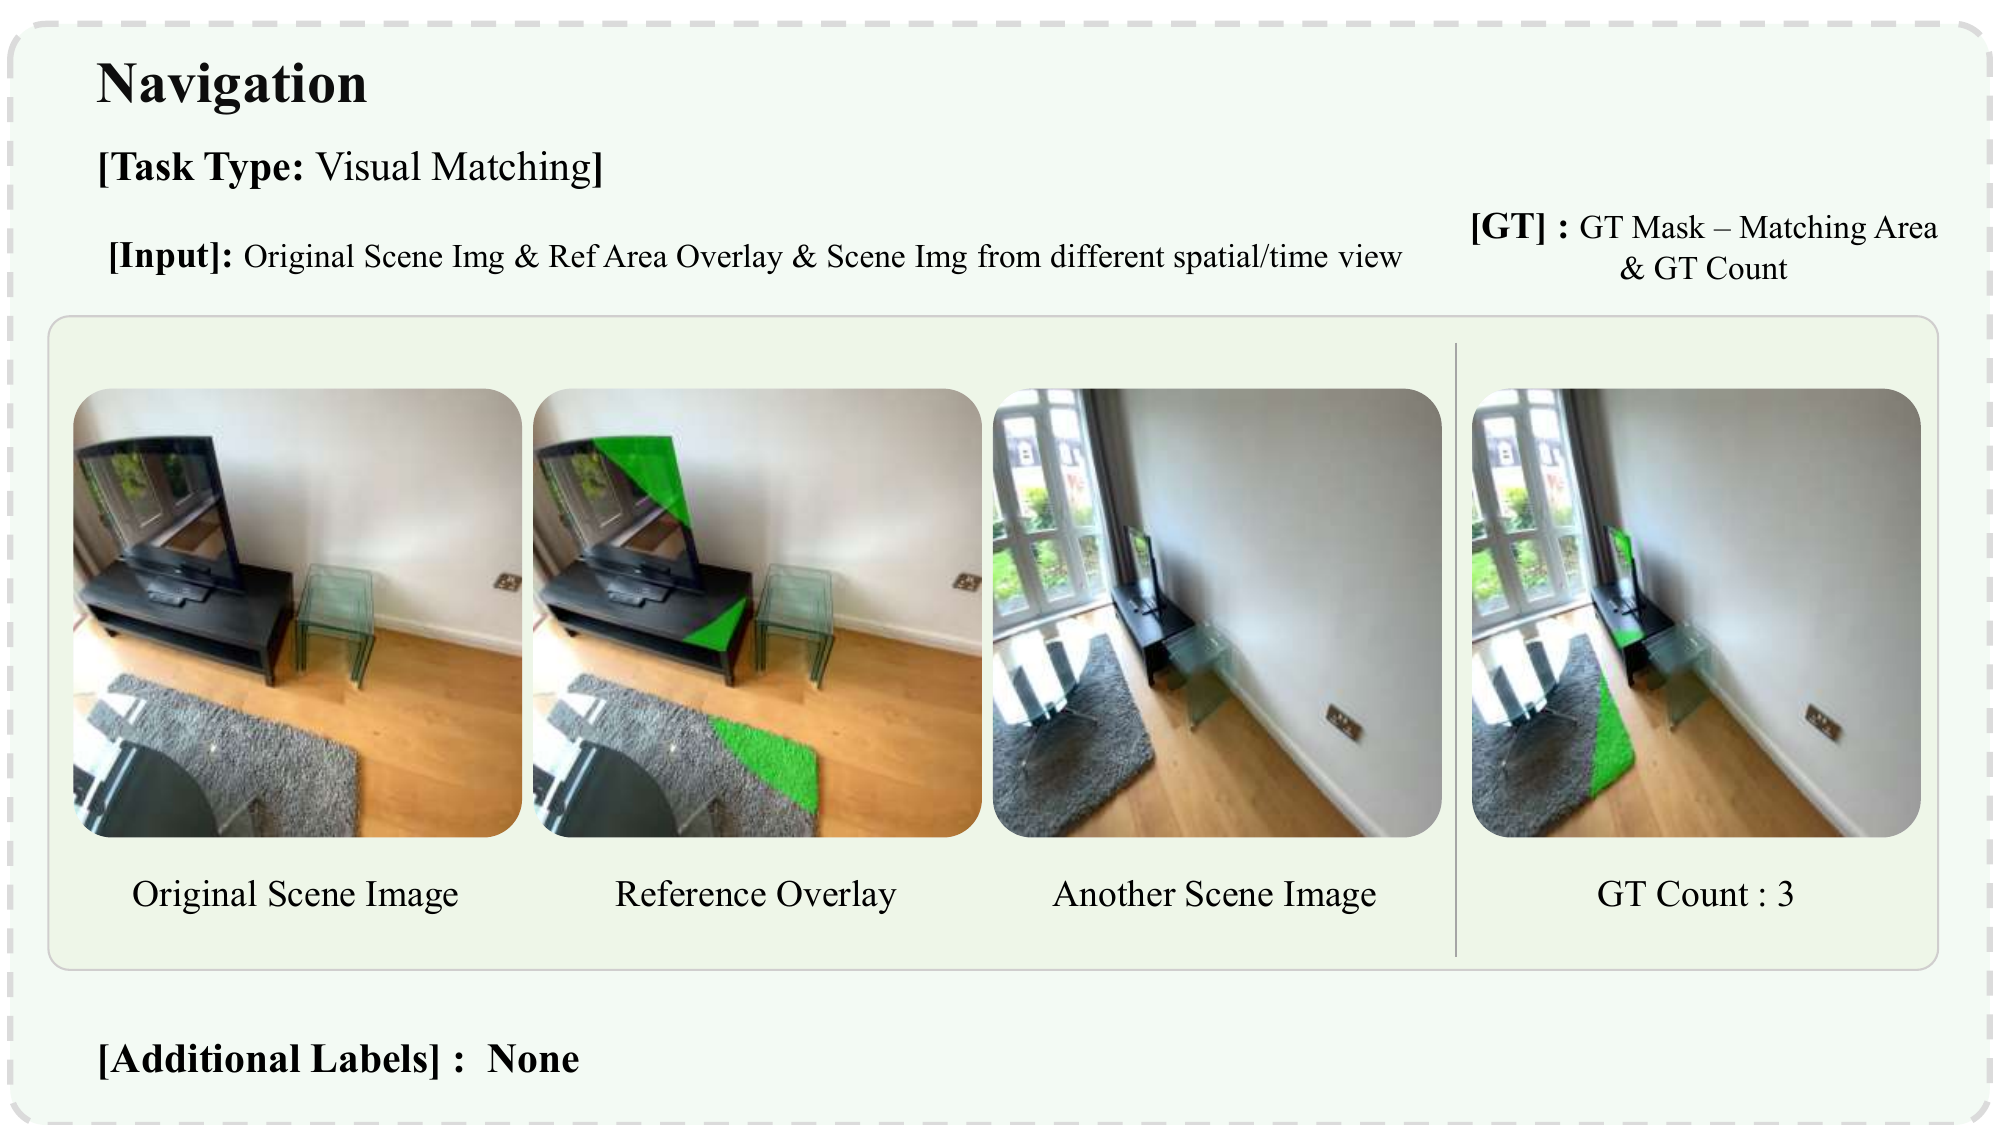}

\caption{Examples of Navigation tasks}
\label{fig:example_NAV}
\end{figure*}





% \clearpage
\begin{figure*}[t]
\centering
\includegraphics[width=0.48\textwidth]{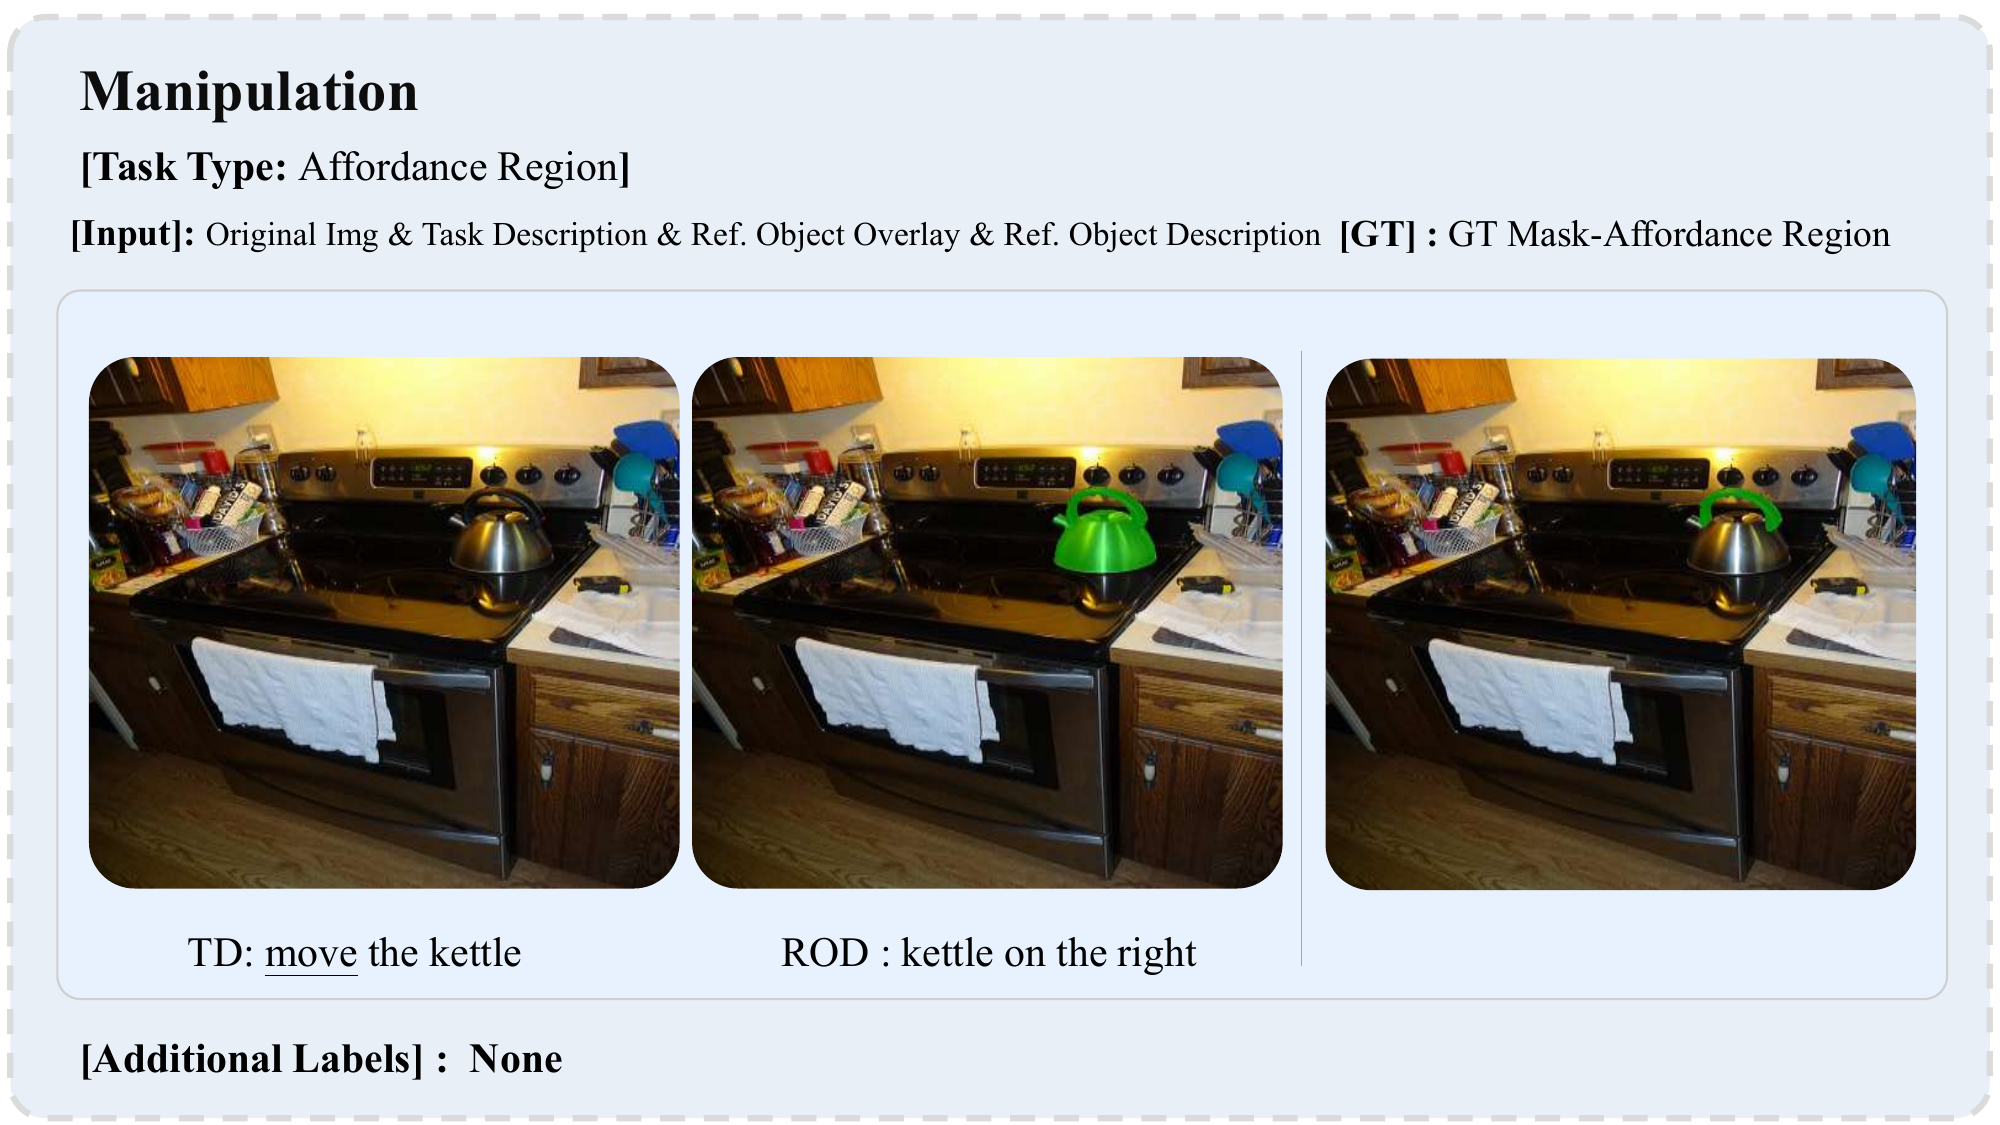}
\includegraphics[width=0.48\textwidth]{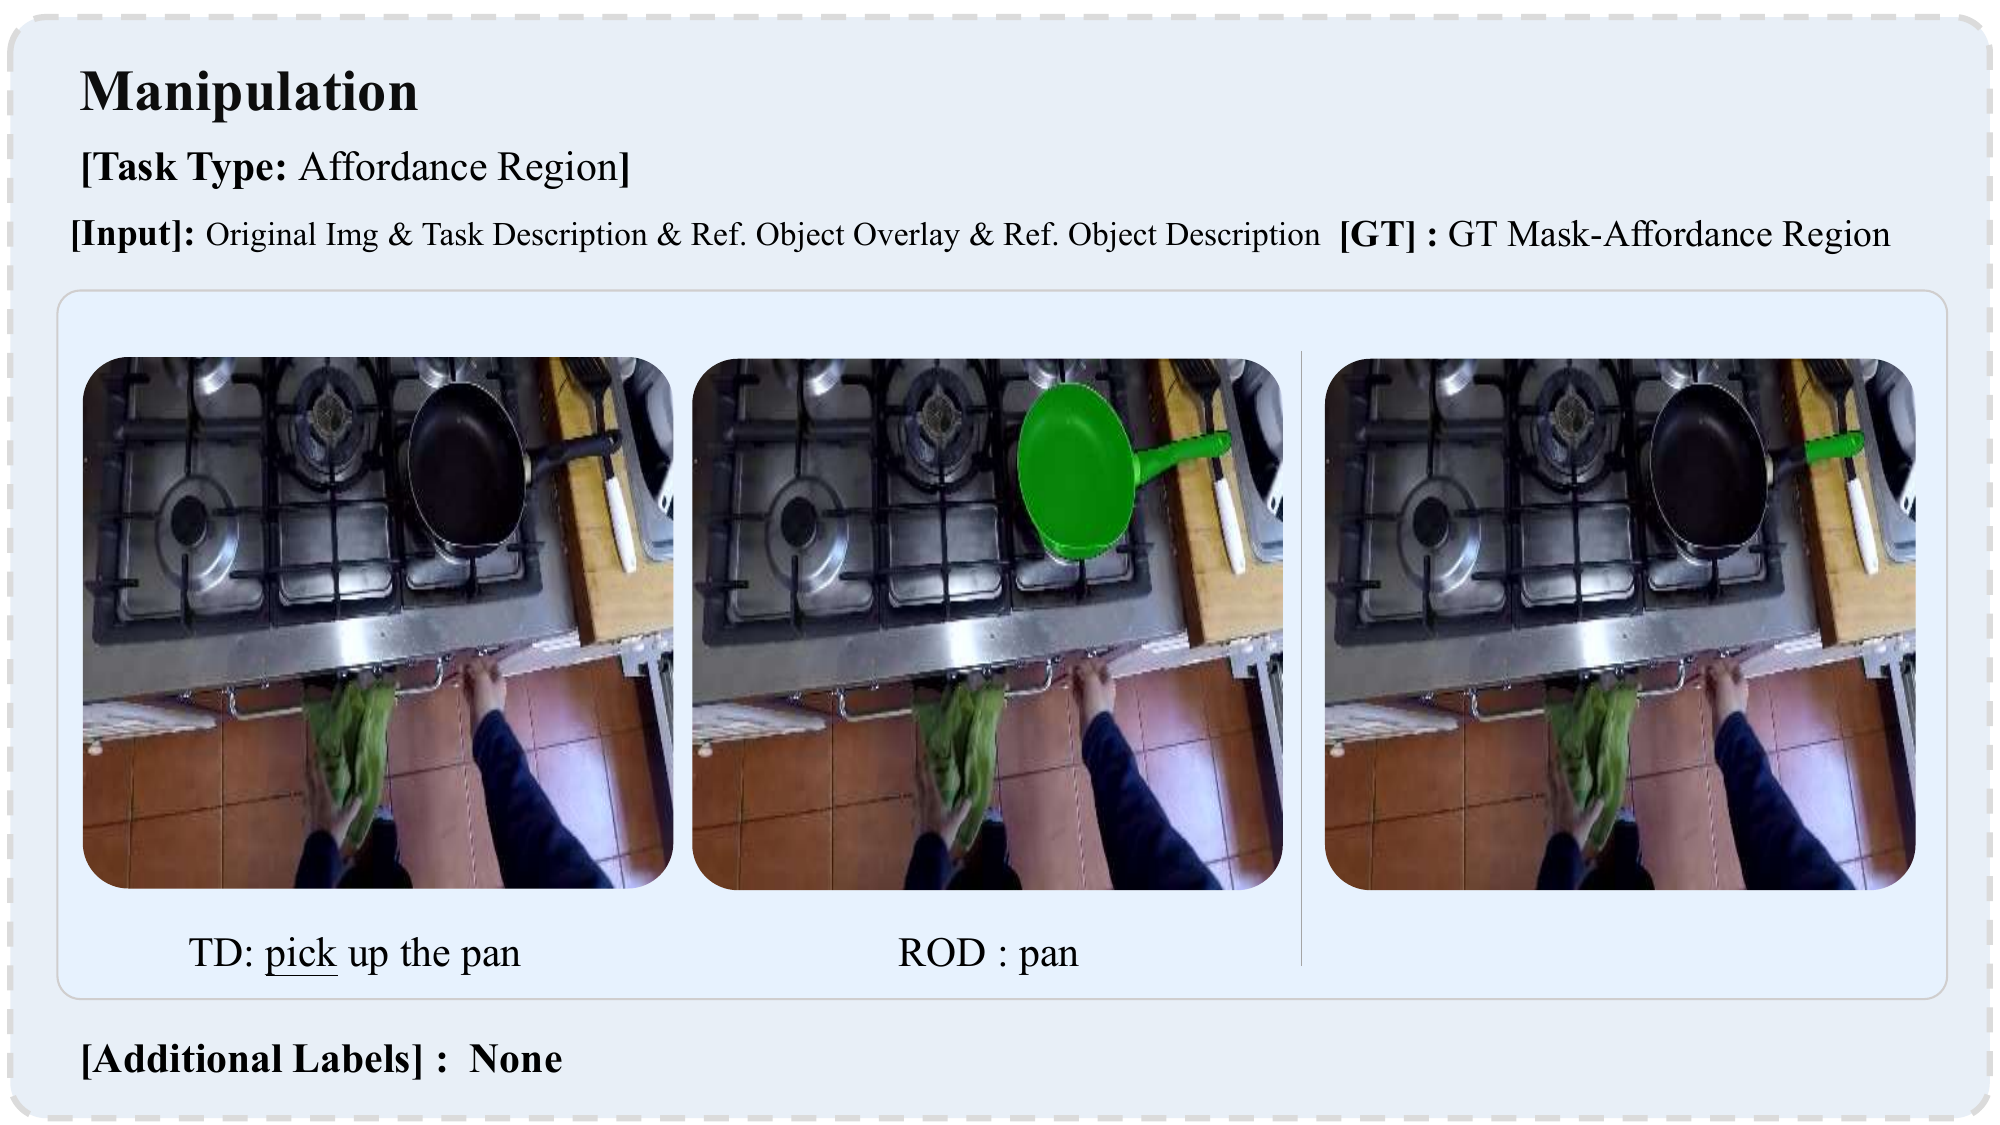}

\includegraphics[width=0.48\textwidth]{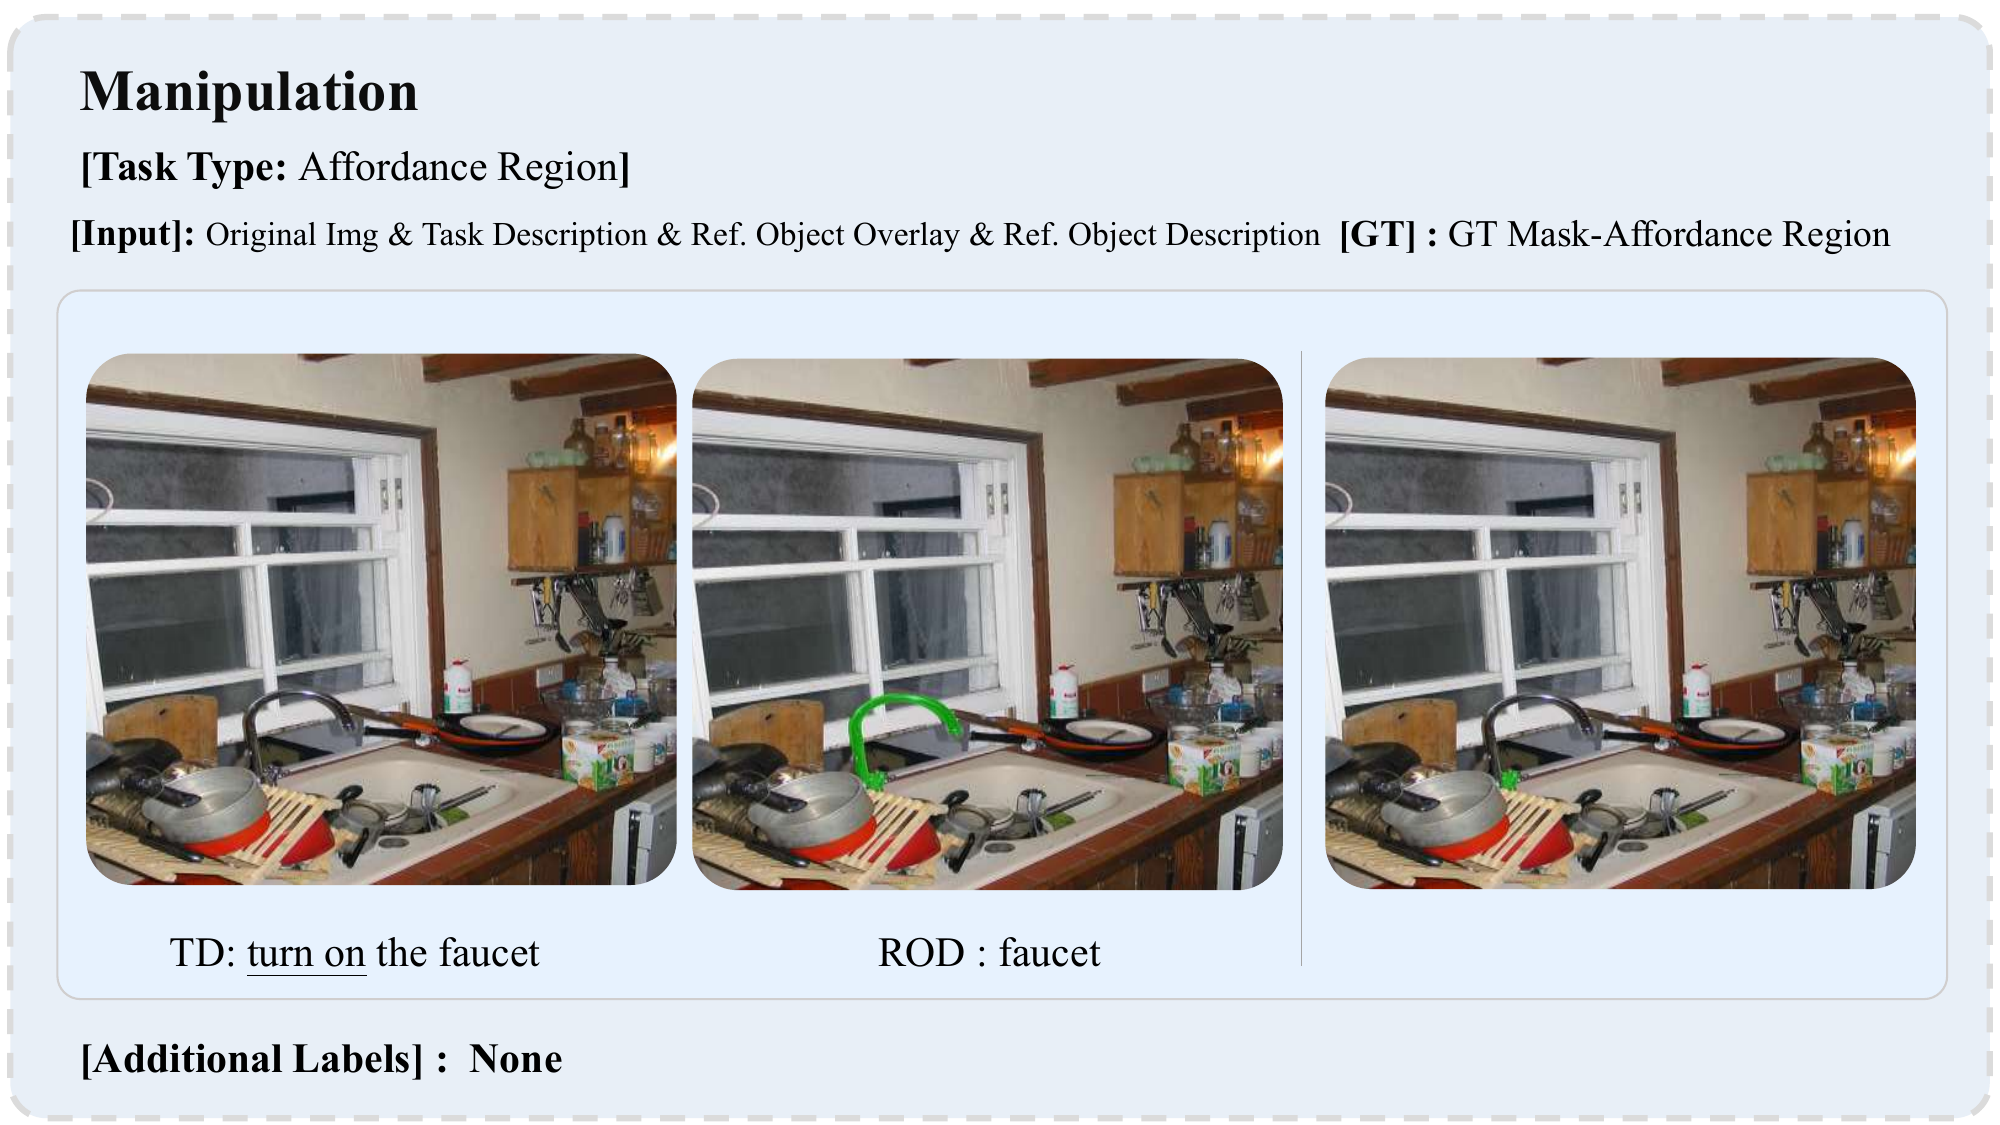}
\includegraphics[width=0.48\textwidth]{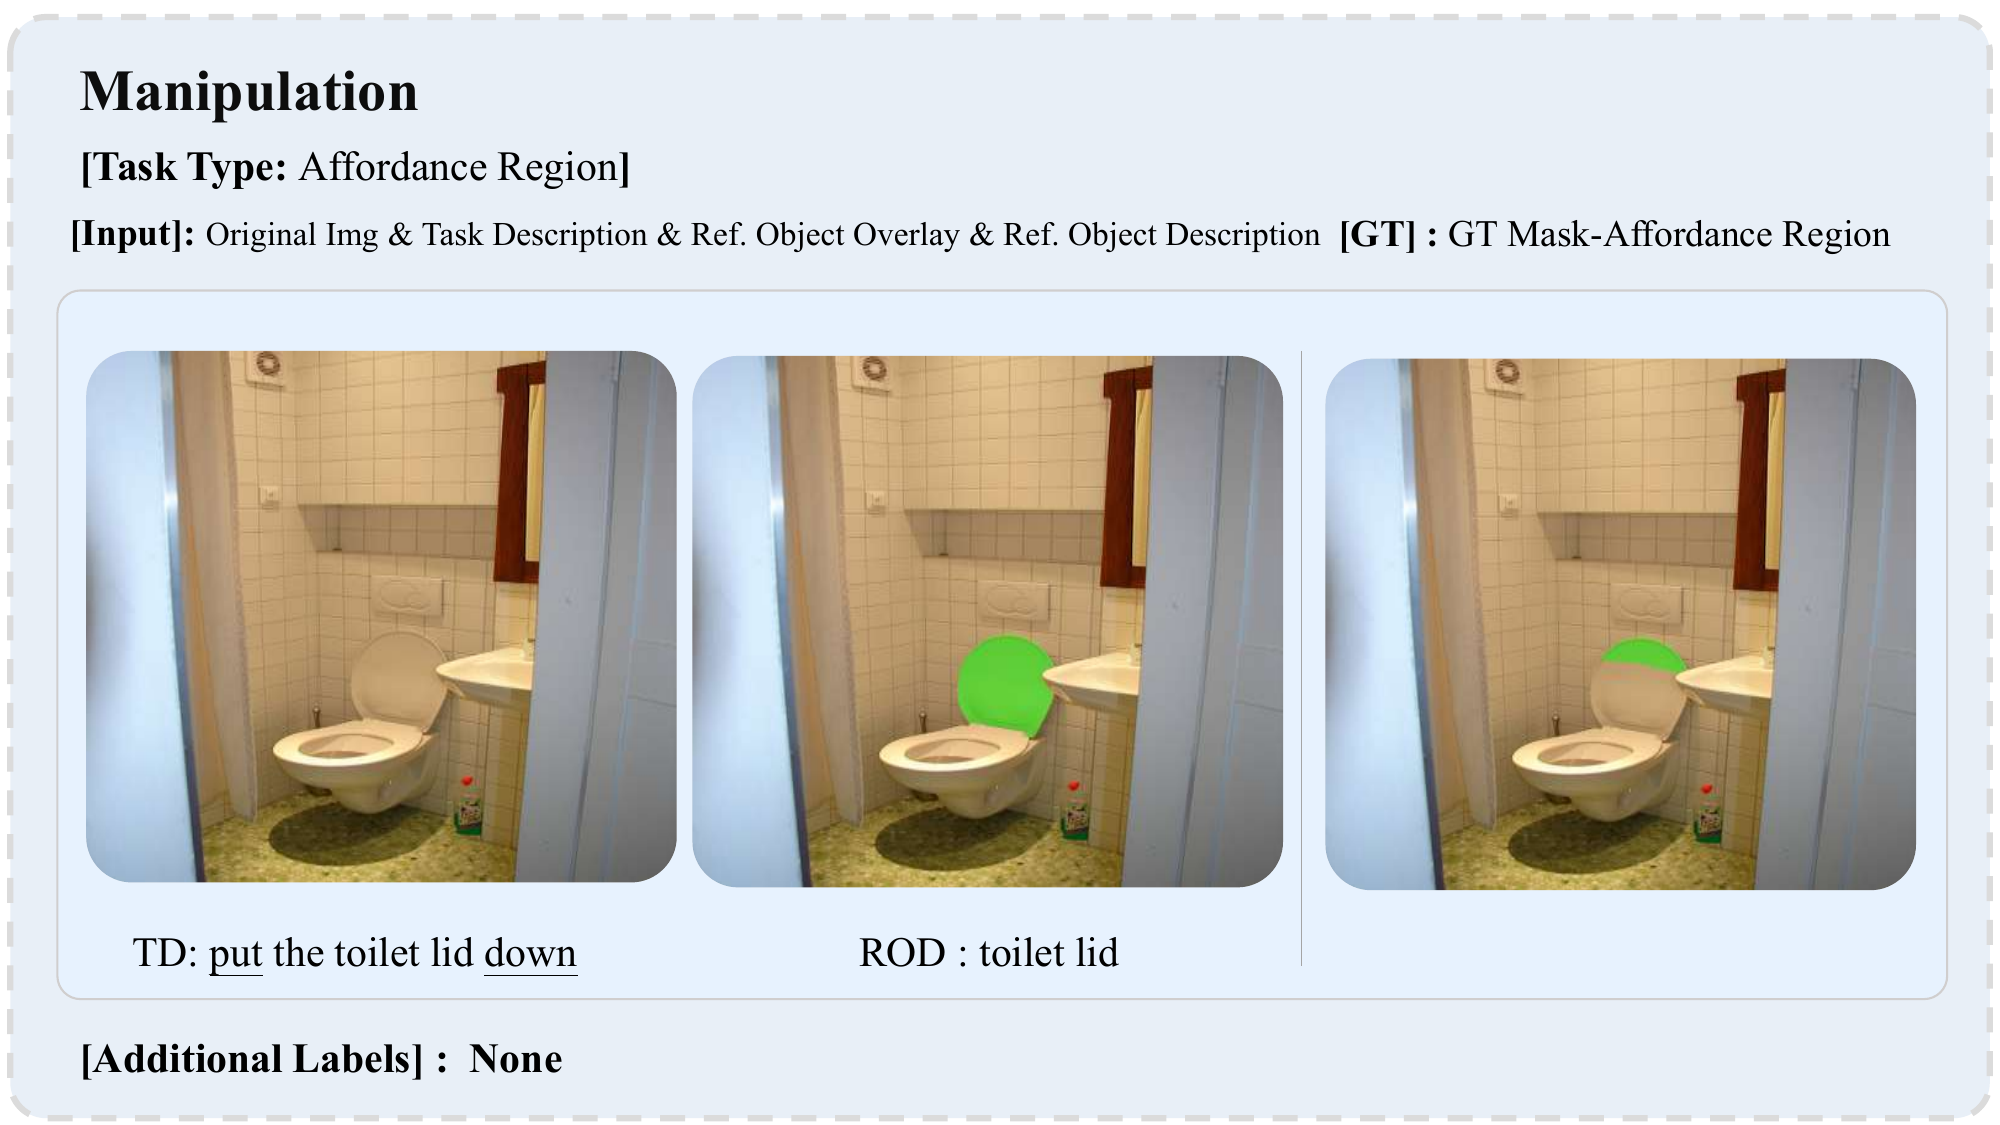}

\includegraphics[width=0.48\textwidth]{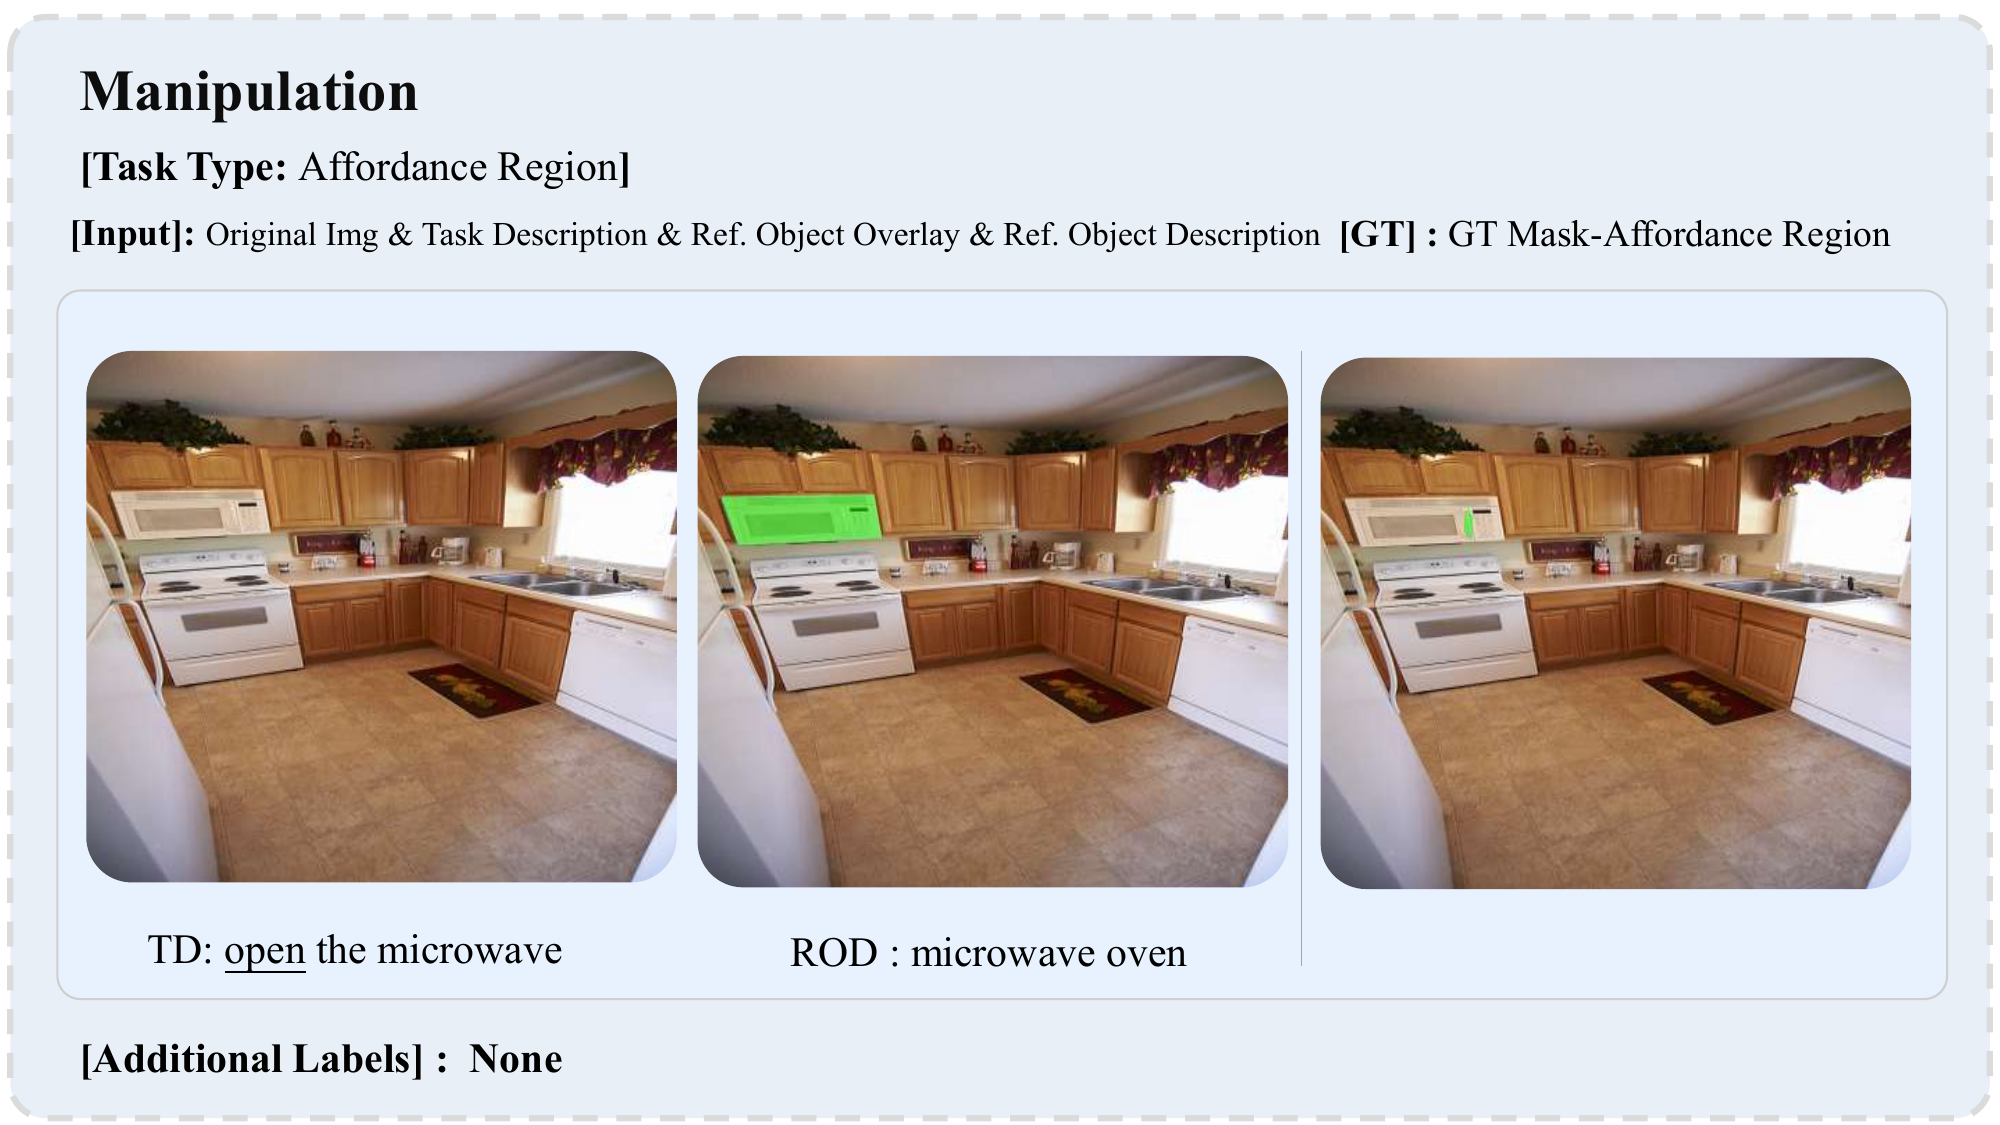}
\includegraphics[width=0.48\textwidth]{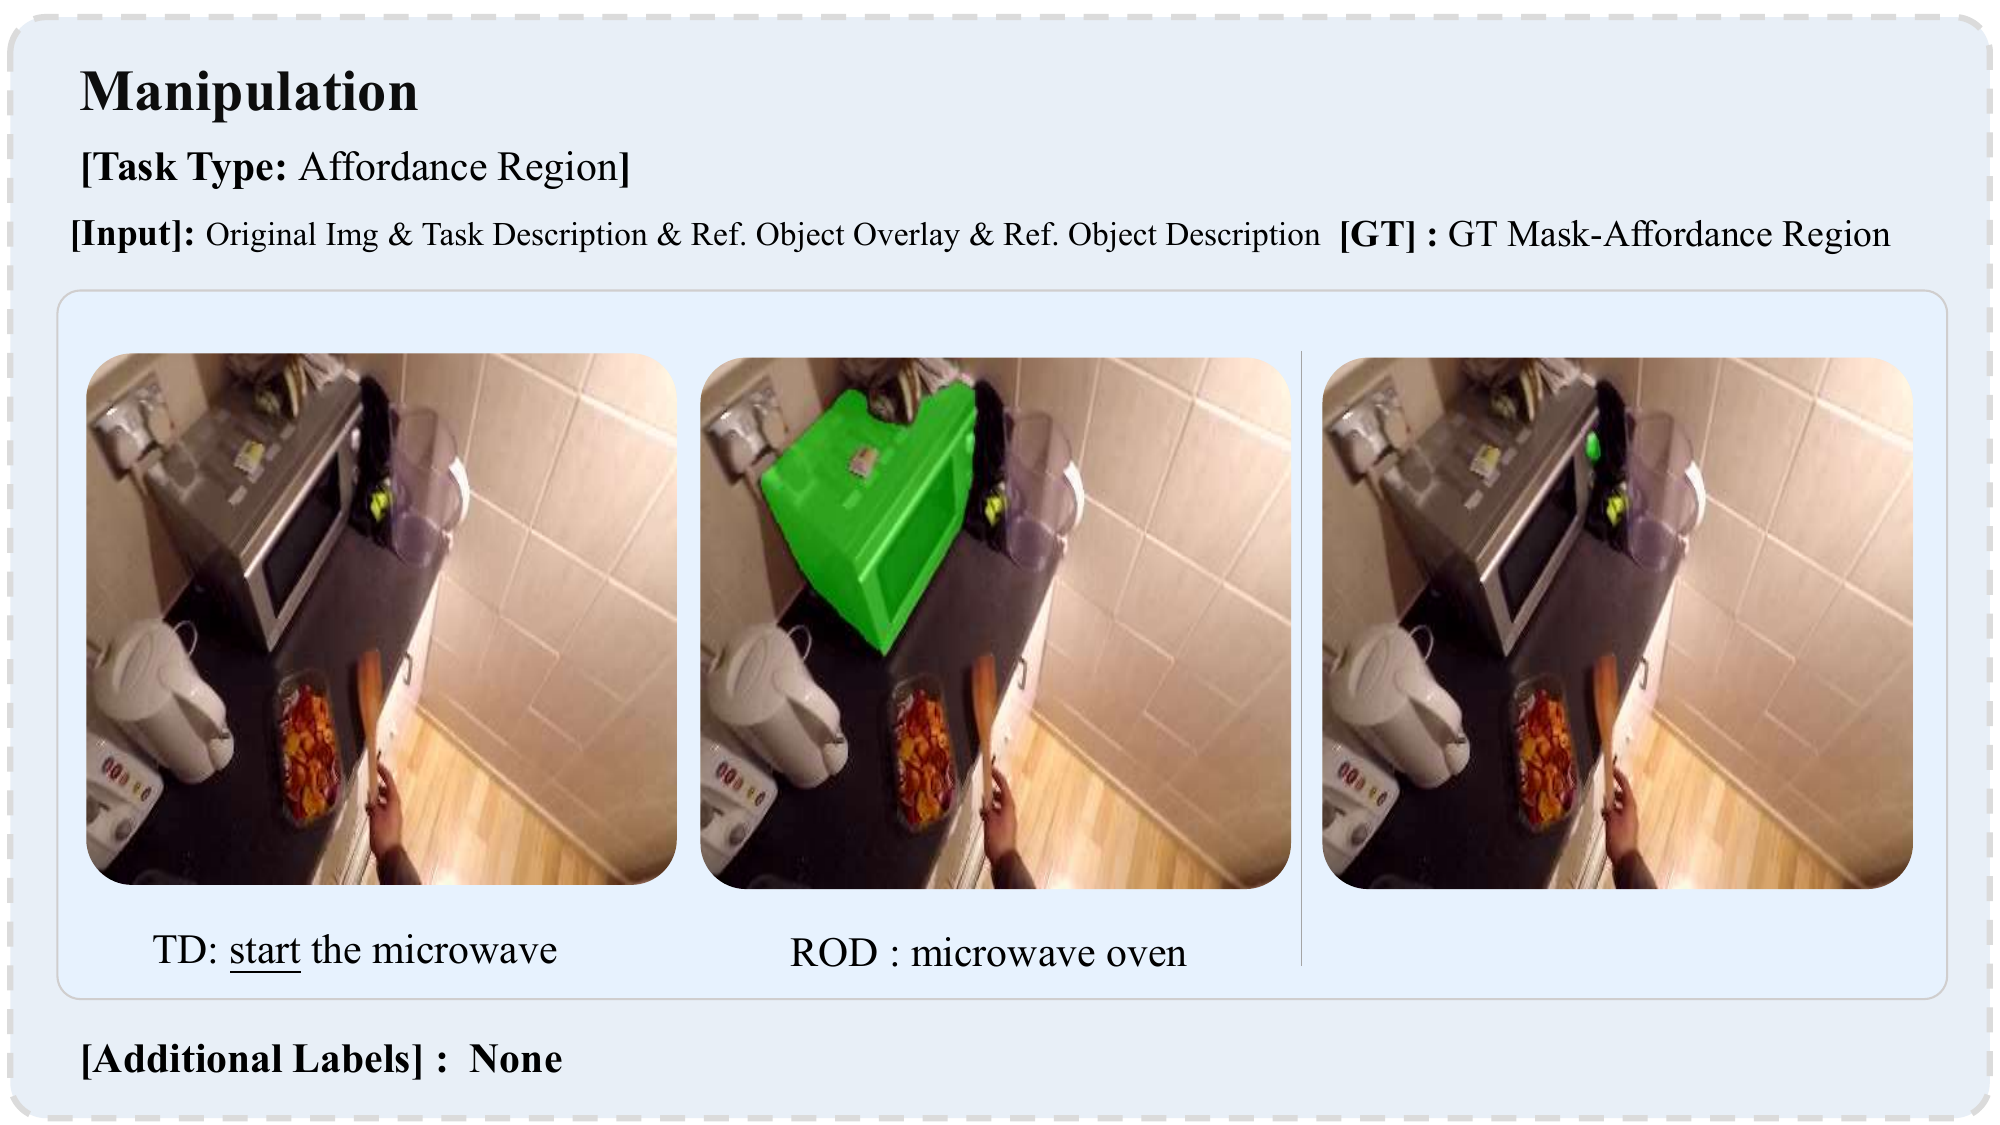}

\caption{Examples of Manipulation - Affordance Region task}
\label{fig:example_MAN_AR}
\end{figure*}


% \clearpage
\begin{figure*}[t]
\centering
\includegraphics[width=0.48\textwidth]{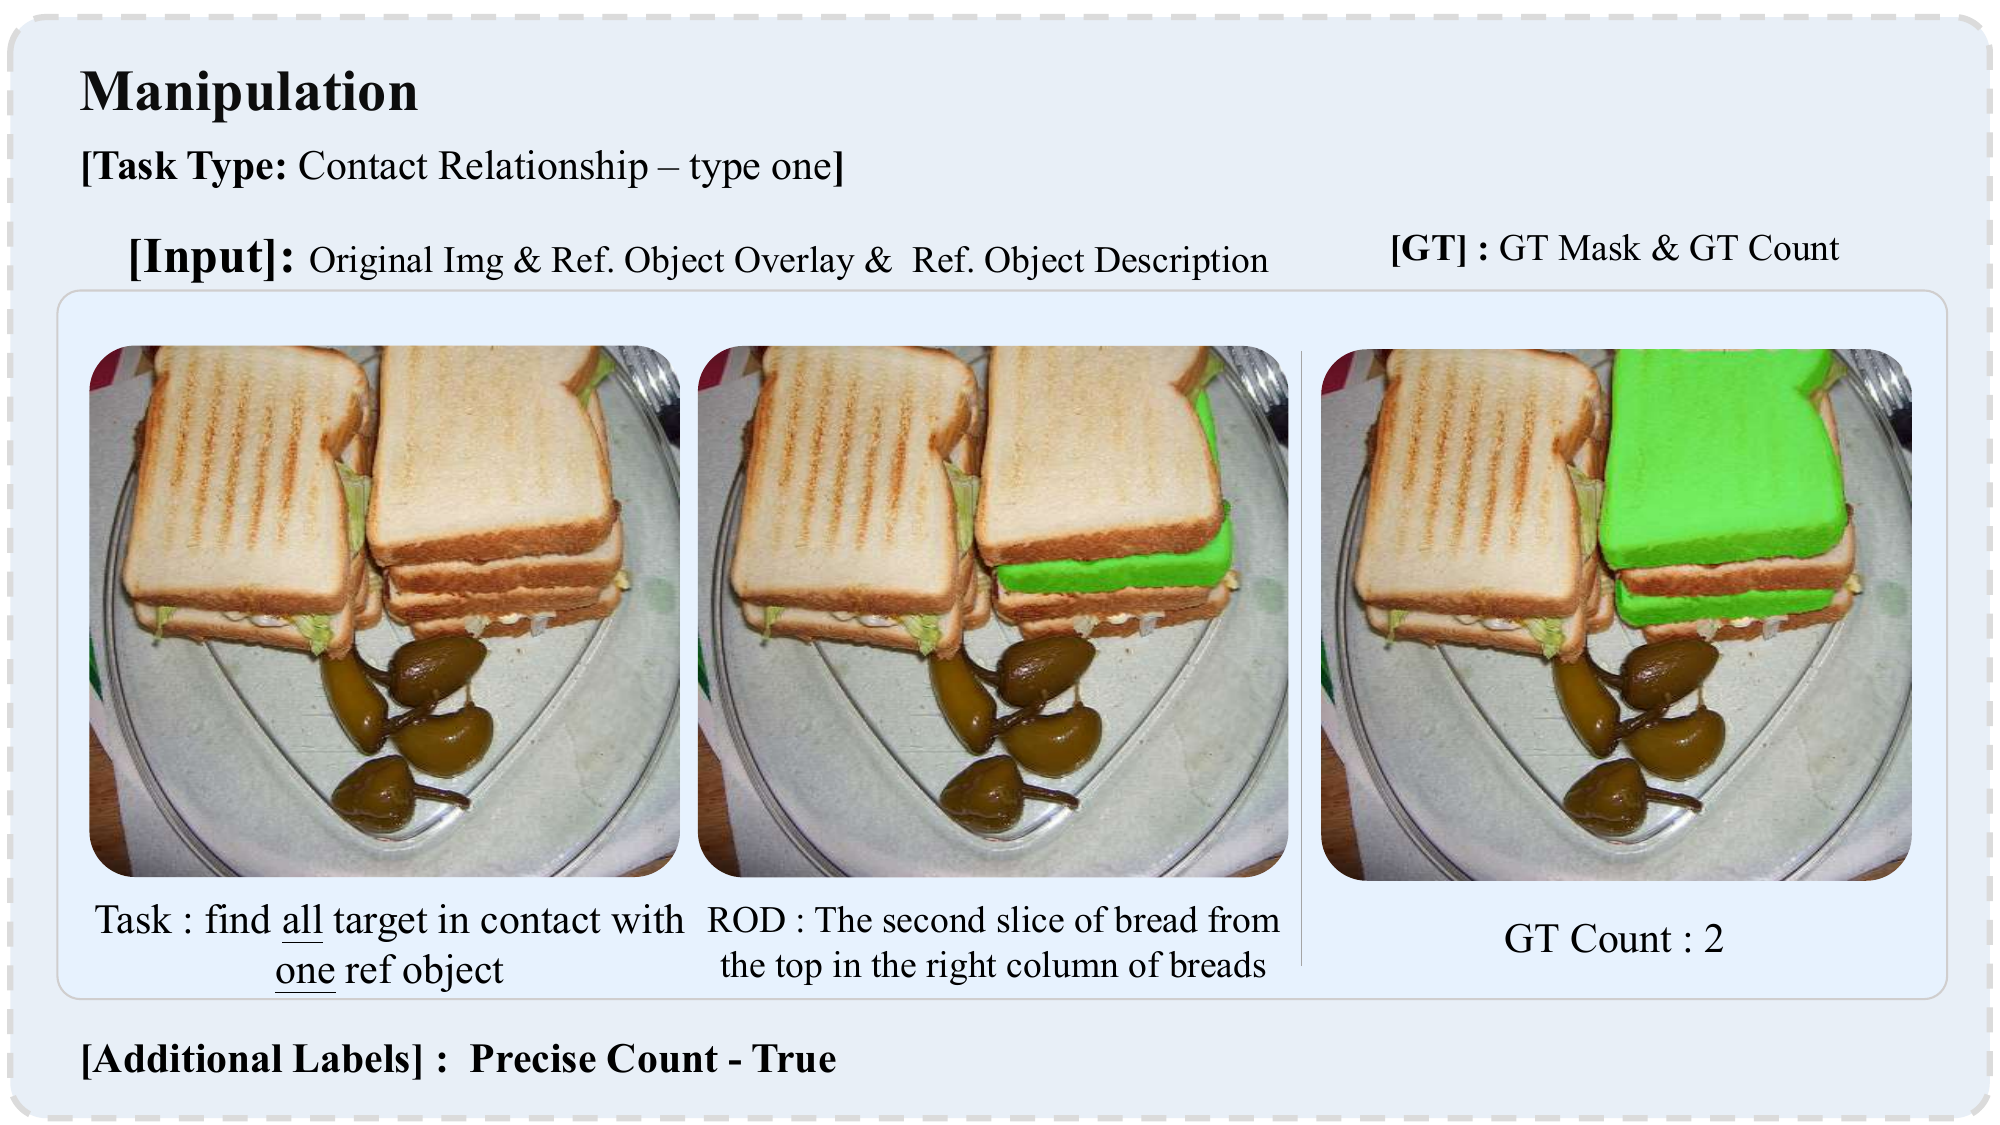}
\includegraphics[width=0.48\textwidth]{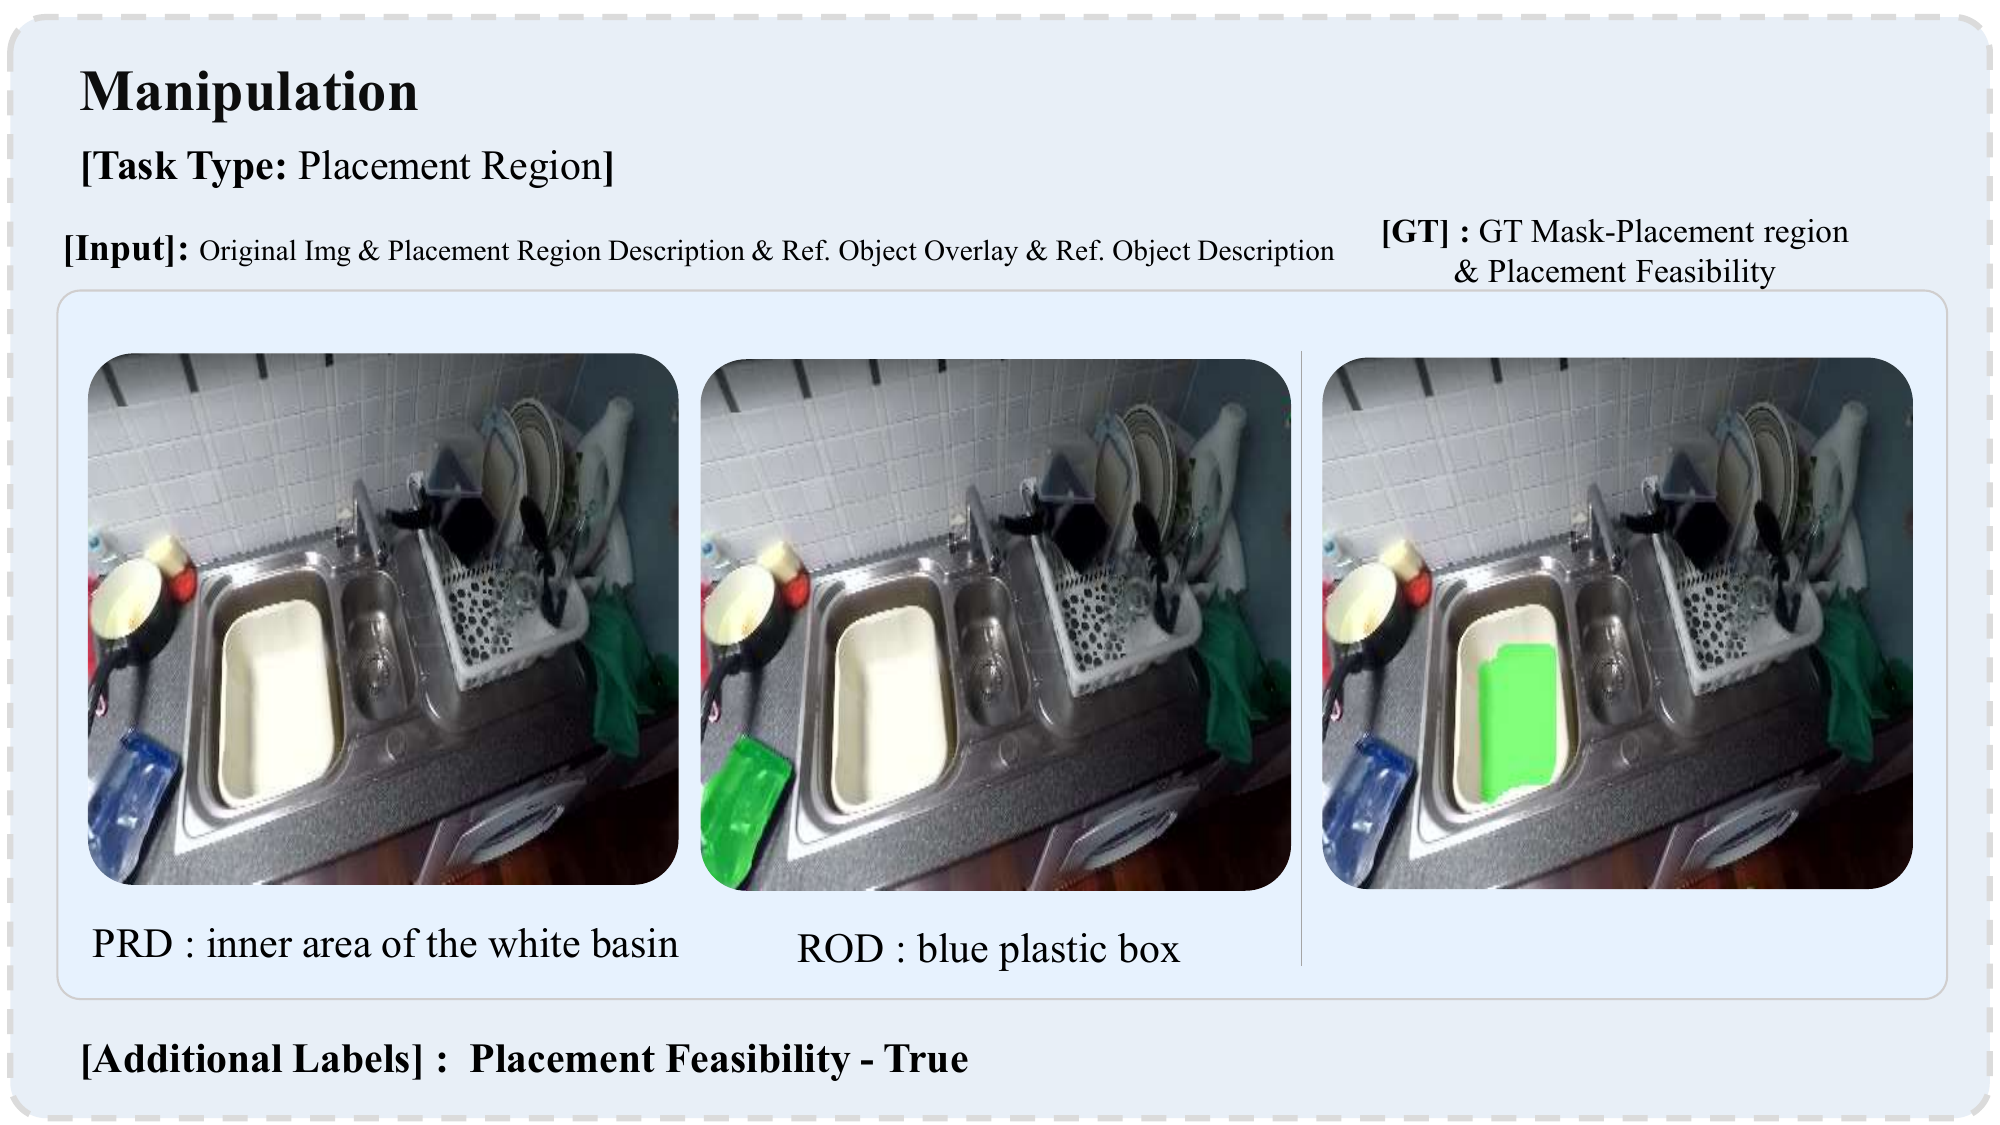}

\includegraphics[width=0.48\textwidth]{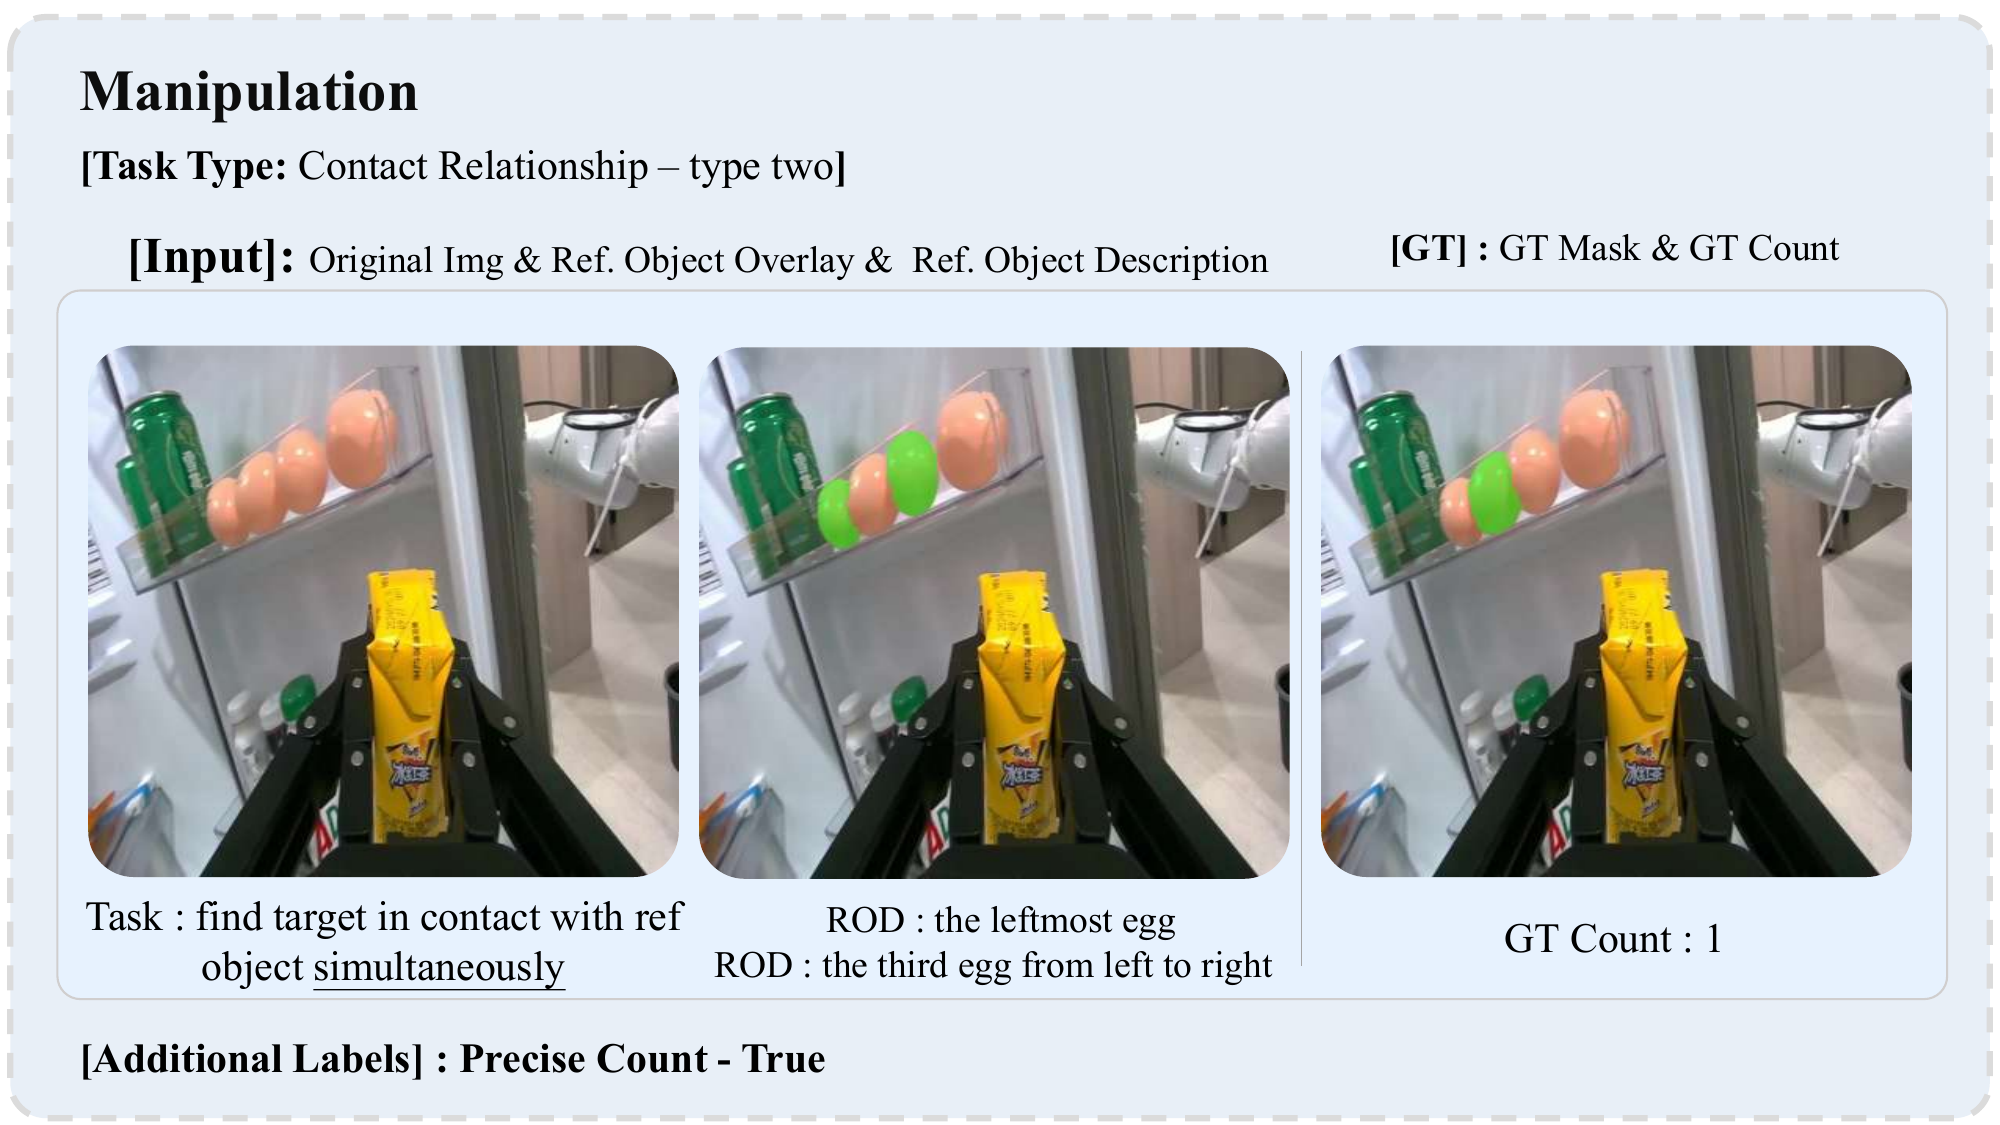}
\includegraphics[width=0.48\textwidth]{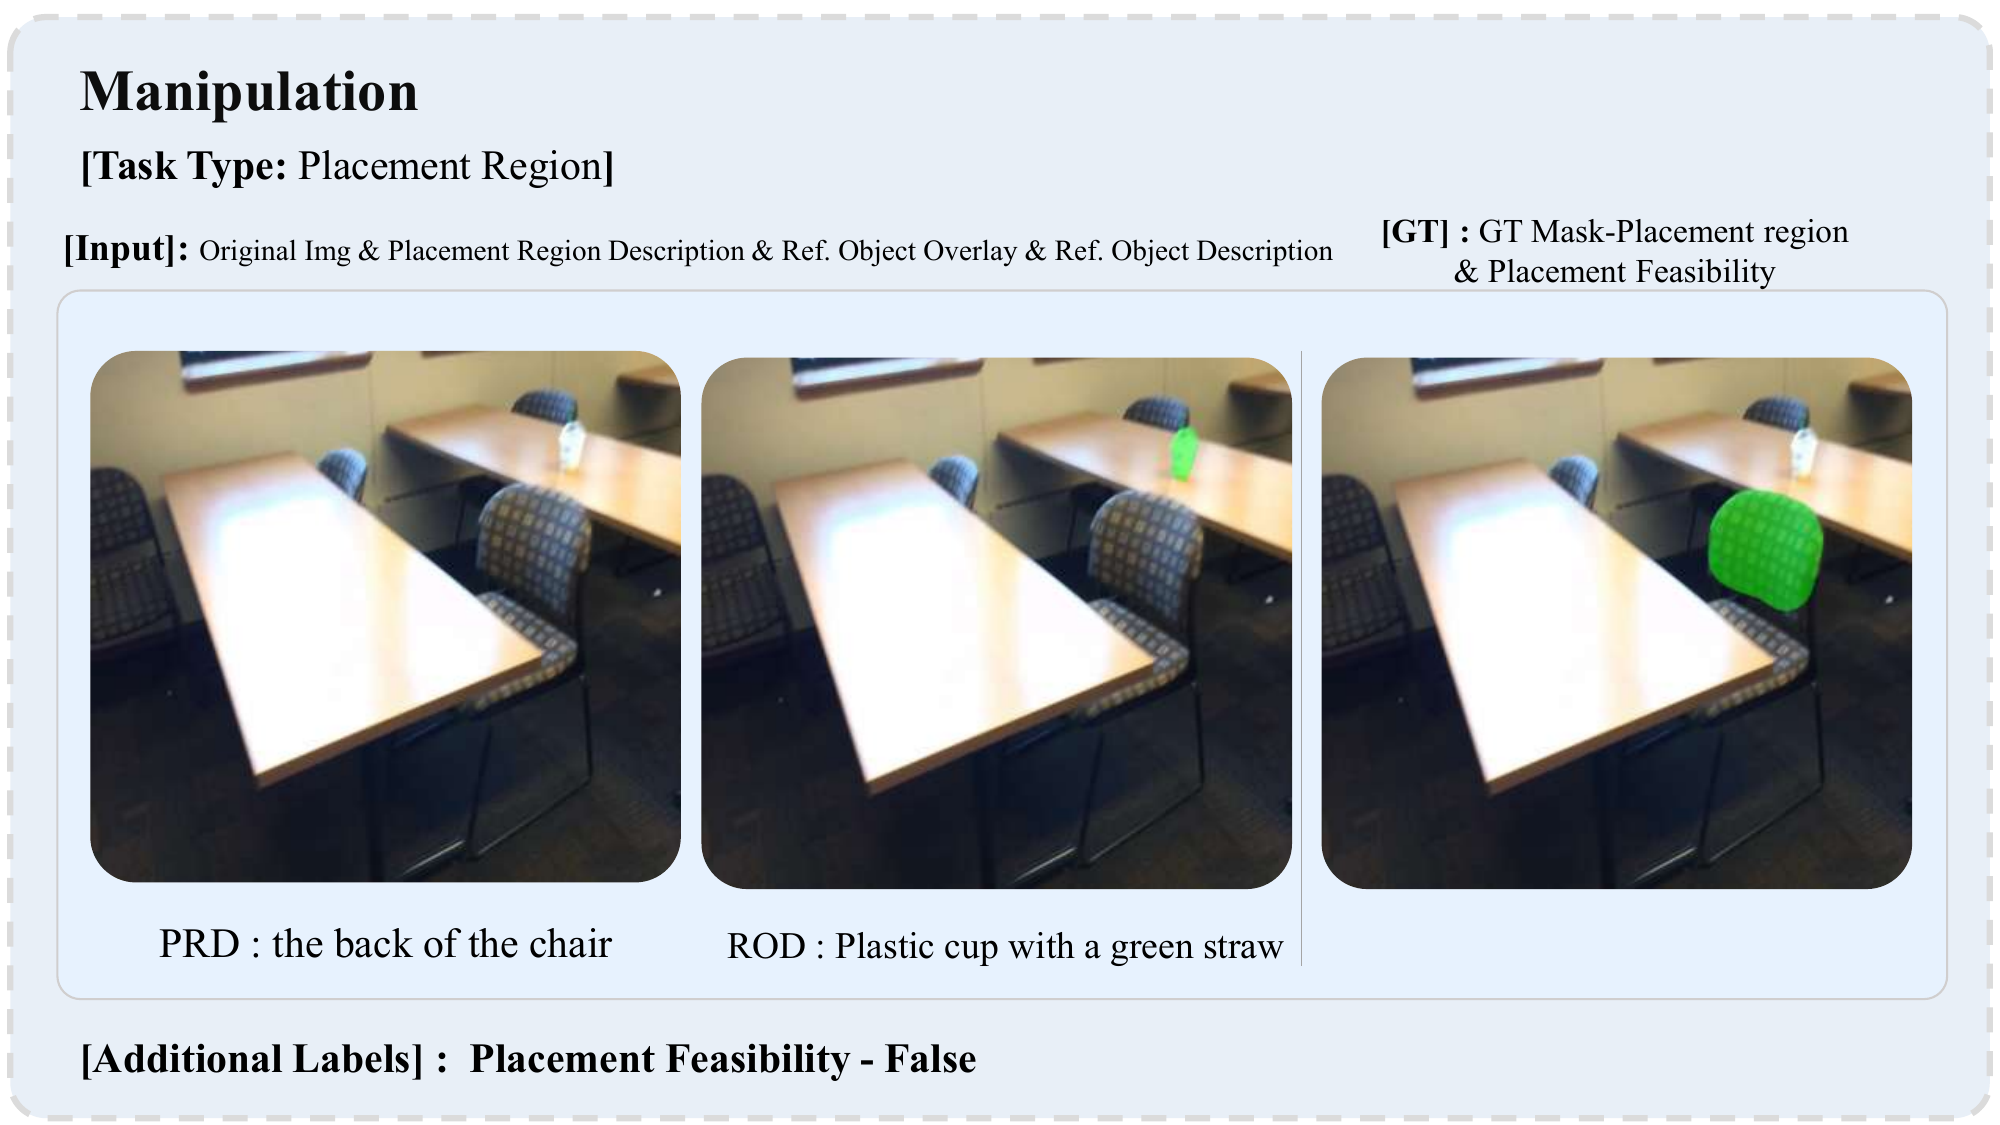}

\includegraphics[width=0.48\textwidth]{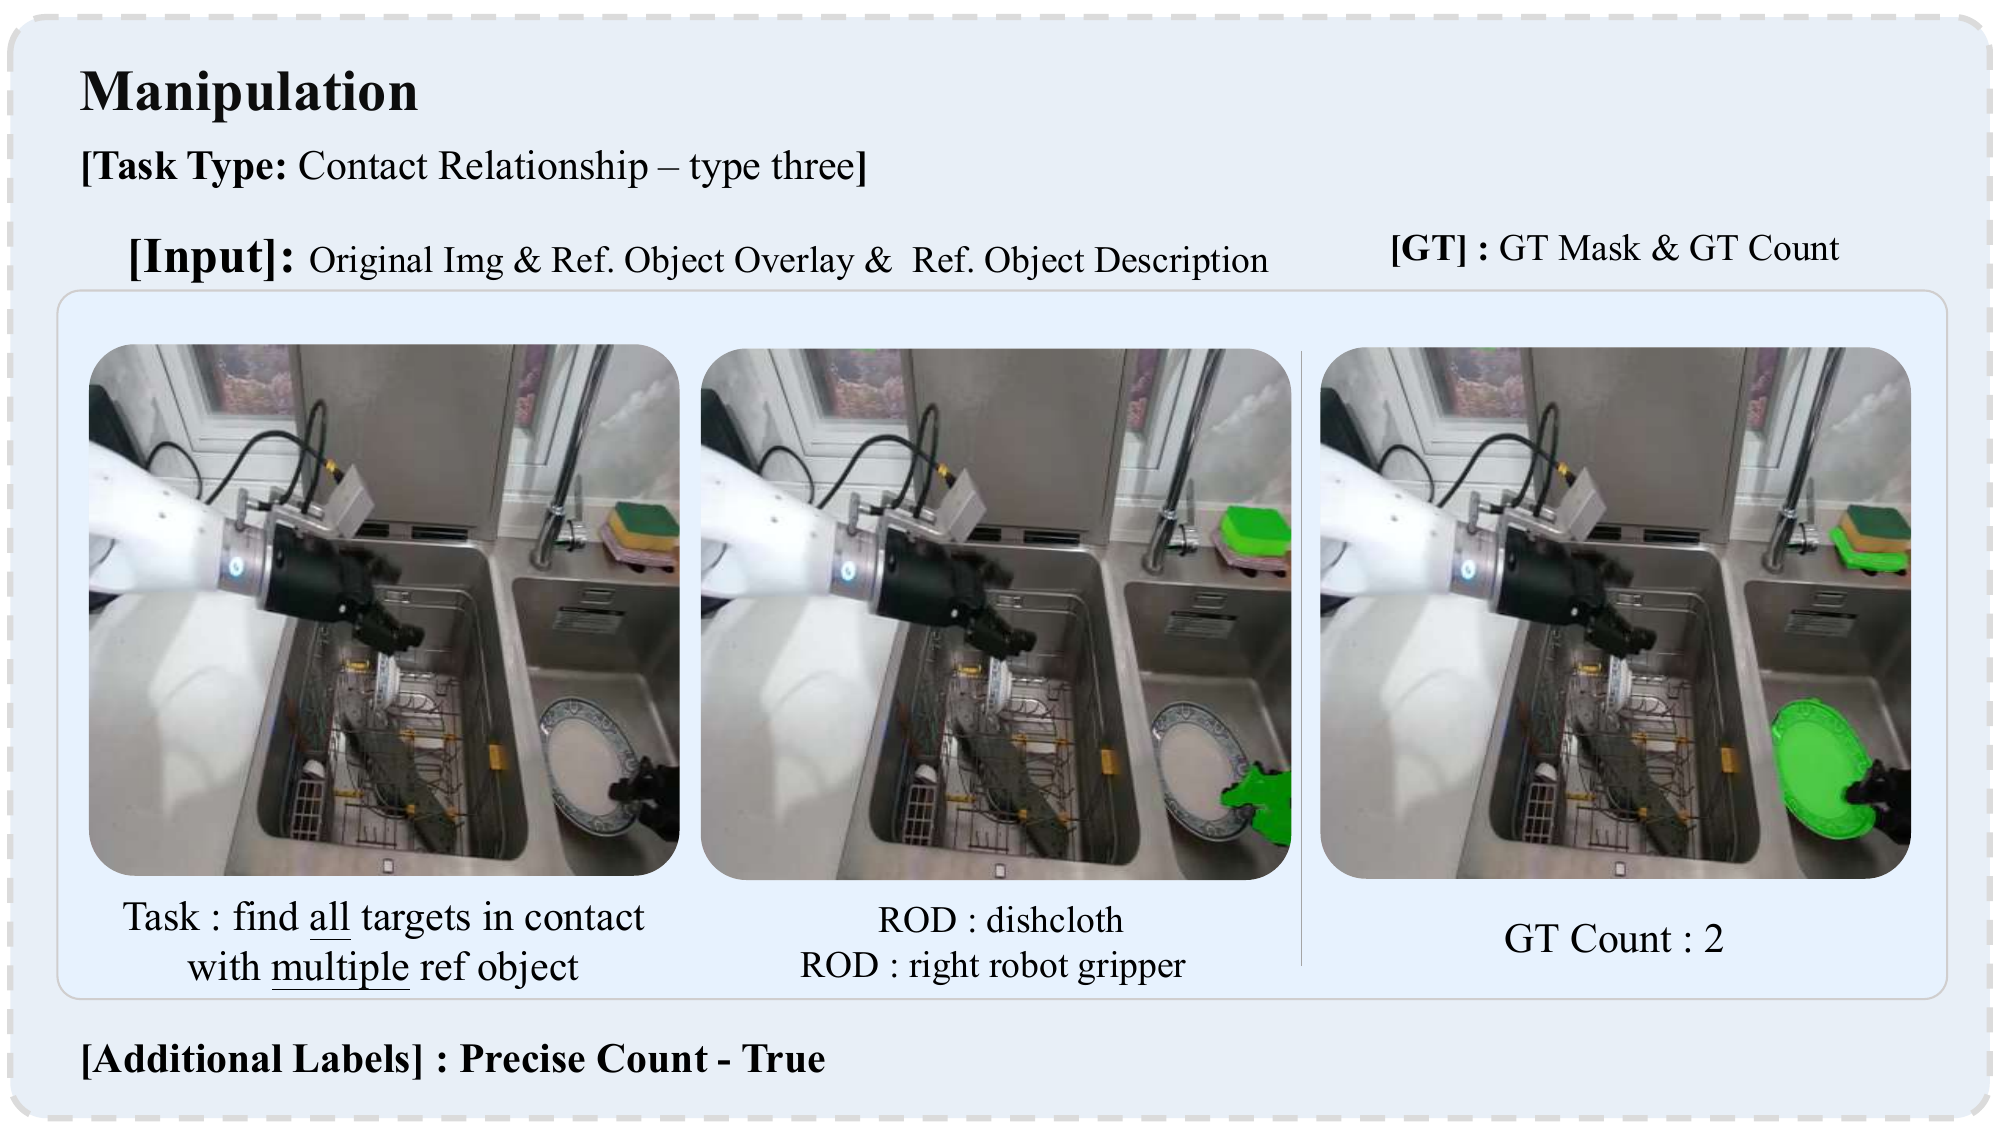}
\includegraphics[width=0.48\textwidth]{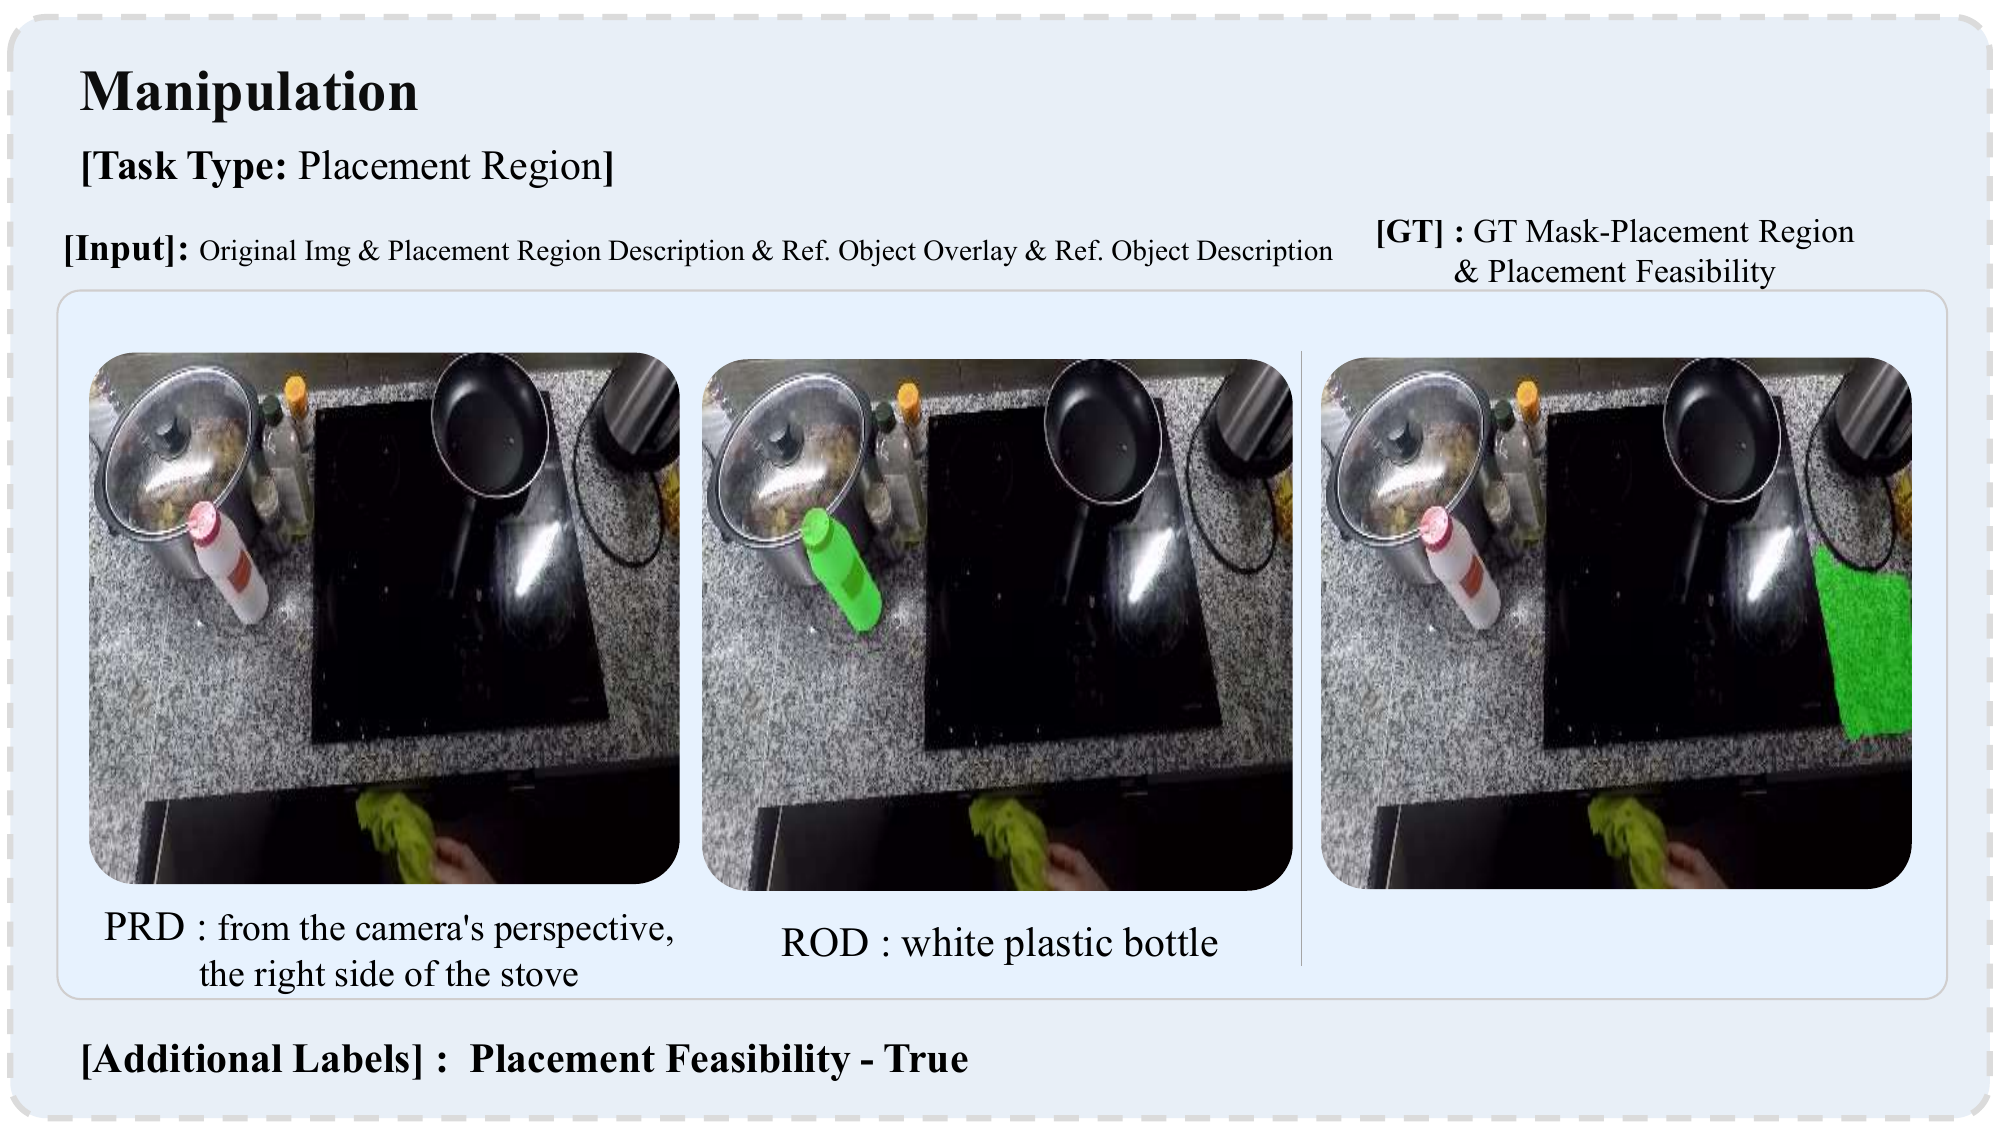}

\caption{Examples of Manipulation - Contact Relationship and Placement Region tasks}
\label{fig:example_MAN_CR_PR}
\end{figure*}




% \clearpage
\subsection{Data Sources}
\label{app:data_sources}
In this section, we provide a detailed summary of the source datasets used in EPIC-Bench. As shown in Table~\ref{tab:data_source}, we curate images from 20 publicly available datasets spanning four domains: general scenes, indoor environments, robotics, and egocentric views, thereby ensuring the diversity of our dataset.

We obtain all existing datasets from their original sources released by the authors. We refer readers to these sources for the dataset licenses.

\begin{table*}[th!]
\centering
% \begin{tabular}{l|l}
% \hline
% \textbf{Task} & \textbf{Dataset} \\
% \hline
\begin{tabular}{l|p{12cm}}
\hline
\textbf{Task} & \multicolumn{1}{c}{\textbf{Benchmark Dataset Source}} \\
\hline
General & Visual Genome \cite{Visual_genome}, GQA \cite{GQA}, ADE20K \cite{ade20k}, MSD \cite{MSD} \\
& RefCOCO \cite{refcoco}, OmniSpatial\cite{OmniSpatial},  LVIS \cite{LVIS}, CLEVR \cite{clevr}\\
\hline
Indoor & OpenSurfaces \cite{os_v3}, ARKitScenes \cite{arkitscenes}, ScanNet \cite{scanNet}, MP3D\cite{MP3D}, OCID \cite{OCID} \\
& 3RScan \cite{3RScan} \\
\hline
Robotic & Agibot-World \cite{agibotworld}, RoboVQA \cite{robovqa2023arxiv}, BridgeData V2 \cite{BridgeData}, RoboNet \cite{robonet} \\
\hline
Egocentric & EPIC-KITCHENS \cite{epic-kitchens}, RoboVQA \cite{robovqa2023arxiv}\\
& HOVA-500K \cite{HOVA-500K}, EGTEA Gaze+ \cite{EGTEA} \\
\hline
\end{tabular}
\caption{Dataset source summary in EPIC-Bench.}
\label{tab:data_source}
\end{table*}

%  HICO \cite{HICO},   HoloAssit \cite{HoloAssit},      HOI4D \cite{HOI4D}






\subsection{Quality Control Details}

We employ 20 human annotators with undergraduate-level education, contributing over 4,800 person-hours across 30 working days. Annotators are initially assigned to different task categories, and all annotations undergo at least two rounds of cross-checking. The revision rates after the first and second rounds are 15\% and 6\%, respectively.

We explicitly identify and revise ambiguous or shortcut-prone samples. For example, as shown in Fig.~\ref{fig:data_collection_pipeline}, the description \textit{the first shelf of the bookcase} is ambiguous because \textit{first} may refer to either the top or bottom shelf; we therefore revise it to \textit{the top shelf} according to the annotated target. Another sample with the description \textit{the person on the ice} is considered overly simple because both people in the image are on the ice, allowing the target to be identified from the category cue alone without understanding the spatial relation \textit{on the ice}. Such samples are revised or removed. For samples with target-count labels, a second annotator independently verifies the number of targets using only the image and text. In cases of disagreement, we revise the count, set \texttt{precise\_count} to false, or remove the sample. Similarly, when an image contains multiple objects of the same category with different sizes, we avoid ambiguous descriptions such as \textit{the bigger objects} and instead specify the target count, e.g., \textit{the two larger objects}.

For tasks involving subjective spatial or interaction judgments, the ground truth is defined according to the region that a human would most likely traverse or interact with when executing the instruction. For example, for ``pick up the cup,'' the annotated affordance region typically covers the handle or central body rather than the rim, although grasping the rim may occasionally be feasible. These annotations are further validated through cross-checking to improve consistency.




\section{Evaluatioin Details}

\subsection{Prompt Templates and Prompt Robustness}
\label{app:prompts}
\subsubsection{Prompt Details}
\paragraph{Task Prompt} we present the prompt templates for each sub-task. We design task-specific prompts for the categories of Target Localization (shown in Figure~\ref{fig:TL}), Navigation (Ground Detection, Feasible Path, Visual Matching) (shown in Figure~\ref{fig:nav}), and Manipulation (Affordance Region, Contact Relationship, Placement Region) categories (shown in Figure~\ref{fig:man}).




\begin{figure*}[t]
  \centering
  \includegraphics[width=\textwidth]{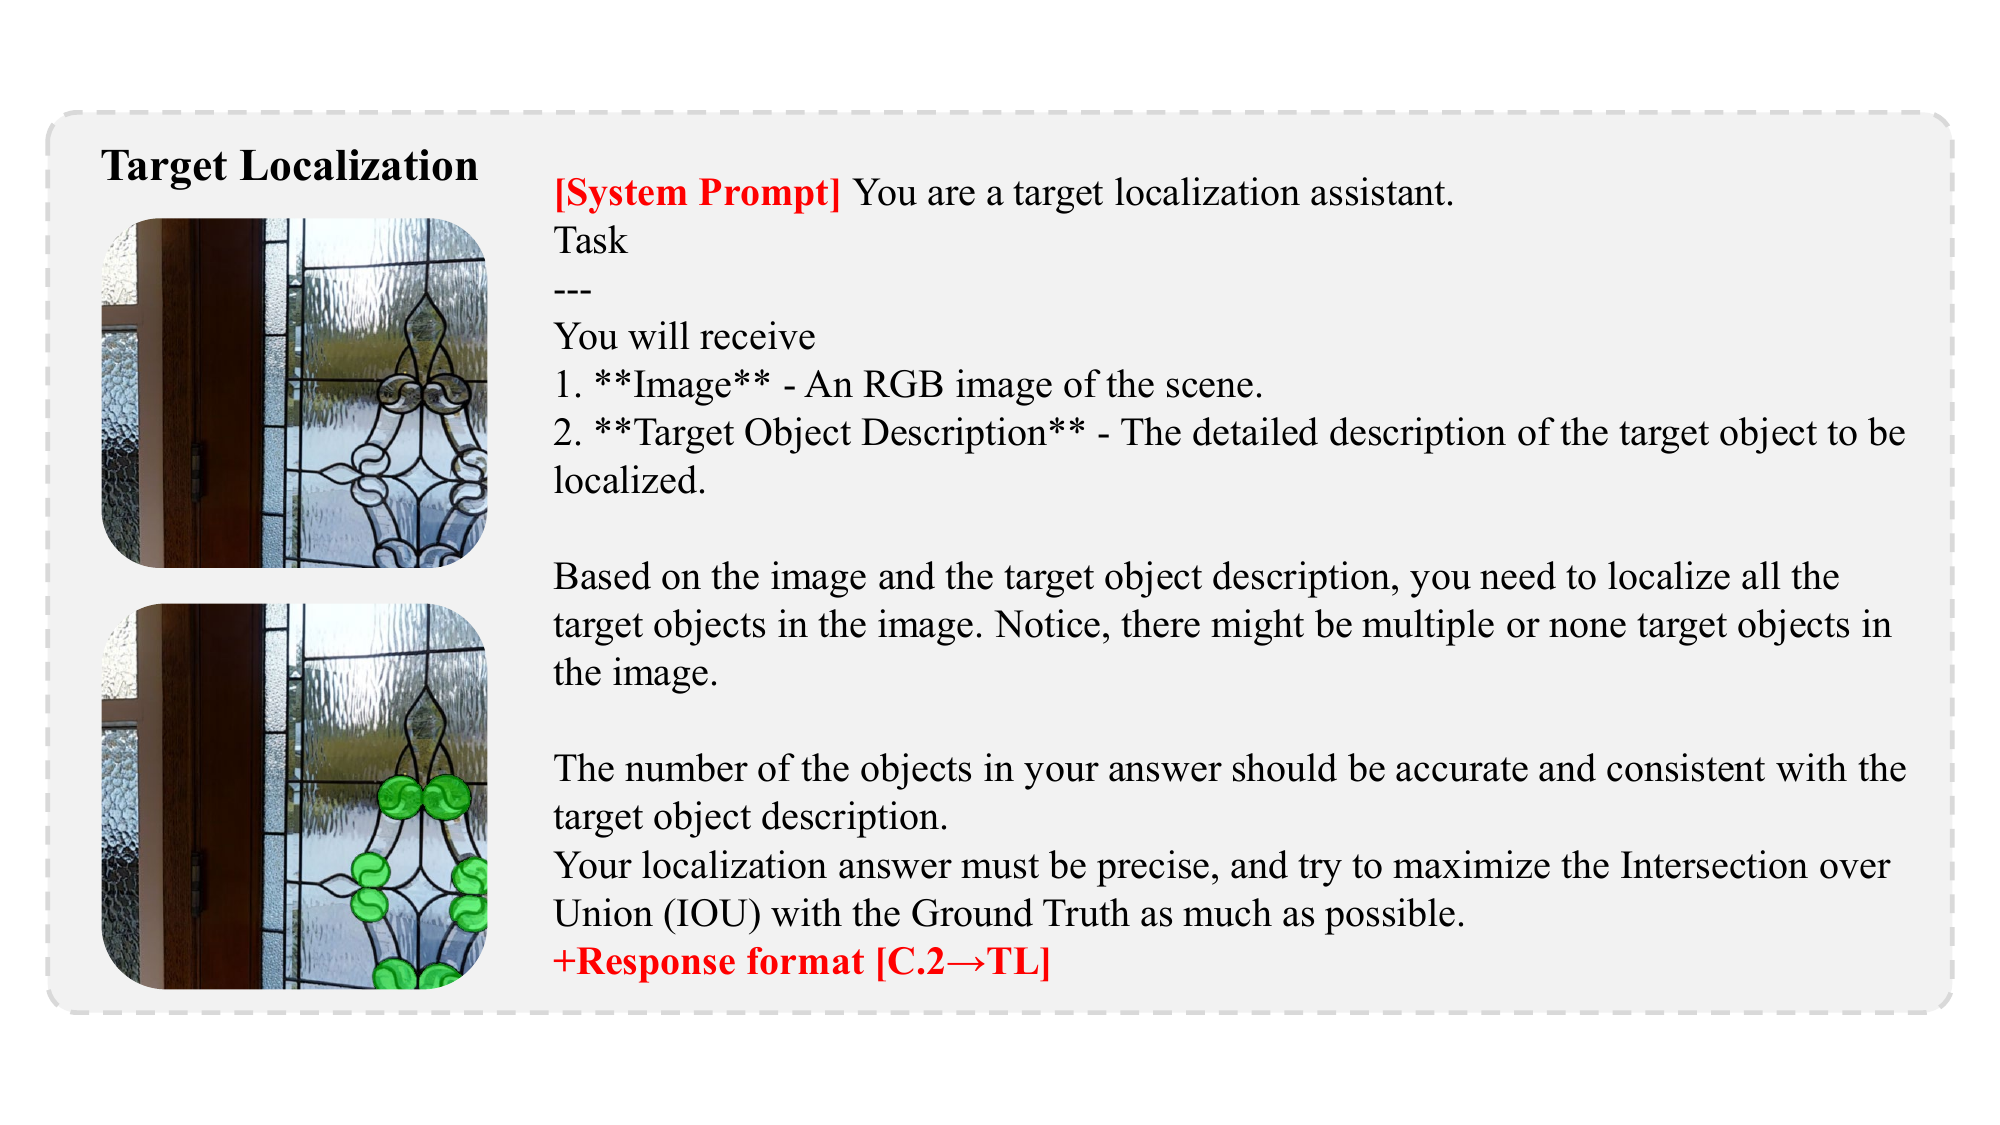}
    \caption{\textbf{Prompt for Target Localization.} Target Localization requires the model to identify all target objects matching the textual description.}
  \label{fig:TL}
\end{figure*}




% \begin{table}[th!]
% \centering
% \caption{Dataset source summary in Epic-Bench.}
% \label{tab: data_source}
% % \begin{tabular}{l|l}
% % \hline
% % \textbf{Task} & \textbf{Dataset} \\
% % \hline
% \begin{tabular}{l|l}
% \hline
% \textbf{Task} & \multicolumn{1}{c}{\textbf{Benchmark Dataset Source}} \\
% \hline
% General & HICO \cite{HICO}, Visual Genome \cite{Visual_genome}, GQA \cite{GQA}, ADE20K \cite{ade20k}, MSD \cite{MSD} \\
% & RefCOCO \cite{refcoco}, OmniSpatial\cite{OmniSpatial},  LVIS \cite{LVIS}, CLEVR \cite{clevr}\\
% \hline
% Indoor & OpenSurfaces \cite{os_v3}, ARKitScenes \cite{arkitscenes}, ScanNet \cite{scanNet}, MP3D\cite{MP3D}, OCID \cite{OCID} \\
% & 3RScan \cite{3RScan}, Charades \cite{Charades} \\
% \hline
% Robotic & Agibot-World \cite{agibotworld}, RoboVQA \cite{robovqa2023arxiv}, BridgeData V2 \cite{BridgeData}, RoboNet \cite{robonet} \\
% \hline
% Egocentric & EPIC-KITCHENS \cite{epic-kitchens}, HoloAssit \cite{HoloAssit}, RoboVQA \cite{robovqa2023arxiv}, Charades \cite{Charades}\\
% & HOVA-500K \cite{HOVA-500K}, EGTEA Gaze+ \cite{EGTEA}, HOI4D \cite{HOI4D} \\
% \hline
% \end{tabular}
% \end{table}

% \begin{figure}[b]
%   \centering
%   \includegraphics[width=\textwidth]{Graphics/Appendix_C_prompts/TL.pdf}
%     \caption{\textbf{Prompt for Target Localization.} Target Localization requires the model to identify all target objects matching the textual description.}
%   \label{fig:TL}
% \end{figure}





\begin{figure*}[t]
  \centering
  \includegraphics[width=0.9\textwidth]{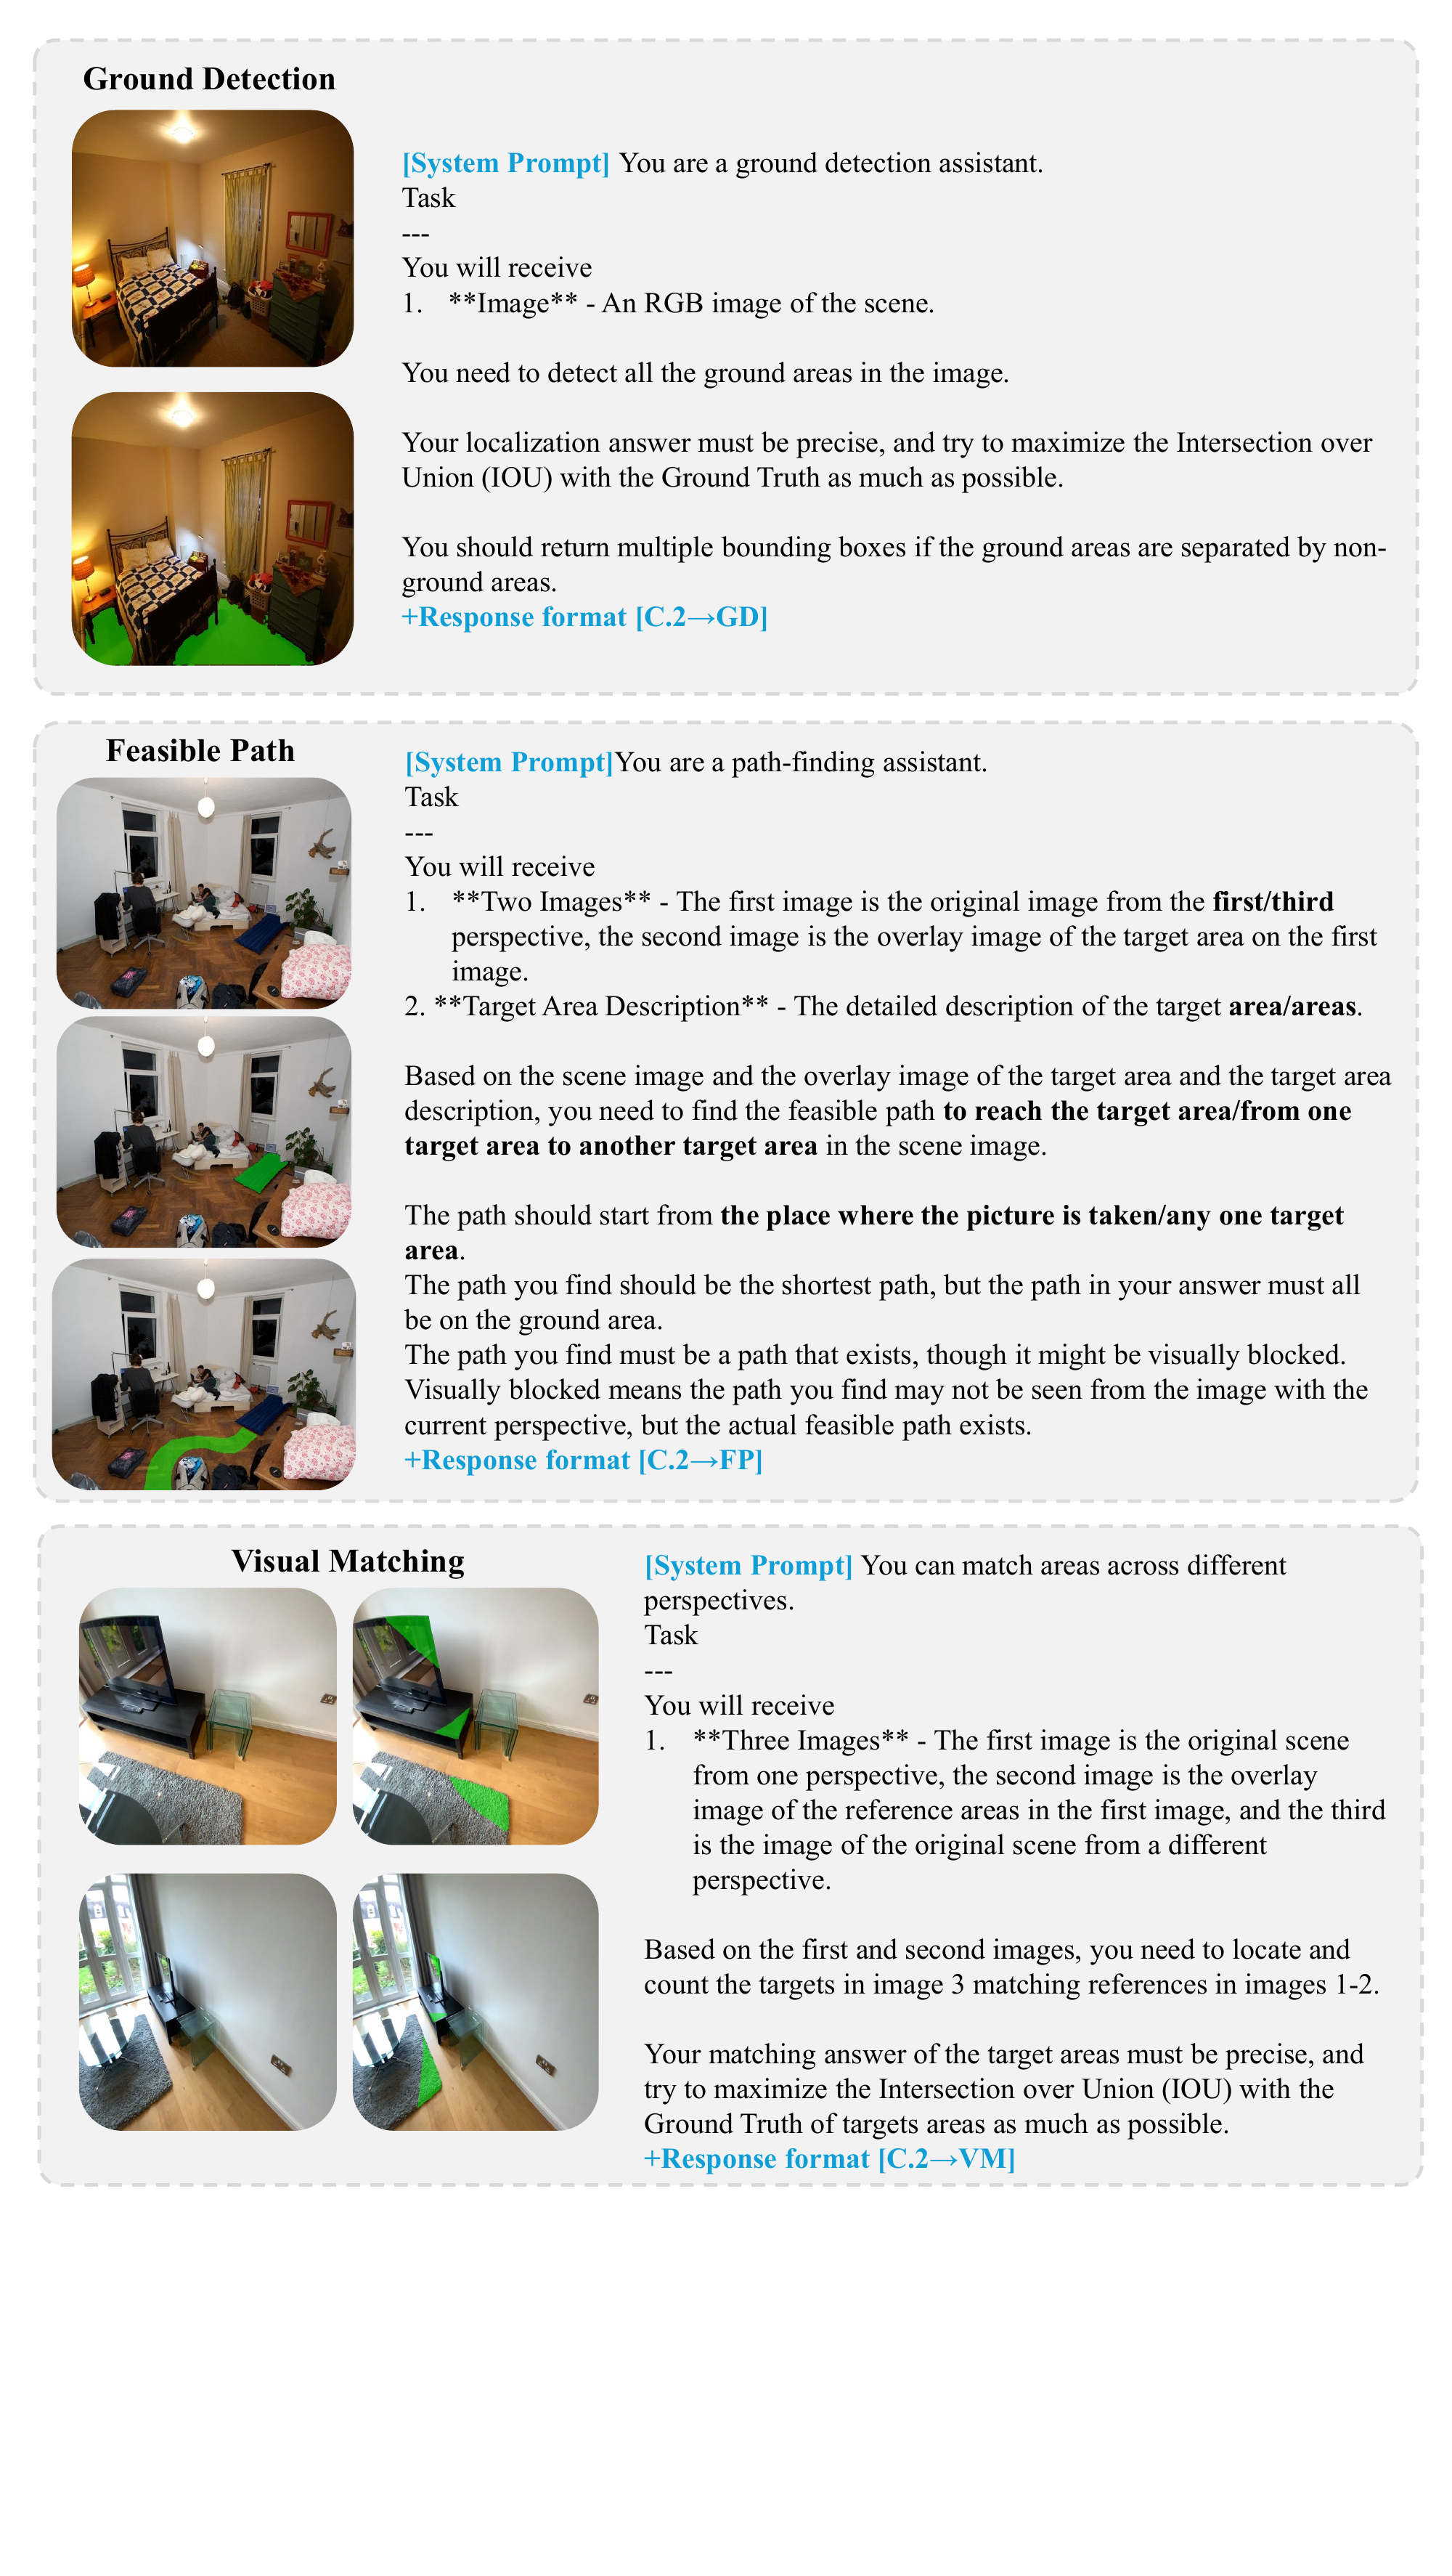}
    \caption{\textbf{Prompts for Navigation.} Navigation category includes three sub-tasks: Ground Detection (identifying traversable ground regions), Feasible Path (planning routes to target objects in egocentric view or between two targets in exocentric view), and Visual Matching (localizing the same reference area across different viewpoints).}
  \label{fig:nav}
\end{figure*}

\begin{figure*}[t]
  \centering
  \includegraphics[width=0.8\textwidth]{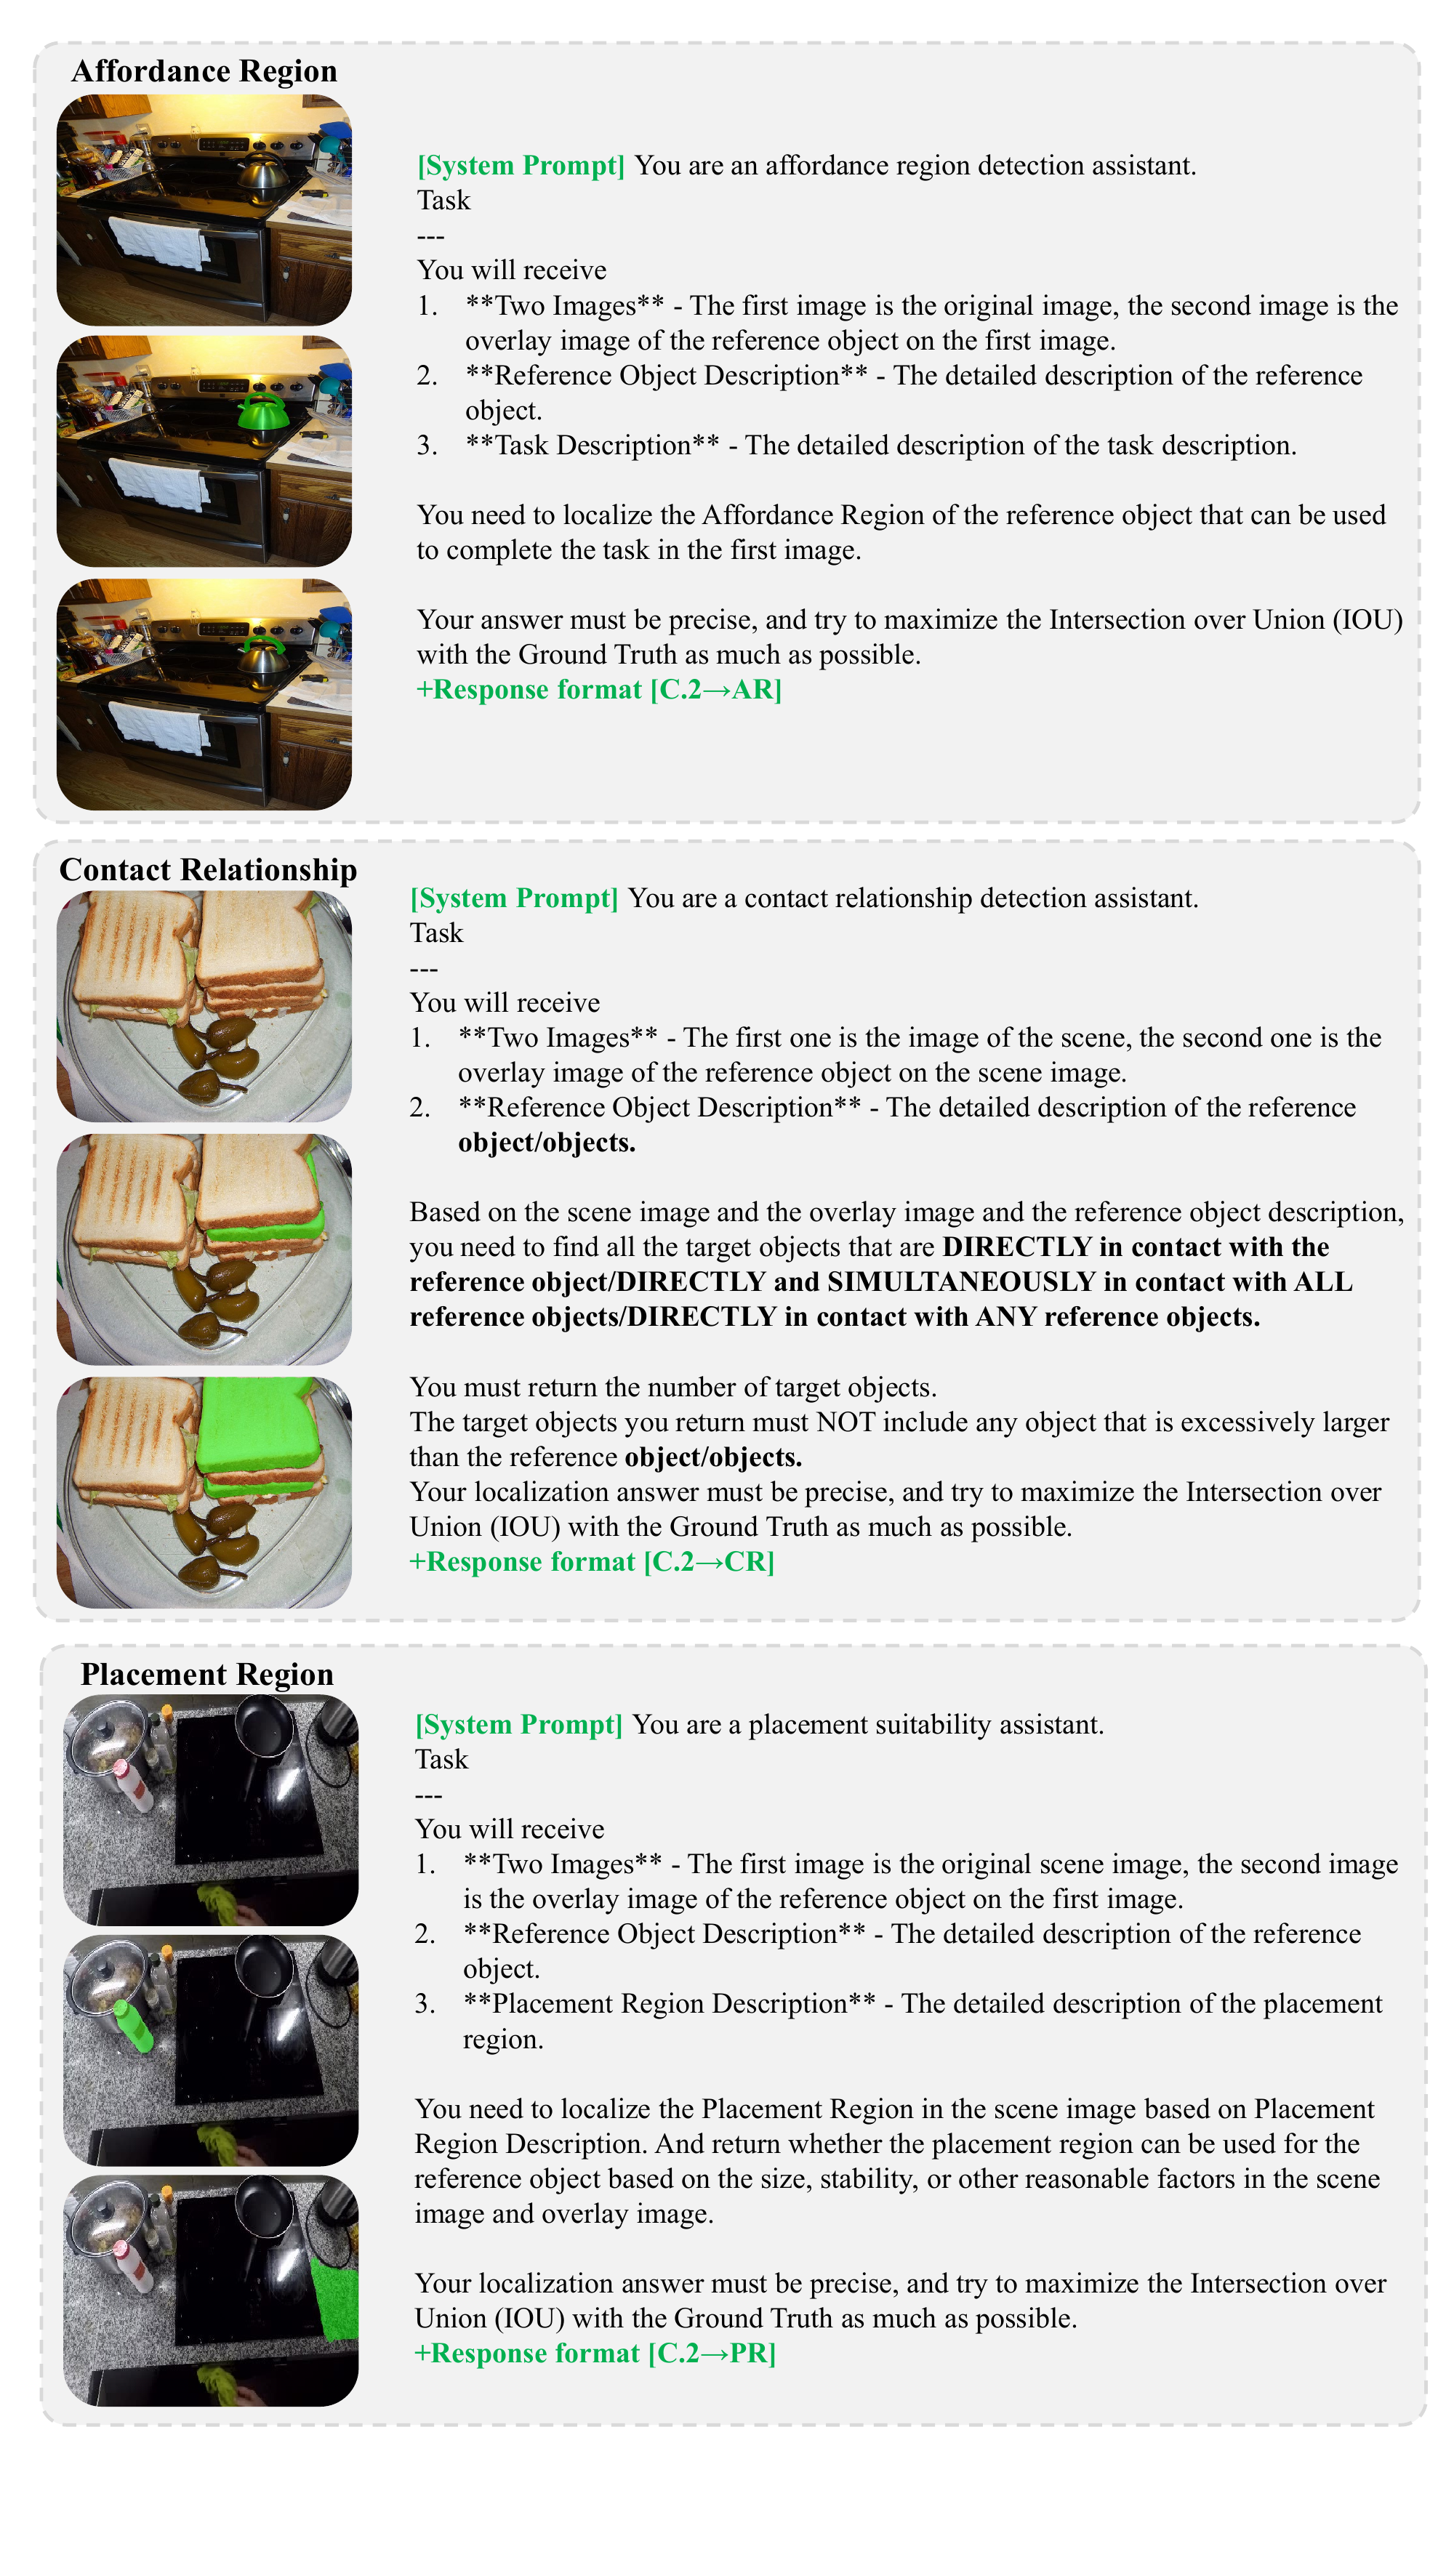}
    \caption{\textbf{Prompts for Manipulation.} Affordance Region (localizing operable regions of a reference object), Contact Relationship (identifying objects in contact with single/multiple reference objects under three contact conditions), and Placement Region (localizing placement areas and determining placement feasibility).}
  \label{fig:man}
\end{figure*}



\paragraph{Response Format.}
As illustrated in Figure~\ref{fig:response_format}, we require models to return predictions in a structured JSON format for consistent evaluation. The grounding representation itself follows the format natively supported by each model: conventional VLMs typically predict bounding-box coordinates, while models with pixel-level grounding capabilities may directly output masks. We further implement a robust answer-extraction procedure that tolerates minor formatting errors in raw responses, such as mismatched brackets or extra spaces. Since different models may use absolute coordinates, normalized coordinates, or coordinates scaled to the 0--1000 range, our parser explicitly handles these variations.




\begin{figure*}[htbp]
  \centering
  \includegraphics[width=\textwidth]{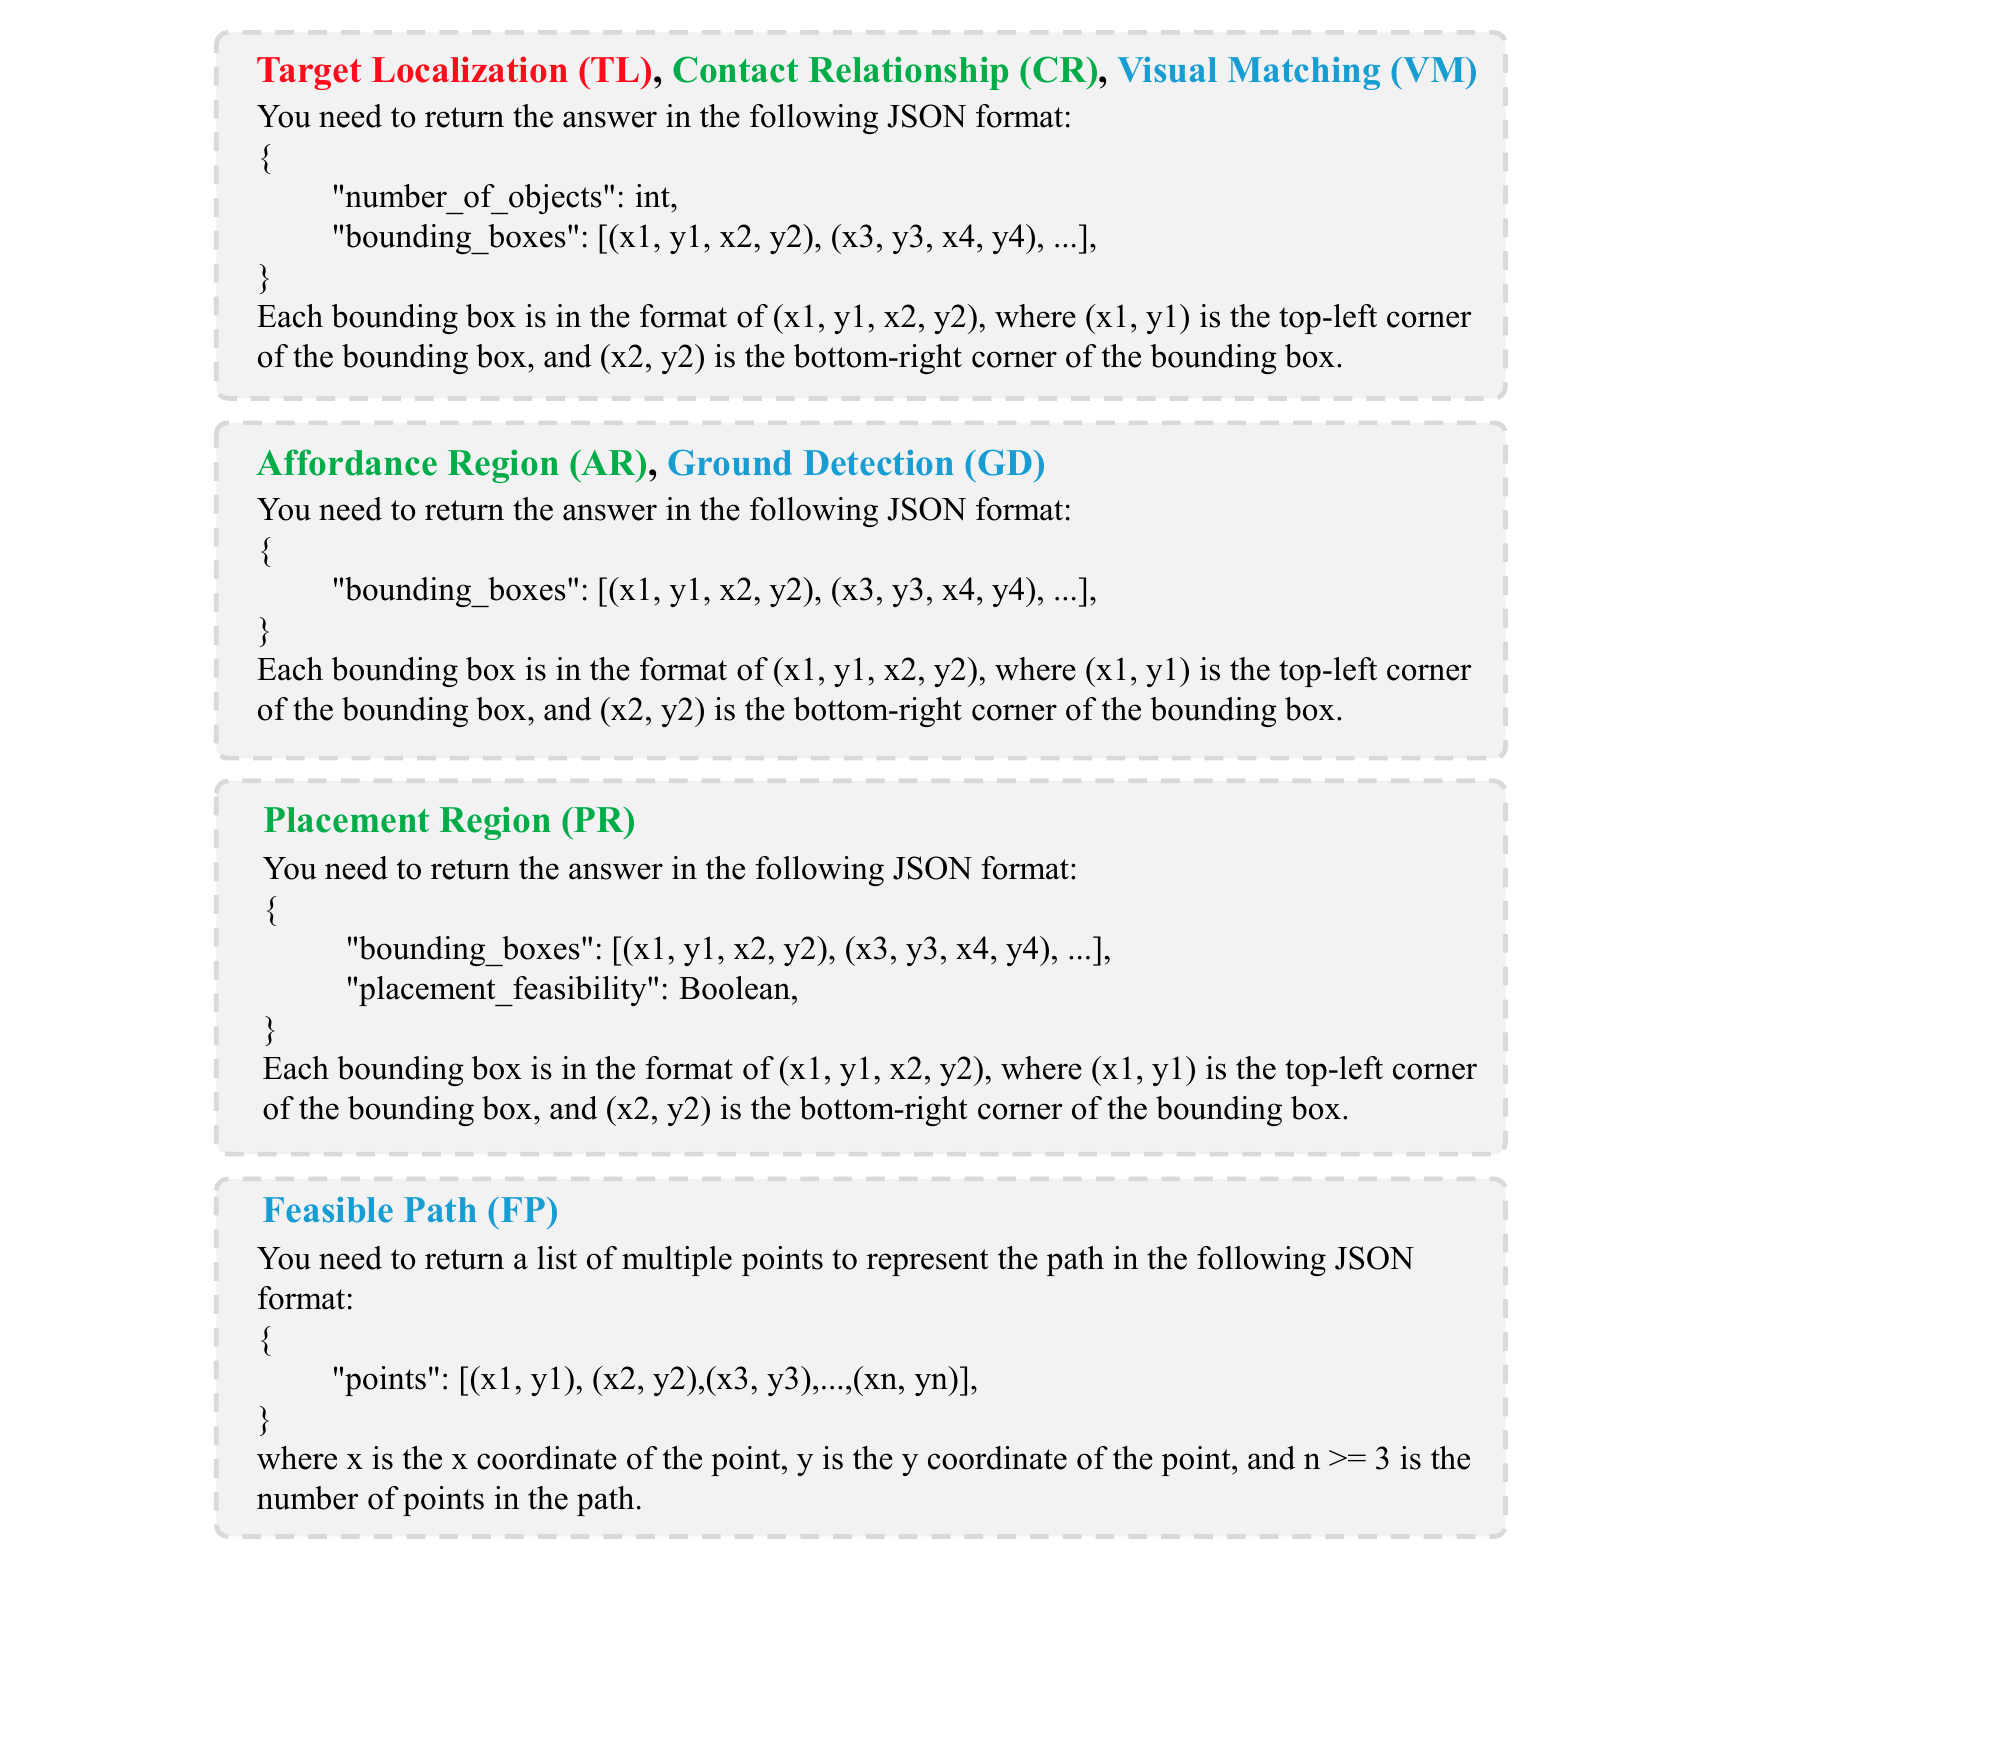}
\caption{\textbf{Response format for each sub-task.} For \textbf{Target Localization (TL)}, \textbf{Contact Relationship (CR)}, and \textbf{Visual Matching (VM)}, models are required to output bounding boxes and the count of target objects. \textbf{Affordance Region (AR)} and \textbf{Ground Detection (GD)}, models are required to output the corresponding bounding boxes. For \textbf{Placement Region (PR)}, models are required to output the placement region bounding box along with a binary judgment on placement feasibility. For \textbf{Feasible Path (FP)}, models are required to output a sequence of points representing the path.}
\label{fig:response_format}
\end{figure*}


\subsubsection{Prompt Robustness}

We further evaluate the robustness of EPIC-Bench evaluation to prompt variations. We randomly sample 40 examples from each of the 23 subtasks, resulting in 920 examples, and evaluate 11 representative models under three prompting strategies: (1) the base task prompt containing the task description, (2) a simple CoT prompt additionally instructing the model to ``think step by step'', and (3) a complex CoT prompt with manually designed reasoning instructions.

\begin{table}[t]
\centering
\small
\resizebox{\columnwidth}{!}{
\begin{tabular}{lccc}
\toprule
\textbf{Model} & \textbf{Base} & \textbf{Simple CoT} & \textbf{Complex CoT} \\
\midrule
GPT-5.5                     & 54.10 & 53.67 & 54.11 \\
Gemini-3-Pro-Preview        & 53.44 & 56.12 & 56.16 \\
Doubao-Seed-1.8             & 50.38 & 50.54 & 50.49 \\
Qwen3-VL-30B-A3B-Thinking   & 45.49 & 45.63 & 46.34 \\
GLM-4.6V                    & 41.20 & 40.97 & 41.61 \\
InternVL3.5-241B-A28B       & 41.03 & 41.59 & 41.77 \\
RoboBrain2.0-32B            & 39.78 & 38.46 & 39.81 \\
Pelican1.0-VL-72B           & 35.75 & 24.41 & 34.71 \\
Gemma-3-27B-IT              & 28.52 & 28.23 & 29.63 \\
Cosmos-Reason1-7B           & 22.97 & 22.18 & 21.31 \\
LLaVA-NeXT-72B              & 22.55 & 22.24 & 21.95 \\
\midrule
\textbf{Average}            & \textbf{39.56} & \textbf{38.55} & \textbf{39.81} \\
\bottomrule
\end{tabular}
}
\caption{Performance under different prompting strategies.}
\label{tab:cot_prompt}
\end{table}

As shown in Table~\ref{tab:cot_prompt}, the average scores vary only slightly across the three prompting strategies, indicating that the benchmark results are generally robust to these prompt variations.

Since VLMs deployed as embodied agents are expected to possess general instruction-following capabilities, EPIC-Bench does not require a fixed prompt template. Developers may adapt the prompt format as long as the task semantics remain consistent with the benchmark definition.






\subsection{Post-Processing Strategies}

EPIC-Bench provides its ground-truth annotations in mask format. Our main evaluation is based on the models' original grounding predictions. For models that natively produce irregular mask outputs, we directly compute IoU between the predicted and ground-truth masks. For models whose grounding outputs are primarily represented as bounding boxes, we convert each predicted box into the corresponding mask before computing IoU. This preserves the spatial region directly predicted by the model.

We further analyze the effect of applying an external segmentation model to the original predictions. Specifically, we use SAM3 to extract the mask of the most salient object or region within each predicted bounding box region. We compare the overall score, per-sample win/loss/tie statistics, and IoU before and after SAM3-based post-processing. A sample is counted as a win or loss when the absolute score change exceeds 0.01; otherwise, it is counted as a tie.

\begin{table*}[t]
\centering
\small
\resizebox{\textwidth}{!}{
\begin{tabular}{lccccccccc}
\toprule
\textbf{Model} &
\textbf{Score (BBox)} &
\textbf{Score (SAM3)} &
$\boldsymbol{\Delta}$\textbf{Score} &
\textbf{Win (\%)} &
\textbf{Loss (\%)} &
\textbf{Tie (\%)} &
\textbf{IoU (BBox)} &
\textbf{IoU (SAM3)} &
$\boldsymbol{\Delta}$\textbf{IoU} \\
\midrule
Gemini-3-Pro                     & 53.85 & 63.28 &  9.42 & 61.79 & 15.55 & 22.65 & 0.404 & 0.569 &  0.165 \\
Qwen3-VL-235B-A22B-Thinking      & 50.23 & 57.54 &  7.32 & 56.63 & 23.71 & 19.67 & 0.391 & 0.513 &  0.123 \\
GPT-5.5                          & 51.72 & 57.78 &  6.06 & 53.18 & 25.22 & 21.60 & 0.375 & 0.481 &  0.106 \\
GLM-4.6V                         & 42.07 & 46.69 &  4.61 & 42.34 & 24.67 & 33.00 & 0.285 & 0.360 &  0.075 \\
Doubao-Seed-1.8                  & 46.53 & 51.11 &  4.58 & 40.52 & 25.49 & 33.99 & 0.301 & 0.374 &  0.073 \\
InternVL3.5-241B-A28B            & 40.30 & 44.34 &  4.03 & 39.68 & 23.45 & 36.87 & 0.307 & 0.379 &  0.073 \\
RoboBrain2-32B                   & 39.40 & 40.90 &  1.49 & 35.52 & 32.66 & 31.82 & 0.307 & 0.336 &  0.028 \\
Cosmos-Reason1-7B                & 26.26 & 26.25 & -0.01 & 23.33 & 34.05 & 42.62 & 0.167 & 0.167 &  0.000 \\
LLaVA-NeXT-72B                   & 24.42 & 23.71 & -0.71 & 23.68 & 40.05 & 36.27 & 0.148 & 0.137 & -0.011 \\
Gemma-3-27B-IT                   & 26.68 & 25.08 & -1.61 &  6.64 & 36.27 & 57.09 & 0.058 & 0.030 & -0.028 \\
Pelican1.0-VL-72B                & 36.10 & 32.64 & -3.46 & 10.04 & 50.46 & 39.50 & 0.221 & 0.161 & -0.060 \\
\midrule
\textbf{Average}                 & \textbf{39.78} & \textbf{42.66} & \textbf{2.88} &
\textbf{35.76} & \textbf{30.14} & \textbf{34.10} &
\textbf{0.269} & \textbf{0.319} & \textbf{0.049} \\
\bottomrule
\end{tabular}
}
\caption{Effect of SAM3-based post-processing on grounding evaluation. BBox denotes evaluation using the original bounding-box region mask predictions, while SAM3 denotes evaluation after converting each predicted region into a salient-object mask using SAM3.}
\label{tab:sam3_postprocess}
\end{table*}

As shown in Table~\ref{tab:sam3_postprocess}, SAM3-based post-processing yields an average score increase of 2.88 and an average IoU increase of 0.049, while the average win and loss rates remain relatively close. However, the effect varies substantially across models. The improvement is strongly correlated with the original bbox-based performance: Spearman $\rho(\Delta\mathrm{Score}, \mathrm{Score}_{\mathrm{BBox}})=0.9000$ and $\rho(\Delta\mathrm{IoU}, \mathrm{IoU}_{\mathrm{BBox}})=0.8545$, with $p<0.001$ in both cases.

Stronger models generally benefit more from SAM3-based refinement, suggesting that their coarse predictions often already identify the correct target region and can therefore be further improved through finer boundary extraction. In contrast, weaker models frequently produce inaccurate or misaligned bounding boxes, limiting the benefit of subsequent segmentation. Importantly, although post-processing changes the absolute scores and enlarges the performance differences between some models, the overall model ranking remains largely unchanged.

These results suggest that the main evaluation protocol of EPIC-Bench provides a stable reflection of the relative VLG capabilities of existing models while avoiding the additional capability introduced by an external segmentation model. At the same time, the mask-level annotations in EPIC-Bench enable more fine-grained evaluation for models that natively support mask outputs, which we encourage future models to adopt.




% \clearpage
\subsection{Path Score Definition}
\label{app:path_score}


In this section, we describe the detailed design of the \textbf{Path Score}, which is used to evaluate the quality of predicted navigation paths. The score consists of five components: \textbf{Start-End Score}, \textbf{Traversable Path Ratio Score}, \textbf{Away-From-Start-Area Score}, \textbf{Approaching-Goal-Area Score} and \textbf{Continuity Score}.

Given a sequence of points predicted by the model, we first apply a \textbf{Neighbor Filtering} step to remove redundant points. If the distance between two consecutive points is smaller than $\frac{1}{30}$ of the image diagonal length, the two points are merged. After filtering, each remaining point is assigned a weighted score based on the five components described below. 

\textbf{Start-End Score.}
The Start-End Score measures how well the predicted path aligns with the target start and end areas. Specifically, we compute the distance between the first predicted point and the start area, as well as the distance between the last predicted point and the goal area $Dis(S,D)$. The distances are normalized by the image diagonal length to ensure scale invariance.

\begin{equation}
\text{Start-End Score} = \max(0, 1 - k \cdot D_{\text{norm}}),
\end{equation}

\begin{equation}
D_{\text{norm}} = \frac{\text{Distance}}{\text{Image Diagonal Length}},
\end{equation}
where $k$ is a hyperparameter (default $k=3.0$).

\textbf{Traversable Path Ratio Score.}
The Traversable Path Ratio Score encourages the model to generate paths that lie within regions annotated as feasible and traversable by human annotators. Starting from the second point, each point is connected to its preceding point to form a line segment $l_i$. The score is determined by the proportion of the segment that lies inside the ground-truth feasible-path mask $M_{fp}$.

\begin{equation}
\text{Traversable Path Ratio Score}_i =
\frac{\text{Length}(l_i \cap M_{fp})}{\text{Length}(l_i)},
\end{equation}
where $l_i$ denotes the line segment connecting points $p_{i-1}$ and $p_i$, and $M_{fp}$ denotes the ground-truth feasible-path Mask.

\textbf{Away-From-Start-Area Score} and \textbf{Approaching-Goal-Area Score.}
The two scores jointly encourage the model to generate more reasonable navigation trajectories, especially in complex scenes where detours may be necessary. If the evaluation only considers whether the path approaches the destination, the model may favor trivial straight-line predictions. To address this issue, we additionally reward paths that progressively move away from the start area while approaching the goal area.

For each point $p_i$ ($i \geq 2$), we compare its relative distances to the start and goal areas with those of its preceding point $p_{i-1}$. The \textbf{Away-From-Start-Area Score} is assigned in a binary manner: a point receives a score of $1$ if it is farther from the start area than its predecessor, and $0$ otherwise. Similarly, the \textbf{Approaching-Goal-Area Score} is also binary: a point receives a score of $1$ if it is closer to the goal area than its predecessor, and $0$ otherwise. Let $A_i$ denote the Away-From-Start-Area score, and $B_i$ denote the Approaching-Goal-Area score.

% \begin{equation}
% \begin{aligned}
% \text{Away-From-Start-Area Score}_i
% &=
% \begin{cases}
% 1, & \text{if } d(p_i, S) > d(p_{i-1}, S), \\
% 0, & \text{otherwise}.
% \end{cases}
% \end{aligned}
% \end{equation}

% \begin{equation}
% \text{Approaching-Goal-Area Score}_i =
% \begin{cases}
% 1, & \text{if } d(p_i, G) < d(p_{i-1}, G) \\
% 0, & \text{otherwise},
% \end{cases}
% \end{equation}

\begin{equation}
A_i =
\begin{cases}
1, & d(p_i, S) > d(p_{i-1}, S), \\
0, & \text{otherwise}.
\end{cases}
\end{equation}

\begin{equation}
B_i =
\begin{cases}
1, & d(p_i, G) < d(p_{i-1}, G), \\
0, & \text{otherwise}.
\end{cases}
\end{equation}

where $d(p_i, S)$ denotes the shortest distance between point $p_i$ and start area $S$, and $d(p_i, G)$ denotes the shortest distance between point $p_i$ and goal area $G$.

\textbf{Continuity Score.}
The continuity Score evaluates whether consecutive points form a coherent and realistic navigation path. Extremely large jumps between consecutive points often indicate unreliable or unrealistic predictions. Therefore, we penalize points whose distance to the preceding point exceeds a predefined threshold.

For each point $p_i$ ($i \geq 2$), the Continuity Score is assigned in a binary manner. If the distance between two consecutive points exceeds a threshold proportional to the start–goal distance, the point is considered discontinuous and receives a score of $0$; otherwise, it receives a score of $1$.

\begin{equation}
\text{Continuity Score}_i =
\begin{cases}
1, & \text{if } d(p_i, p_{i-1}) \leq \frac{2}{3} D_{SG}; \\
0, & \text{otherwise},
\end{cases}
\end{equation}
where $d(p_i, p_{i-1})$ denotes the Euclidean distance between two consecutive points, and $D_{SG}$ represents the shortest distance between the start area and the destination goal area.

% Together with the nearest-neighbor filtering step, this term encourages models to generate smoother and more continuous feasible paths.

We require the model to output at least \textbf{three consecutive points} to represent a valid path. The final score for each point is computed as a weighted combination of the five components, with weights determined by the point type, as shown in Table~\ref{tab:path_score_weight}. The final score of a predicted path is defined as the \textbf{average score over all valid points} in the sequence.


\begin{table}[!t]
\centering
\small
\resizebox{\columnwidth}{!}{
\begin{tabular}{lccccc}
\toprule
\textbf{Point Type} &
\textbf{Start-End} &
\makecell{\textbf{Traversable} \\ \textbf{Path Ratio}} &
\makecell{\textbf{Away-from-} \\ \textbf{Start-Area}} &
\makecell{\textbf{Approaching} \\ \textbf{Goal-Area}} &
\textbf{Continuity} \\
\midrule
Start point (first) & 1.0 & 0   & 0   & 0   & 0   \\
End point (last)    & 0.3 & 0.4 & 0.1 & 0.1 & 0.1 \\
Intermediate point  & 0   & 0.4 & 0.2 & 0.2 & 0.2 \\
\bottomrule
\end{tabular}
}
\caption{Weight configuration of the Path Score components.}
\label{tab:path_score_weight}
\end{table}


























% \input{sections/appendix_tab}

\section{Full Evaluation Results}
\label{app:additional_results}

In this section, we report the evaluation results of \textcolor{red}{80} representative VLMs on EPIC-Bench, as shown in Table~\ref{tab:table-performance-full}. 
We organize the models into four main categories:

\textbf{Proprietary models}: Gemini-2.5-Flash-Lite~\cite{gemini25}, Gemini-2.5-Flash~\cite{gemini25}, Gemini-2.5-Pro~\cite{gemini25}, Gemini-3-Flash-Pre~\cite{gemini3}, Gemini-3-pro~\cite{gemini3}, Gemini-3.1-Pro~\cite{gemini3}, Claude-Sonnet-4.6~\cite{claude46}, Claude-Haiku-4.5~\cite{ClaudeHaiku45}, Claude-Opus-4~\cite{ClaudeOpus4andClaudeSonnet4}, qwen3.6-plus~\cite{qwen36plus}, Qwen3.5-plus~\cite{qwen35}, Qwen3.6-27B~\cite{qwen36-27b}, Qwen3.6-35B-A3B~\cite{qwen36-35b-a3b}, Doubao-Seed-1.8~\cite{Seed1_8}, Doubao-Seed-1.6-Vision~\cite{Seed1_6}, HunYuan-T1-Vision~\cite{HunyuanVision}, HunYuan-Vision-1.5~\cite{HunyuanVision}, HunYuan-Turbos-Vision~\cite{HunyuanVision}, o3~\cite{openai_o3_o4mini_2025}, o4-mini~\cite{openai_o3_o4mini_2025}, GPT-4o~\cite{gpt-4o}, GPT-5-mini~\cite{gpt5}, GPT-5.1~\cite{gpt51}, GPT-5.2~\cite{gpt52}, GPT-5.4~\cite{gpt54}, GPT-5.5~\cite{gpt55}.

\textbf{Open-source models}: Qwen3.6-35B-A3B~\cite{qwen36-35b-a3b}, Qwen3.6-27B~\cite{qwen36-27b}, Qwen3.5~\cite{qwen35}, Qwen3-VL~\cite{qwen3vl}, Qwen2.5-VL-72B~\cite{qwen25vl}, InternVL3.5~\cite{internvl35}, InternVL3-78B~\cite{internvl3}, InternVL3-38B~\cite{internvl3}, InternVL3-14B~\cite{internvl3}, InternVL3-8B~\cite{internvl3}, Gemma-3~\cite{gemma3}, MiMo-VL-7B~\cite{MiMo-VL}, GLM-4.6V~\cite{glm46}, Step3-VL-10B~\cite{step3vl}, LLaVA-NeXT-72B~\cite{llavanext}.

\textbf{Embodied foundation models}: RoboBrain2~\cite{RoboBrain2-32B}, MiMo-Embodied-7B~\cite{MiMo-Embodied}, RoboBrain2.5~\cite{RoboBrain2.5}, Pelican1.0-VL-72B~\cite{Pelican-VL}, RynnBrain~\cite{RynnBrain}, VeBrain~\cite{VeBrain}, Cosmos-Reason1-7B~\cite{Cosmos-Reason1-7B}.

\textbf{Pixel-level models}: 

\textcolor{red}{GLAMM,LISA,UFO}

Our evaluation covers a diverse range of model scales, from large models to lightweight variants, and includes both open-source and proprietary systems. We hope these results will provide a comprehensive reference for researchers when selecting VLMs for embodied perception tasks.

\input{sections/appendix_tab}

% \begingroup
% \setlength{\tabcolsep}{2pt}       % 更紧凑的列间距
% \setlength{\extrarowheight}{2pt}  % 增加行高，让表格更宽松
% \renewcommand{\arraystretch}{1} % 稍微压缩行高
% \scriptsize                       % 更小的字体
% \onecolumn
% \begin{longtable}{l@{}c@{\hspace{1em}} lll lll lll}
% \caption{The full evaluation results for all \textbf{76 VLM variants} on EPIC-Bench.
% \colorbox{green!10}{\textbf{Green bold}} indicates the overall best result across all models.
% \textbf{Bold} and \underline{underline} indicate the best and second-best results within each model category, respectively.
% $^{\dagger}$ denotes models evaluated with thinking mode enabled.
% }\\
% \toprule
% \multirow{2}{*}{\textbf{Model}}
%     & \multirow{2}{*}{\textbf{Average}}
%     & \multicolumn{3}{c}{\textbf{Target Local.}}
%     & \multicolumn{3}{c}{\textbf{Navigation}}
%     & \multicolumn{3}{c}{\textbf{Manipulation}} \\
% \cmidrule(r){3-5} \cmidrule(r){6-8} \cmidrule(r){9-11}
% &  & Bas. & Spa. & Emb. & Gro. & Fea. & Vis. & Aff. & Con. & Pla. \\
% \midrule
% \endfirsthead % 以下为后续页的表头
% \toprule
% \multirow{2}{*}{\textbf{Model}}
%     & \multirow{2}{*}{\textbf{Average}}
%     & \multicolumn{3}{c}{\textbf{Target Local.}}
%     & \multicolumn{3}{c}{\textbf{Navigation}}
%     & \multicolumn{3}{c}{\textbf{Manipulation}} \\
% \cmidrule(r){3-5} \cmidrule(r){6-8} \cmidrule(r){9-11}
% &  & Bas. & Spa. & Emb. & Gro. & Fea. & Vis. & Aff. & Con. & Pla. \\
% \midrule
% \endhead
% \bottomrule
% % \\
% \multicolumn{11}{r}{\footnotesize Continued on next page} \\ % 可选的页末提示
% \endfoot
% \bottomrule
% \endlastfoot

% % 表格数据部分（原样复制，注意省略号需替换为实际行）
% \rowcolor{blue!8}[0pt][0pt]
% \multicolumn{11}{@{}c@{}}{\textbf{Proprietary Models}} \\

% Gemini-2.5-Flash-Lite\cite{gemini25}                & 34.77 & 39.06 & 39.53 & 31.51 & 35.97 & 40.21 & 33.02 & 2.58 & 30.17 & 32.38 \\
% Gemini-2.5-Flash\cite{gemini25}                     & 36.33 & 38.46 & 39.16 & 34.05 & 27.28 & 51.98 & 40.79 & 2.88 & 37.15 & 36.28 \\
% Gemini-2.5-Pro$^{\dagger}$\cite{gemini25}           & 37.63 & 42.86 & 41.62 & 36.43 & 9.63  & 46.29 & 42.70 & 8.72 & 33.94 & 42.78 \\
% Gemini-3-Flash-Pre\cite{gemini3}                    & 37.04 & 46.40 & 31.48 & 32.29 & \cellcolor{gray!10}\underline{48.98} & 22.89 & 47.25 & 11.91 & 42.29 & 48.09 \\
% Gemini-3-Flash-Pre$^{\dagger}$\cite{gemini3}        & 44.69 & 50.26 & 41.70 & 37.79 & \textbf{51.11} & 52.63 & \cellcolor{gray!10}\underline{49.92} & \cellcolor{gray!10}\underline{22.62} & 46.51 & \cellcolor{gray!10}\underline{50.89} \\
% Gemini-3-pro$^{\dagger}$\cite{gemini3}              & 54.81 & 56.81 & 54.50 & 53.90 & 48.82 & 70.82 & 60.08 & 30.40 & 51.78 & 53.42 \\
% Gemini-3.1-Pro$^{\dagger}$\cite{gemini3}            & \cellcolor{green!10}\textbf{54.72} & \textbf{55.38} & \cellcolor{green!10}\textbf{56.65} & \cellcolor{green!10}\textbf{53.04} & 47.22 & \cellcolor{green!10}\textbf{70.32} & \cellcolor{green!10}\textbf{59.06} & \cellcolor{green!10}\textbf{28.89} & \cellcolor{green!10}\textbf{53.7} & \cellcolor{green!10}\textbf{55.25} \\

% Claude-Sonnet-4.6$^{\dagger}$\cite{claude46}        & 43.24 & 45.43 & 45.49 & 36.47 & 40.16 & \cellcolor{gray!10}\underline{68.46} & 42.77 & 9.79 & 46.21 & 43.81 \\
% Claude-Sonnet-4.6\cite{claude46}                    & 31.34 & 43.84 & 32.16 & 21.94 & 5.25  & 39.56 & 40.9  & 0.54 & 35.90 & 35.77 \\
% Claude-Haiku-4.5$^{\dagger}$\cite{ClaudeHaiku45}    & 22.03 & 25.55 & 24.15 & 17.59 & 3.92  & 33.82 & 36.34 & 0.40 & 9.81  & 30.37 \\
% Claude-Haiku-4.5\cite{ClaudeHaiku45}                & 30.94 & 31.96 & 34.50 & 28.78 & 24.76 & 40.91 & 35.88 & 1.89 & 29.88 & 33.18 \\
% Claude-Opus-4\cite{ClaudeOpus4andClaudeSonnet4}     & 25.71 & 26.60 & 31.22 & 22.47 & 12.44 & 27.30 & 32.57 & 1.42 & 27.27 & 34.81 \\

% qwen3.6-plus$^{\dagger}$\cite{qwen36plus}           & 45.48 & 47.66 & 50.17 & 41.07 & 44.47 & 62.12 & 41.57 & 11.95 & 47.84 & 41.59 \\
% Qwen3.5-plus$^{\dagger}$\cite{qwen35}               & 47.10 & 55.09 & 51.90 & 41.82 & 50.85 & 57.89 & 45.21 & 13.82 & 22.34 & 42.46 \\
% Qwen3.6-27B$^{\dagger}$\cite{qwen36-27b}            & 36.31 & 46.33 & 45.05 & 36.31 & 11.61 & 35.10 & 28.07 & 10.76 & 21.53 & 26.78 \\
% Qwen3.6-35B-A3B$^{\dagger}$\cite{qwen36-35b-a3b}    & 35.07 & 48.17 & 43.99 & 36.61 & 14.41 & 33.97 & 21.30 &  2.84 & 17.05 & 15.90 \\

% Doubao-Seed-1.8$^{\dagger}$\cite{Seed1_8}           & 46.32 & \cellcolor{gray!10}\underline{55.29} & 49.68 &  \cellcolor{gray!10}\underline{46.10} & 46.02 & 53.43 & 45.9 & 10.94 & 14.36 & 40.79 \\
% Doubao-Seed-1.6-Vision$^{\dagger}$\cite{Seed1_6}    & \cellcolor{gray!10}\underline{46.80} & 54.64 &  \cellcolor{gray!10}\underline{49.92}& 42.27 & 41.64 & 58.74 & 42.66 & 9.52 & \cellcolor{gray!10}\underline{47.48} & 41.62 \\

% HunYuan-T1-Vision$^{\dagger}$\cite{HunyuanVision}   & 43.00 & 51.24 & 47.6  & 39.67 & 42.63 & 50.08 & 33.54 & 6.63 & 38.95 & 34.49 \\
% HunYuan-Vision-1.5\cite{HunyuanVision}              & 32.55 & 38.37 & 39.60 & 29.67 & 31.72 & 17.07 & 35.71 & 6.38 & 32.88 & 29.25 \\
% HunYuan-Turbos-Vision\cite{HunyuanVision}           & 24.61 & 24.72 & 33.33 & 25.58 & 4.49  & 17.88 & 36.14 & 0.67 & 22.02 & 26.69 \\

% o3$^{\dagger}$\cite{openai_o3_o4mini_2025}          & 36.05 & 39.37 & 40.96 & 32.86 & 36.24 & 30.64 & 40.73 & 5.49 & 32.43 & 43.64 \\
% o4-mini$^{\dagger}$\cite{openai_o3_o4mini_2025}     & 32.83 & 36.75 & 38.02 & 32.73 & 18.27 & 20.49 & 45.63 & 3.54 & 33.58 & 38.75 \\
% GPT-4o\cite{gpt-4o}                                 & 29.52 & 27.42 & 35.99 & 26.69 & 26.95 & 32.45 & 36.36 & 2.18 & 33.22 & 34.50 \\
% GPT-5-mini$^{\dagger}$\cite{gpt5}                   & 35.21 & 38.70 & 39.43 & 30.24 & 24.36 & 38.53 & 45.97 & 3.86 & 41.32 & 38.78 \\
% GPT-5.1\cite{gpt51}                                 & 34.81 & 35.31 & 39.66 & 32.05 & 36.62 & 38.62 & 44.69 & 4.34 & 26.44 & 38.63 \\
% GPT-5.2\cite{gpt52}                                 & 36.82 & 38.26 & 41.53 & 32.02 & 33.06 & 48.72 & 44.1  & 5.01 & 35.25 & 37.26 \\
% GPT-5.4\cite{gpt54}                                 & 38.95 & 43.78 & 43.90 & 33.84 & 32.24 & 43.12 & 44.35 & 8.67 & 39.55 & 37.30 \\
% GPT-5.5\cite{gpt55}                                 & 50.16 & 57.78 & 55.37 & 45.19 & 50.97 & 38.57 & 51.65 & 24.62& 49.67 & 48.70 \\

% % ... 其他行
% \midrule
% \rowcolor{blue!8}[0pt][0pt]
% \multicolumn{11}{@{}c@{}}{\textbf{Open-source Models}} \\
% Qwen3.6-35B-A3B\cite{qwen36-35b-a3b}           & 38.52 & 46.40 & 46.19 & 40.01 &  3.90 & 39.16 & 39.42 &  5.41 & 34.19 & 34.52 \\
% Qwen3.6-27B\cite{qwen36-27b}                   & 45.38 & 51.04 & 48.02 & 41.46 & 49.99 & 59.15 & 43.45 & 10.61 & 38.69 & 37.35 \\
% Qwen3.5-397B-A17B$^{\dagger}$\cite{qwen35}     &  \cellcolor{gray!10}\underline{47.47} & \cellcolor{gray!10}\underline{55.45} & 51.82 & 42.1  & 51.1  & 60.11 & 45.35 & 12.4  & 26.33 & \cellcolor{gray!10}\underline{42.51} \\
% Qwen3.5-397B-A17B\cite{qwen35}                 & 45.16 & 50.56 & 50.06 &  \cellcolor{gray!10}\underline{43.45} & \cellcolor{green!10}\textbf{51.94} & 50.61 & 41.46 & 8.31  & 34.51 & 37.08 \\
% Qwen3.5-122B-A10B$^{\dagger}$\cite{qwen35}     & 47.24 & 53.61 & 49.13 & 41.16 & \cellcolor{gray!10}\underline{51.42} & \textbf{63.47} & 45.19 & 12.31 & 46.04 & 39.77 \\
% Qwen3.5-122B-A10B\cite{qwen35}                 & 44.54 & 50.77 & 49.28 & 42.31 & 49.65 & 50.5  & 42.62 & 8.30  & 36.91 & 32.16 \\
% Qwen3.5-35B-A3B$^{\dagger}$\cite{qwen35}       & 45.58 & 53.51 & 49.18 & 39.03 & 43.09 & \cellcolor{gray!10}\underline{61.17} & 41.18 & 10.75 & 41.70 & 38.05 \\
% Qwen3.5-35B-A3B\cite{qwen35}                   & 41.32 & 46.76 & 45.82 & 38.19 & 48.00 & 45.47 & 37.01 & 10.01 & 36.94 & 32.36 \\
% Qwen3.5-27B$^{\dagger}$\cite{qwen35}           & 45.67 & 54.15 & 50.03 & 40.61 & 46.96 & 39.43 & \cellcolor{gray!10}\underline{46.77} & 13.15 &\textbf{49.56} & 39.84 \\
% Qwen3.5-27B\cite{qwen35}                       & 44.71 & 49.10 & 48.55 & 42.23 & 49.74 & 53.50 & 44.10 & 11.93 & 37.22 & 36.42 \\

% Qwen3.5-9B$^{\dagger}$\cite{qwen35}            & 38.86 & 44.60 & 43.38 & 33.87 & 31.26 & 49.06 & 40.22 & 6.07 & 37.64 & 34.92 \\
% Qwen3.5-9B\cite{qwen35}                        & 35.45 & 40.49 & 42.04 & 31.90 & 38.07 & 36.81 & 33.93 & 6.09 & 26.70 & 28.25 \\
% Qwen3.5-4B$^{\dagger}$\cite{qwen35}            & 35.59 & 40.83 & 42.34 & 31.24 & 24.09 & 45.21 & 35.33 & 5.65 & 24.79 & 33.90 \\
% Qwen3.5-4B\cite{qwen35}                        & 33.27 & 39.84 & 40.87 & 30.04 & 33.70 & 29.66 & 32.54 & 5.56 & 17.60 & 26.49 \\
% Qwen3.5-2B$^{\dagger}$\cite{qwen35}            & 28.49 & 33.36 & 35.06 & 27.34 & 14.58 & 25.31 & 25.13 & 3.39 & 30.10 & 27.01 \\
% Qwen3.5-2B\cite{qwen35}                        & 23.12 & 26.93 & 32.91 & 25.11 & 7.84  & 3.72 & 22.43 & 0.37 & 20.64 & 24.09 \\
% Qwen3.5-0.8B$^{\dagger}$\cite{qwen35}          & 19.27 & 21.89 & 28.72 & 19.82 & 0.77  & 9.26 & 13.02 & 0.95 & 18.88 & 22.36 \\
% Qwen3.5-0.8B\cite{qwen35}                      & 4.89  & 2.58  & 4.62  & 2.05  & 0.15  & 4.94 & 11.33 & 0.57 & 13.12 & 20.67 \\

% Qwen3-VL-235B-A22B$^{\dagger}$\cite{qwen3vl}      &\textbf{50.93} & \cellcolor{green!10}\textbf{58.00} &\textbf{55.67} & \textbf{48.12} & 48.18 & 51.19 & \textbf{49.01} & \cellcolor{gray!10}\underline{16.96} & \cellcolor{gray!10}\underline{48.04} & \textbf{46.49} \\
% Qwen3-VL-235B-A22B\cite{qwen3vl}                  & 42.64 & 50.12 & 45.86 & 39.34 & 50.96 & 43.14 & 38.69 & 12.00 & 34.55 & 35.71 \\
% Qwen3-VL-30B-A3B$^{\dagger}$\cite{qwen3vl}        & 44.02 & 52.69 & 49.37 & 40.87 & 42.34 & 41.65 & 36.20 & 10.62 & 38.78 & 40.72 \\
% Qwen3-VL-30B-A3B\cite{qwen3vl}                    & 30.60 & 28.31 & 34.27 & 25.04 & 49.37 & 37.09 & 30.12 & 9.33  & 31.49 & 34.07 \\
% Qwen3-VL-32B$^{\dagger}$\cite{qwen3vl}            & 37.21 & 39.94 & 41.26 & 36.05 & 31.03 & 42.04 & 39.07 & 4.84  & 35.23 & 40.03 \\
% Qwen3-VL-32B\cite{qwen3vl}                        & 35.21 & 37.49 & 39.82 & 33.21 & 44.38 & 36.74 & 36.57 & 4.72  & 30.62 & 30.49 \\
% Qwen3-VL-8B$^{\dagger}$\cite{qwen3vl}             & 35.55 & 39.92 & 41.66 & 33.89 & 21.68 & 38.51 & 34.94 & 5.22  & 32.05 & 37.01 \\
% Qwen3-VL-8B\cite{qwen3vl}                         & 34.07 & 39.48 & 42.54 & 32.10 & 38.11 & 26.67 & 31.84 & 5.19  & 14.63 & 30.91 \\
% Qwen3-VL-4B$^{\dagger}$\cite{qwen3vl}             & 32.83 & 38.42 & 41.30 & 31.97 & 18.29 & 29.47 & 30.95 & 3.91  & 22.15 & 31.83 \\
% Qwen3-VL-4B\cite{qwen3vl}                         & 33.24 & 39.95 & 41.55 & 33.78 & 40.39 & 18.45 & 30.17 & 3.20  & 11.30 & 27.00 \\
% Qwen3-VL-2B$^{\dagger}$\cite{qwen3vl}             & 31.82 & 39.67 & 40.75 & 30.08 & 15.36 & 24.02 & 22.59 & 6.07  & 28.24 & 28.97 \\
% Qwen3-VL-2B\cite{qwen3vl}                         & 32.53 & 38.43 & 42.87 & 29.08 & 37.55 & 9.78  & 28.55 & 7.99  & 29.56 & 29.59 \\

% Qwen2.5-VL-72B\cite{qwen25vl}                     & 42.51 & 47.54 & 49.79 & 40.92 & 49.45 & 42.49 & 37.08 & 14.77 & 21.21 & 35.90 \\

% InternVL3.5-241B-A28B\cite{internvl35}      & 40.75 & 44.65 & 50.59 & 37.61 & 35.94 & 35.47 & 33.73 & 16.85 & 36.41 & 37.60 \\
% InternVL3.5-38B\cite{internvl35}            & 42.54 & 48.69 & \cellcolor{gray!10}\underline{52.60} & 39.95 & 43.21 & 35.01 & 28.07 & \textbf{17.22} & 34.05 & 35.83 \\
% InternVL3.5-30B-A3B\cite{internvl35}        & 29.71 & 30.96 & 39.11 & 27.03 & 45.43 & 24.11 & 17.24 & 8.41  & 18.75 & 25.30 \\
% InternVL3.5-14B\cite{internvl35}            & 38.92 & 43.95 & 49.96 & 37.13 & 46.11 & 31.82 & 24.57 & 11.23 & 25.98 & 28.66 \\
% InternVL3.5-8B\cite{internvl35}             & 33.58 & 40.67 & 45.40 & 32.05 & 32.15 & 22.77 & 15.94 & 10.79 & 17.42 & 25.57 \\

% InternVL3-78B\cite{internvl3}           & 36.04 & 40.68 & 44.56 & 32.78 & 35.98 & 30.55 & 34.93 & 6.90  & 29.07 & 31.69 \\
% InternVL3-38B\cite{internvl3}           & 28.50 & 34.88 & 28.85 & 23.22 & 36.69 & 22.31 & 34.88 & 3.99  & 30.43 & 30.44 \\
% InternVL3-14B\cite{internvl3}           & 30.17 & 31.98 & 38.44 & 25.41 & 32.29 & 29.53 & 27.64 & 3.25  & 27.49 & 31.19 \\
% InternVL3-8B\cite{internvl3}            & 30.23 & 35.51 & 40.72 & 26.69 & 33.38 & 21.53 & 23.16 & 3.83  & 16.08 & 26.07 \\

% Gemma-3-27B-IT\cite{gemma3}             & 27.17 & 26.93 & 33.66 & 26.68 & 11.62 & 32.17 & 26.33 & 1.65  & 31.26 & 32.18 \\
% Gemma-3-12B-IT\cite{gemma3}             & 26.21 & 25.55 & 32.44 & 24.59 & 13.71 & 36.27 & 23.39 & 1.30  & 27.48 & 31.43 \\
% Gemma-3-4B-IT\cite{gemma3}              & 23.50 & 21.79 & 31.48 & 22.31 & 8.04  & 27.53 & 22.04 & 0.97  & 28.80 & 29.59 \\

% MiMo-VL-7B-SFT-2508\cite{MiMo-VL}       & 31.18 & 33.01 & 37.17 & 32.98 & 17.59 & 29.14 & 36.89 &  4.91 & 23.20 & 32.82 \\
% MiMo-VL-7B-RL-2508\cite{MiMo-VL}        & 34.65 & 36.65 & 42.31 & 34.92 & 18.31 & 36.90 & 37.45 &  6.51 & 30.37 & 32.86 \\

% GLM-4.6V$^{\dagger}$\cite{glm46}        & 42.84 & 50.19 & 47.71 & 37.89 & 42.46 & 51.11 & 36.55 & 8.32  & 34.14 & 39.79 \\
% Step3-VL-10B\cite{step3vl}              & 32.40 & 42.22 & 40.10 & 31.88 & 17.96 & 24.03 & 17.77 & 5.94  & 27.22 & 27.56 \\
% LLaVA-NeXT-72B\cite{llavanext}          & 20.40 & 26.54 & 29.42 & 19.93 & 14.18 & 6.34  & 6.19  & 2.99  & 12.75 & 18.63 \\
% \midrule

% \rowcolor{blue!8}[0pt][0pt]
% \multicolumn{11}{@{}c@{}}{\textbf{Embodied Foundation Models}} \\
% RoboBrain2-32B\cite{RoboBrain2-32B}      & \textbf{39.32} & \textbf{50.66} & \textbf{49.67} & \textbf{38.83} & \cellcolor{gray!10}\underline{38.85} & 0.61  & \cellcolor{gray!10}\underline{37.63} & 0.08 & \textbf{36.22} & \textbf{39.61} \\
% RoboBrain2-7B\cite{RoboBrain2-32B}       & 30.09 & 35.93 & 36.01 & 30.52 & 42.92 & 0.00  & 24.31 & 2.29 & \cellcolor{gray!10}\underline{31.58} & 32.95 \\

% MiMo-Embodied-7B\cite{MiMo-Embodied}     & 37.16 & 41.22 & 44.17 & 38.74 & 24.67 & 32.22 & 40.23 &  8.71 & 28.23 & 33.88 \\

% RoboBrain2.5-8B-NV\cite{RoboBrain2.5}    & 23.81 & 24.81 & 32.88 & 24.97 & 22.57 & 1.66  & 27.98 & 1.13 & 24.98 & 24.03 \\
% RoboBrain2.5-8B-MT\cite{RoboBrain2.5}    & 29.83 & 31.20 & 37.41 & 26.76 & 33.52 & \textbf{30.89} & 27.84 & 2.65 & 25.45 & 24.34 \\

% Pelican1.0-VL-72B\cite{Pelican-VL}       & \cellcolor{gray!10}\underline{35.29} & \cellcolor{gray!10}\underline{44.08} & \cellcolor{gray!10}\underline{42.11} & \cellcolor{gray!10}\underline{34.79} & \textbf{44.91} & 0.00  & \textbf{38.13} & \textbf{7.32} & 22.68 & \cellcolor{gray!10}\underline{37.96} \\

% RynnBrain-8B\cite{RynnBrain}            & 22.34 & 28.31 & 33.28 & 24.81 & 7.98  & 5.95  & 15.04 & 0.13 & 13.84 & 11.26 \\
% RynnBrain-CoP-8B\cite{RynnBrain}        & 16.83 & 12.48 & 21.78 & 16.08 & 21.51 & \cellcolor{gray!10}\underline{22.51} & 13.58 & 0.28 & 19.62 & 18.09 \\
% RynnBrain-Plan-8B\cite{RynnBrain}       & 23.59 & 23.53 & 32.53 & 26.08 & 2.12  & 19.57 & 21.41 & 0.11 & 18.79 & 31.02 \\
% RynnBrain-2B\cite{RynnBrain}            & 12.05 & 12.84 & 16.49 & 17.07 & 0.00  & 7.10  & 13.35 & 0.01 & 8.73  & 12.45 \\

% VeBrain\cite{VeBrain}                        & 29.27 & 33.63 & 35.98 & 27.69 & 29.56 & 20.04 & 27.58 &  2.85 & 19.25 & 32.30 \\
% Cosmos-Reason1-7B\cite{Cosmos-Reason1-7B}    & 23.25 & 29.74 & 26.64 & 19.67 & 24.68 & 3.03  & 25.44 & \cellcolor{gray!10}\underline{5.37} & 22.12 & 32.75 \\
% % \bottomrule
% \label{tab:table-performance-full}
% \end{longtable}
% % \endgroup

% \twocolumn


\clearpage
 
% \section*{Acknowledgements}
% xxxxxxx

% ---- Bibliography ----
%
% BibTeX users should specify bibliography style 'splncs04'.
% References will then be sorted and formatted in the correct style.
%
% \bibliographystyle{splncs04}
% \bibliography{main}
